# Supplementary material for: Can Large Language Models Adequately Perform Symbolic Reasoning Over Time Series?
Source: arXiv:2508.03963 source file (2026-04-24)
Supplement: Supplementary file 1 [file appendix_old.tex]

\begin{appendices}
\section{Coupled Differential Equations}
\label{appendix: coupled_DEs}


\begin{table}[htb]
    \centering
    \tiny
    \begin{tabular}{c|p{3cm}|l|p{2cm}|p{2cm}}
    \toprule
        ID & System description & Equation & Parameters & Initial values\\
        \midrule
1 & RC-circuit (charging capacitor) & $\frac{c_{0} - \frac{x_{0}}{c_{1}}}{c_{2}}$ & 0.7, 1.2, 2.31 & [10.0], [3.54]\\\hline
2 & Population growth (naive) & $c_{0} x_{0}$ & 0.23 & [4.78], [0.87]\\\hline
3 & Population growth with carrying capacity & $c_{0} x_{0} \cdot \left(1 - \frac{x_{0}}{c_{1}}\right)$ & 0.79, 74.3 & [7.3], [21.0]\\\hline
4 & RC-circuit with non-linear resistor (charging capacitor) & $-0.5 + \frac{1}{e^{c_{0} - \frac{x_{0}}{c_{1}}} + 1}$ & 0.5, 0.96 & [0.8], [0.02]\\\hline
5 & Velocity of a falling object with air resistance & $c_{0} - c_{1} x_{0}^{2}$ & 9.81, 0.0021175 & [0.5], [73.0]\\\hline
6 & Autocatalysis with one fixed abundant chemical & $c_{0} x_{0} - c_{1} x_{0}^{2}$ & 2.1, 0.5 & [0.13], [2.24]\\\hline
7 & Gompertz law for tumor growth & $c_{0} x_{0} \log{\left(c_{1} x_{0} \right)}$ & 0.032, 2.29 & [1.73], [9.5]\\\hline
8 & Logistic equation with Allee effect & $c_{0} x_{0} \left(-1 + \frac{x_{0}}{c_{2}}\right) \left(1 - \frac{x_{0}}{c_{1}}\right)$ & 0.14, 130.0, 4.4 & [6.123], [2.1]\\\hline
9 & Language death model for two languages & $c_{0} \cdot \left(1 - x_{0}\right) - c_{1} x_{0}$ & 0.32, 0.28 & [0.14], [0.55]\\\hline
10 & Refined language death model for two languages & $c_{0} x_{0}^{c_{1}} \cdot \left(1 - x_{0}\right) - x_{0} \cdot \left(1 - c_{0}\right) \left(1 - x_{0}\right)^{c_{1}}$ & 0.2, 1.2 & [0.83], [0.34]\\\hline
11 & Naive critical slowing down (statistical mechanics) & $- x_{0}^{3}$ &  & [3.4], [1.6]\\\hline
12 & Photons in a laser (simple) & $c_{0} x_{0} - c_{1} x_{0}^{2}$ & 1.8, 0.1107 & [11.0], [1.3]\\\hline
13 & Overdamped bead on a rotating hoop & $c_{0} \left(c_{1} \cos{\left(x_{0} \right)} - 1\right) \sin{\left(x_{0} \right)}$ & 0.0981, 9.7 & [3.1], [2.4]\\\hline
14 & Budworm outbreak model with predation & $c_{0} x_{0} \cdot \left(1 - \frac{x_{0}}{c_{1}}\right) - \frac{c_{3} x_{0}^{2}}{c_{2}^{2} + x_{0}^{2}}$ & 0.78, 81.0, 21.2, 0.9 & [2.76], [23.3]\\\hline
15 & Budworm outbreak with predation (dimensionless) & $c_{0} x_{0} \cdot \left(1 - \frac{x_{0}}{c_{1}}\right) - \frac{x_{0}^{2}}{x_{0}^{2} + 1}$ & 0.4, 95.0 & [44.3], [4.5]\\\hline
16 & Landau equation (typical time scale tau = 1) & $c_{0} x_{0} - c_{1} x_{0}^{3} - c_{2} x_{0}^{5}$ & 0.1, -0.04, 0.001 & [0.94], [1.65]\\\hline
17 & Logistic equation with harvesting/fishing & $c_{0} x_{0} \cdot \left(1 - \frac{x_{0}}{c_{1}}\right) - c_{2}$ & 0.4, 100.0, 0.3 & [14.3], [34.2]\\\hline
18 & Improved logistic equation with harvesting/fishing & $c_{0} x_{0} \cdot \left(1 - \frac{x_{0}}{c_{1}}\right) - \frac{c_{2} x_{0}}{c_{3} + x_{0}}$ & 0.4, 100.0, 0.24, 50.0 & [21.1], [44.1]\\\hline
19 & Improved logistic equation with harvesting/fishing (dimensionless) & $- \frac{c_{0} x_{0}}{c_{1} + x_{0}} + x_{0} \cdot \left(1 - x_{0}\right)$ & 0.08, 0.8 & [0.13], [0.03]\\\hline
20 & Autocatalytic gene switching (dimensionless) & $c_{0} - c_{1} x_{0} + \frac{x_{0}^{2}}{x_{0}^{2} + 1}$ & 0.1, 0.55 & [0.002], [0.25]\\\hline
21 & Dimensionally reduced SIR infection model for dead people (dimensionless) & $c_{0} - c_{1} x_{0} - e^{- x_{0}}$ & 1.2, 0.2 & [0.0], [0.8]\\\hline
22 & Hysteretic activation of a protein expression (positive feedback, basal promoter expression) & $c_{0} + \frac{c_{1} x_{0}^{5}}{c_{2} + x_{0}^{5}} - c_{3} x_{0}$ & 1.4, 0.4, 123.0, 0.89 & [3.1], [6.3]\\\hline
23 & Overdamped pendulum with constant driving torque/fireflies/Josephson junction (dimensionless) & $c_{0} - \sin{\left(x_{0} \right)}$ & 0.21 & [-2.74], [1.65]\\

    \bottomrule
    \end{tabular}
    \caption{Scalar ODEs in ODEBench.}
    \label{tab:odebench-1d}
\end{table}
\begin{table}[htb]
    \centering
    \tiny
    \begin{tabular}{c|p{3cm}|l|p{2cm}|p{2cm}}
    \toprule
        ID & System description & Equation & Parameters & Initial values\\
        \midrule
24 & Harmonic oscillator without damping & $\begin{cases}&x_{1}\\&- c_{0} x_{0}\end{cases}$ & 2.1 & [0.4, -0.03], [0.0, 0.2]\\\hline
25 & Harmonic oscillator with damping & $\begin{cases}&x_{1}\\&- c_{0} x_{0} - c_{1} x_{1}\end{cases}$ & 4.5, 0.43 & [0.12, 0.043], [0.0, -0.3]\\\hline
26 & Lotka-Volterra competition model (Strogatz version with sheeps and rabbits) & $\begin{cases}&x_{0} \left(c_{0} - c_{1} x_{1} - x_{0}\right)\\&x_{1} \left(c_{2} - x_{0} - x_{1}\right)\end{cases}$ & 3.0, 2.0, 2.0 & [5.0, 4.3], [2.3, 3.6]\\\hline
27 & Lotka-Volterra simple (as on Wikipedia) & $\begin{cases}&x_{0} \left(c_{0} - c_{1} x_{1}\right)\\&- x_{1} \left(c_{2} - c_{3} x_{0}\right)\end{cases}$ & 1.84, 1.45, 3.0, 1.62 & [8.3, 3.4], [0.4, 0.65]\\\hline
28 & Pendulum without friction & $\begin{cases}&x_{1}\\&- c_{0} \sin{\left(x_{0} \right)}\end{cases}$ & 0.9 & [-1.9, 0.0], [0.3, 0.8]\\\hline
29 & Dipole fixed point & $\begin{cases}&c_{0} x_{0} x_{1}\\&- x_{0}^{2} + x_{1}^{2}\end{cases}$ & 0.65 & [3.2, 1.4], [1.3, 0.2]\\\hline
30 & RNA molecules catalyzing each others replication & $\begin{cases}&x_{0} \left(- c_{0} x_{0} x_{1} + x_{1}\right)\\&x_{1} \left(- c_{0} x_{0} x_{1} + x_{0}\right)\end{cases}$ & 1.61 & [0.3, 0.04], [0.1, 0.21]\\\hline
31 & SIR infection model only for healthy and sick & $\begin{cases}&- c_{0} x_{0} x_{1}\\&c_{0} x_{0} x_{1} - c_{1} x_{1}\end{cases}$ & 0.4, 0.314 & [7.2, 0.98], [20.0, 12.4]\\\hline
32 & Damped double well oscillator & $\begin{cases}&x_{1}\\&- c_{0} x_{1} - x_{0}^{3} + x_{0}\end{cases}$ & 0.18 & [-1.8, -1.8], [5.8, 0.0]\\\hline
33 & Glider (dimensionless) & $\begin{cases}&- c_{0} x_{0}^{2} - \sin{\left(x_{1} \right)}\\&x_{0} - \frac{\cos{\left(x_{1} \right)}}{x_{0}}\end{cases}$ & 0.08 & [5.0, 0.7], [9.81, -0.8]\\\hline
34 & Frictionless bead on a rotating hoop (dimensionless) & $\begin{cases}&x_{1}\\&\left(- c_{0} + \cos{\left(x_{0} \right)}\right) \sin{\left(x_{0} \right)}\end{cases}$ & 0.93 & [2.1, 0.0], [-1.2, -0.2]\\\hline
35 & Rotational dynamics of an object in a shear flow & $\begin{cases}&\cos{\left(x_{0} \right)} \cot{\left(x_{1} \right)}\\&\left(c_{0} \sin^{2}{\left(x_{1} \right)} + \cos^{2}{\left(x_{1} \right)}\right) \sin{\left(x_{0} \right)}\end{cases}$ & 4.2 & [1.13, -0.3], [2.4, 1.7]\\\hline
36 & Pendulum with non-linear damping, no driving (dimensionless) & $\begin{cases}&x_{1}\\&- c_{0} x_{1} \cos{\left(x_{0} \right)} - x_{1} - \sin{\left(x_{0} \right)}\end{cases}$ & 0.07 & [0.45, 0.9], [1.34, -0.8]\\\hline
37 & Van der Pol oscillator (standard form) & $\begin{cases}&x_{1}\\&- c_{0} x_{1} \left(x_{0}^{2} - 1\right) - x_{0}\end{cases}$ & 0.43 & [2.2, 0.0], [0.1, 3.2]\\\hline
38 & Van der Pol oscillator (simplified form from Strogatz) & $\begin{cases}&c_{0} \left(- \frac{x_{0}^{3}}{3} + x_{0} + x_{1}\right)\\&- \frac{x_{0}}{c_{0}}\end{cases}$ & 3.37 & [0.7, 0.0], [-1.1, -0.7]\\\hline
39 & Glycolytic oscillator, e.g., ADP and F6P in yeast (dimensionless) & $\begin{cases}&c_{0} x_{1} + x_{0}^{2} x_{1} - x_{0}\\&- c_{0} x_{0} + c_{1} - x_{0}^{2} x_{1}\end{cases}$ & 2.4, 0.07 & [0.4, 0.31], [0.2, -0.7]\\\hline
40 & Duffing equation (weakly non-linear oscillation) & $\begin{cases}&x_{1}\\&c_{0} x_{1} \cdot \left(1 - x_{0}^{2}\right) - x_{0}\end{cases}$ & 0.886 & [0.63, -0.03], [0.2, 0.2]\\\hline
41 & Cell cycle model by Tyson for interaction between protein cdc2 and cyclin (dimensionless) & $\begin{cases}&c_{0} \left(c_{1} + x_{0}^{2}\right) \left(- x_{0} + x_{1}\right) - x_{0}\\&c_{2} - x_{0}\end{cases}$ & 15.3, 0.001, 0.3 & [0.8, 0.3], [0.02, 1.2]\\\hline
42 & Reduced model for chlorine dioxide-iodine-malonic acid rection (dimensionless) & $\begin{cases}&c_{0} - \frac{c_{1} x_{0} x_{1}}{x_{0}^{2} + 1} - x_{0}\\&c_{2} x_{0} \left(- \frac{x_{1}}{x_{0}^{2} + 1} + 1\right)\end{cases}$ & 8.9, 4.0, 1.4 & [0.2, 0.35], [3.0, 7.8]\\\hline
43 & Driven pendulum with linear damping / Josephson junction (dimensionless) & $\begin{cases}&x_{1}\\&c_{0} - c_{1} x_{1} - \sin{\left(x_{0} \right)}\end{cases}$ & 1.67, 0.64 & [1.47, -0.2], [-1.9, 0.03]\\\hline
44 & Driven pendulum with quadratic damping (dimensionless) & $\begin{cases}&x_{1}\\&c_{0} - c_{1} x_{1} \left|{x_{1}}\right| - \sin{\left(x_{0} \right)}\end{cases}$ & 1.67, 0.64 & [1.47, -0.2], [-1.9, 0.03]\\\hline
45 & Isothermal autocatalytic reaction model by Gray and Scott 1985 (dimensionless) & $\begin{cases}&c_{0} \cdot \left(1 - x_{0}\right) - x_{0} x_{1}^{2}\\&- c_{1} x_{1} + x_{0} x_{1}^{2}\end{cases}$ & 0.5, 0.02 & [1.4, 0.2], [0.32, 0.64]\\\hline
46 & Interacting bar magnets & $\begin{cases}&c_{0} \sin{\left(x_{0} - x_{1} \right)} - \sin{\left(x_{0} \right)}\\&- c_{0} \sin{\left(x_{0} - x_{1} \right)} - \sin{\left(x_{1} \right)}\end{cases}$ & 0.33 & [0.54, -0.1], [0.43, 1.21]\\\hline
47 & Binocular rivalry model (no oscillations) & $\begin{cases}&- x_{0} + \frac{1}{e^{c_{0} x_{1} - c_{1}} + 1}\\&- x_{1} + \frac{1}{e^{c_{0} x_{0} - c_{1}} + 1}\end{cases}$ & 4.89, 1.4 & [0.65, 0.59], [3.2, 10.3]\\\hline
48 & Bacterial respiration model for nutrients and oxygen levels & $\begin{cases}&c_{0} - \frac{x_{0} x_{1}}{c_{1} x_{0}^{2} + 1} - x_{0}\\&c_{2} - \frac{x_{0} x_{1}}{c_{1} x_{0}^{2} + 1}\end{cases}$ & 18.3, 0.48, 11.23 & [0.1, 30.4], [13.2, 5.21]\\\hline
49 & Brusselator: hypothetical chemical oscillation model (dimensionless) & $\begin{cases}&c_{1} x_{0}^{2} x_{1} - x_{0} \left(c_{0} + 1\right) + 1\\&c_{0} x_{0} - c_{1} x_{0}^{2} x_{1}\end{cases}$ & 3.03, 3.1 & [0.7, -1.4], [2.1, 1.3]\\\hline
50 & Chemical oscillator model by Schnackenberg 1979 (dimensionless) & $\begin{cases}&c_{0} + x_{0}^{2} x_{1} - x_{0}\\&c_{1} - x_{0}^{2} x_{1}\end{cases}$ & 0.24, 1.43 & [0.14, 0.6], [1.5, 0.9]\\\hline
51 & Oscillator death model by Ermentrout and Kopell 1990 & $\begin{cases}&c_{0} + \sin{\left(x_{1} \right)} \cos{\left(x_{0} \right)}\\&c_{1} + \sin{\left(x_{1} \right)} \cos{\left(x_{0} \right)}\end{cases}$ & 1.432, 0.972 & [2.2, 0.67], [0.03, -0.12]\\
    \bottomrule
    \end{tabular}
    \caption{2 dimensional ODEs in ODEBench.}
    \label{tab:odebench-2d}
\end{table}
\begin{table}[htb]
    \centering
    \tiny
    \begin{tabular}{c|p{3cm}|l|p{2cm}|p{2cm}}
    \toprule
        ID & System description & Equation & Parameters & Initial values\\
        \midrule
52 & Maxwell-Bloch equations (laser dynamics) & $\begin{cases}&c_{0} \left(- x_{0} + x_{1}\right)\\&c_{1} \left(x_{0} x_{2} - x_{1}\right)\\&c_{2} \left(- c_{3} x_{0} x_{1} + c_{3} - x_{2} + 1\right)\end{cases}$ & 0.1, 0.21, 0.34, 3.1 & [1.3, 1.1, 0.89], [0.89, 1.3, 1.1]\\\hline
53 & Model for apoptosis (cell death) & $\begin{cases}&c_{0} - c_{4} x_{0} - \frac{c_{5} x_{0} x_{1}}{c_{9} + x_{0}}\\&c_{1} x_{2} \left(c_{8} + x_{1}\right) - \frac{c_{2} x_{1}}{c_{6} + x_{1}} - \frac{c_{3} x_{0} x_{1}}{c_{7} + x_{1}}\\&- c_{1} x_{2} \left(c_{8} + x_{1}\right) + \frac{c_{2} x_{1}}{c_{6} + x_{1}} + \frac{c_{3} x_{0} x_{1}}{c_{7} + x_{1}}\end{cases}$ & 0.1, 0.6, 0.2, 7.95, 0.05, 0.4, 0.1, 2.0, 0.1, 0.1 & [0.005, 0.26, 2.15], [0.248, 0.0973, 0.0027]\\\hline
54 & Lorenz equations in well-behaved periodic regime & $\begin{cases}&c_{0} \left(- x_{0} + x_{1}\right)\\&c_{1} x_{0} - x_{0} x_{2} - x_{1}\\&- c_{2} x_{2} + x_{0} x_{1}\end{cases}$ & 5.1, 12.0, 1.67 & [2.3, 8.1, 12.4], [10.0, 20.0, 30.0]\\\hline
55 & Lorenz equations in complex periodic regime & $\begin{cases}&c_{0} \left(- x_{0} + x_{1}\right)\\&c_{1} x_{0} - x_{0} x_{2} - x_{1}\\&- c_{2} x_{2} + x_{0} x_{1}\end{cases}$ & 10.0, 99.96, 8/3 & [2.3, 8.1, 12.4], [10.0, 20.0, 30.0]\\\hline
56 & Lorenz equations standard parameters (chaotic) & $\begin{cases}&c_{0} \left(- x_{0} + x_{1}\right)\\&c_{1} x_{0} - x_{0} x_{2} - x_{1}\\&- c_{2} x_{2} + x_{0} x_{1}\end{cases}$ & 10.0, 28.0, 8/3 & [2.3, 8.1, 12.4], [10.0, 20.0, 30.0]\\\hline
57 & Rössler attractor (stable fixed point) & $\begin{cases}&c_{3} \left(- x_{1} - x_{2}\right)\\&c_{3} \left(c_{0} x_{1} + x_{0}\right)\\&c_{3} \left(c_{1} + x_{2} \left(- c_{2} + x_{0}\right)\right)\end{cases}$ & -0.2, 0.2, 5.7, 5.0 & [2.3, 1.1, 0.8], [-0.1, 4.1, -2.1]\\\hline
58 & Rössler attractor (periodic) & $\begin{cases}&c_{3} \left(- x_{1} - x_{2}\right)\\&c_{3} \left(c_{0} x_{1} + x_{0}\right)\\&c_{3} \left(c_{1} + x_{2} \left(- c_{2} + x_{0}\right)\right)\end{cases}$ & 0.1, 0.2, 5.7, 5.0 & [2.3, 1.1, 0.8], [-0.1, 4.1, -2.1]\\\hline
59 & Rössler attractor (chaotic) & $\begin{cases}&c_{3} \left(- x_{1} - x_{2}\right)\\&c_{3} \left(c_{0} x_{1} + x_{0}\right)\\&c_{3} \left(c_{1} + x_{2} \left(- c_{2} + x_{0}\right)\right)\end{cases}$ & 0.2, 0.2, 5.7, 5.0 & [2.3, 1.1, 0.8], [-0.1, 4.1, -2.1]\\\hline
60 & Aizawa attractor (chaotic) & $\begin{cases}&- c_{3} x_{1} + x_{0} \left(- c_{1} + x_{2}\right)\\&c_{3} x_{0} + x_{1} \left(- c_{1} + x_{2}\right)\\&c_{0} x_{2} + c_{2} + c_{5} x_{0}^{3} x_{2} - 1/3 x_{2}^{3} - \left(x_{0}^{2} + x_{1}^{2}\right) \left(c_{4} x_{2} + 1\right)\end{cases}$ & 0.95, 0.7, 0.65, 3.5, 0.25, 0.1 & [0.1, 0.05, 0.05], [-0.3, 0.2, 0.1]\\\hline
61 & Chen-Lee attractor; system for gyro motion with feedback control of rigid body (chaotic) & $\begin{cases}&c_{0} x_{0} - x_{1} x_{2}\\&c_{1} x_{1} + x_{0} x_{2}\\&c_{2} x_{2} + \frac{x_{0} x_{1}}{c_{3}}\end{cases}$ & 5.0, -10.0, -3.8, 3.0 & [15, -15, -15], [8, 14, -10]\\\hline
62 & Binocular rivalry model with adaptation (oscillations) & $\begin{cases}&- x_{0} + \frac{1}{e^{c_{0} x_{2} + c_{1} x_{1} - c_{2}} + 1}\\&c_{3} \left(x_{0} - x_{1}\right)\\&- x_{2} + \frac{1}{e^{c_{0} x_{0} + c_{1} x_{3} - c_{2}} + 1}\\&c_{3} \left(x_{2} - x_{3}\right)\end{cases}$ & 0.89, 0.4, 1.4, 1.0 & [2.25, -0.5, -1.13, 0.4], [0.342, -0.431, -0.86, 0.041]\\\hline
63 & SEIR infection model (proportions) & $\begin{cases}&- c_{1} x_{0} x_{2}\\&- c_{0} x_{1} + c_{1} x_{0} x_{2}\\&c_{0} x_{1} - c_{2} x_{2}\\&c_{2} x_{2}\end{cases}$ & 0.47, 0.28, 0.3 & [0.6, 0.3, 0.09, 0.01], [0.4, 0.3, 0.25, 0.05]\\
    \bottomrule
    \end{tabular}
    \caption{3 and 4 dimensional ODEs in ODEBench.}
    \label{tab:odebench-3d}
\end{table}


\begin{figure}[h]
    \centering
    \includegraphics[width=1\linewidth]{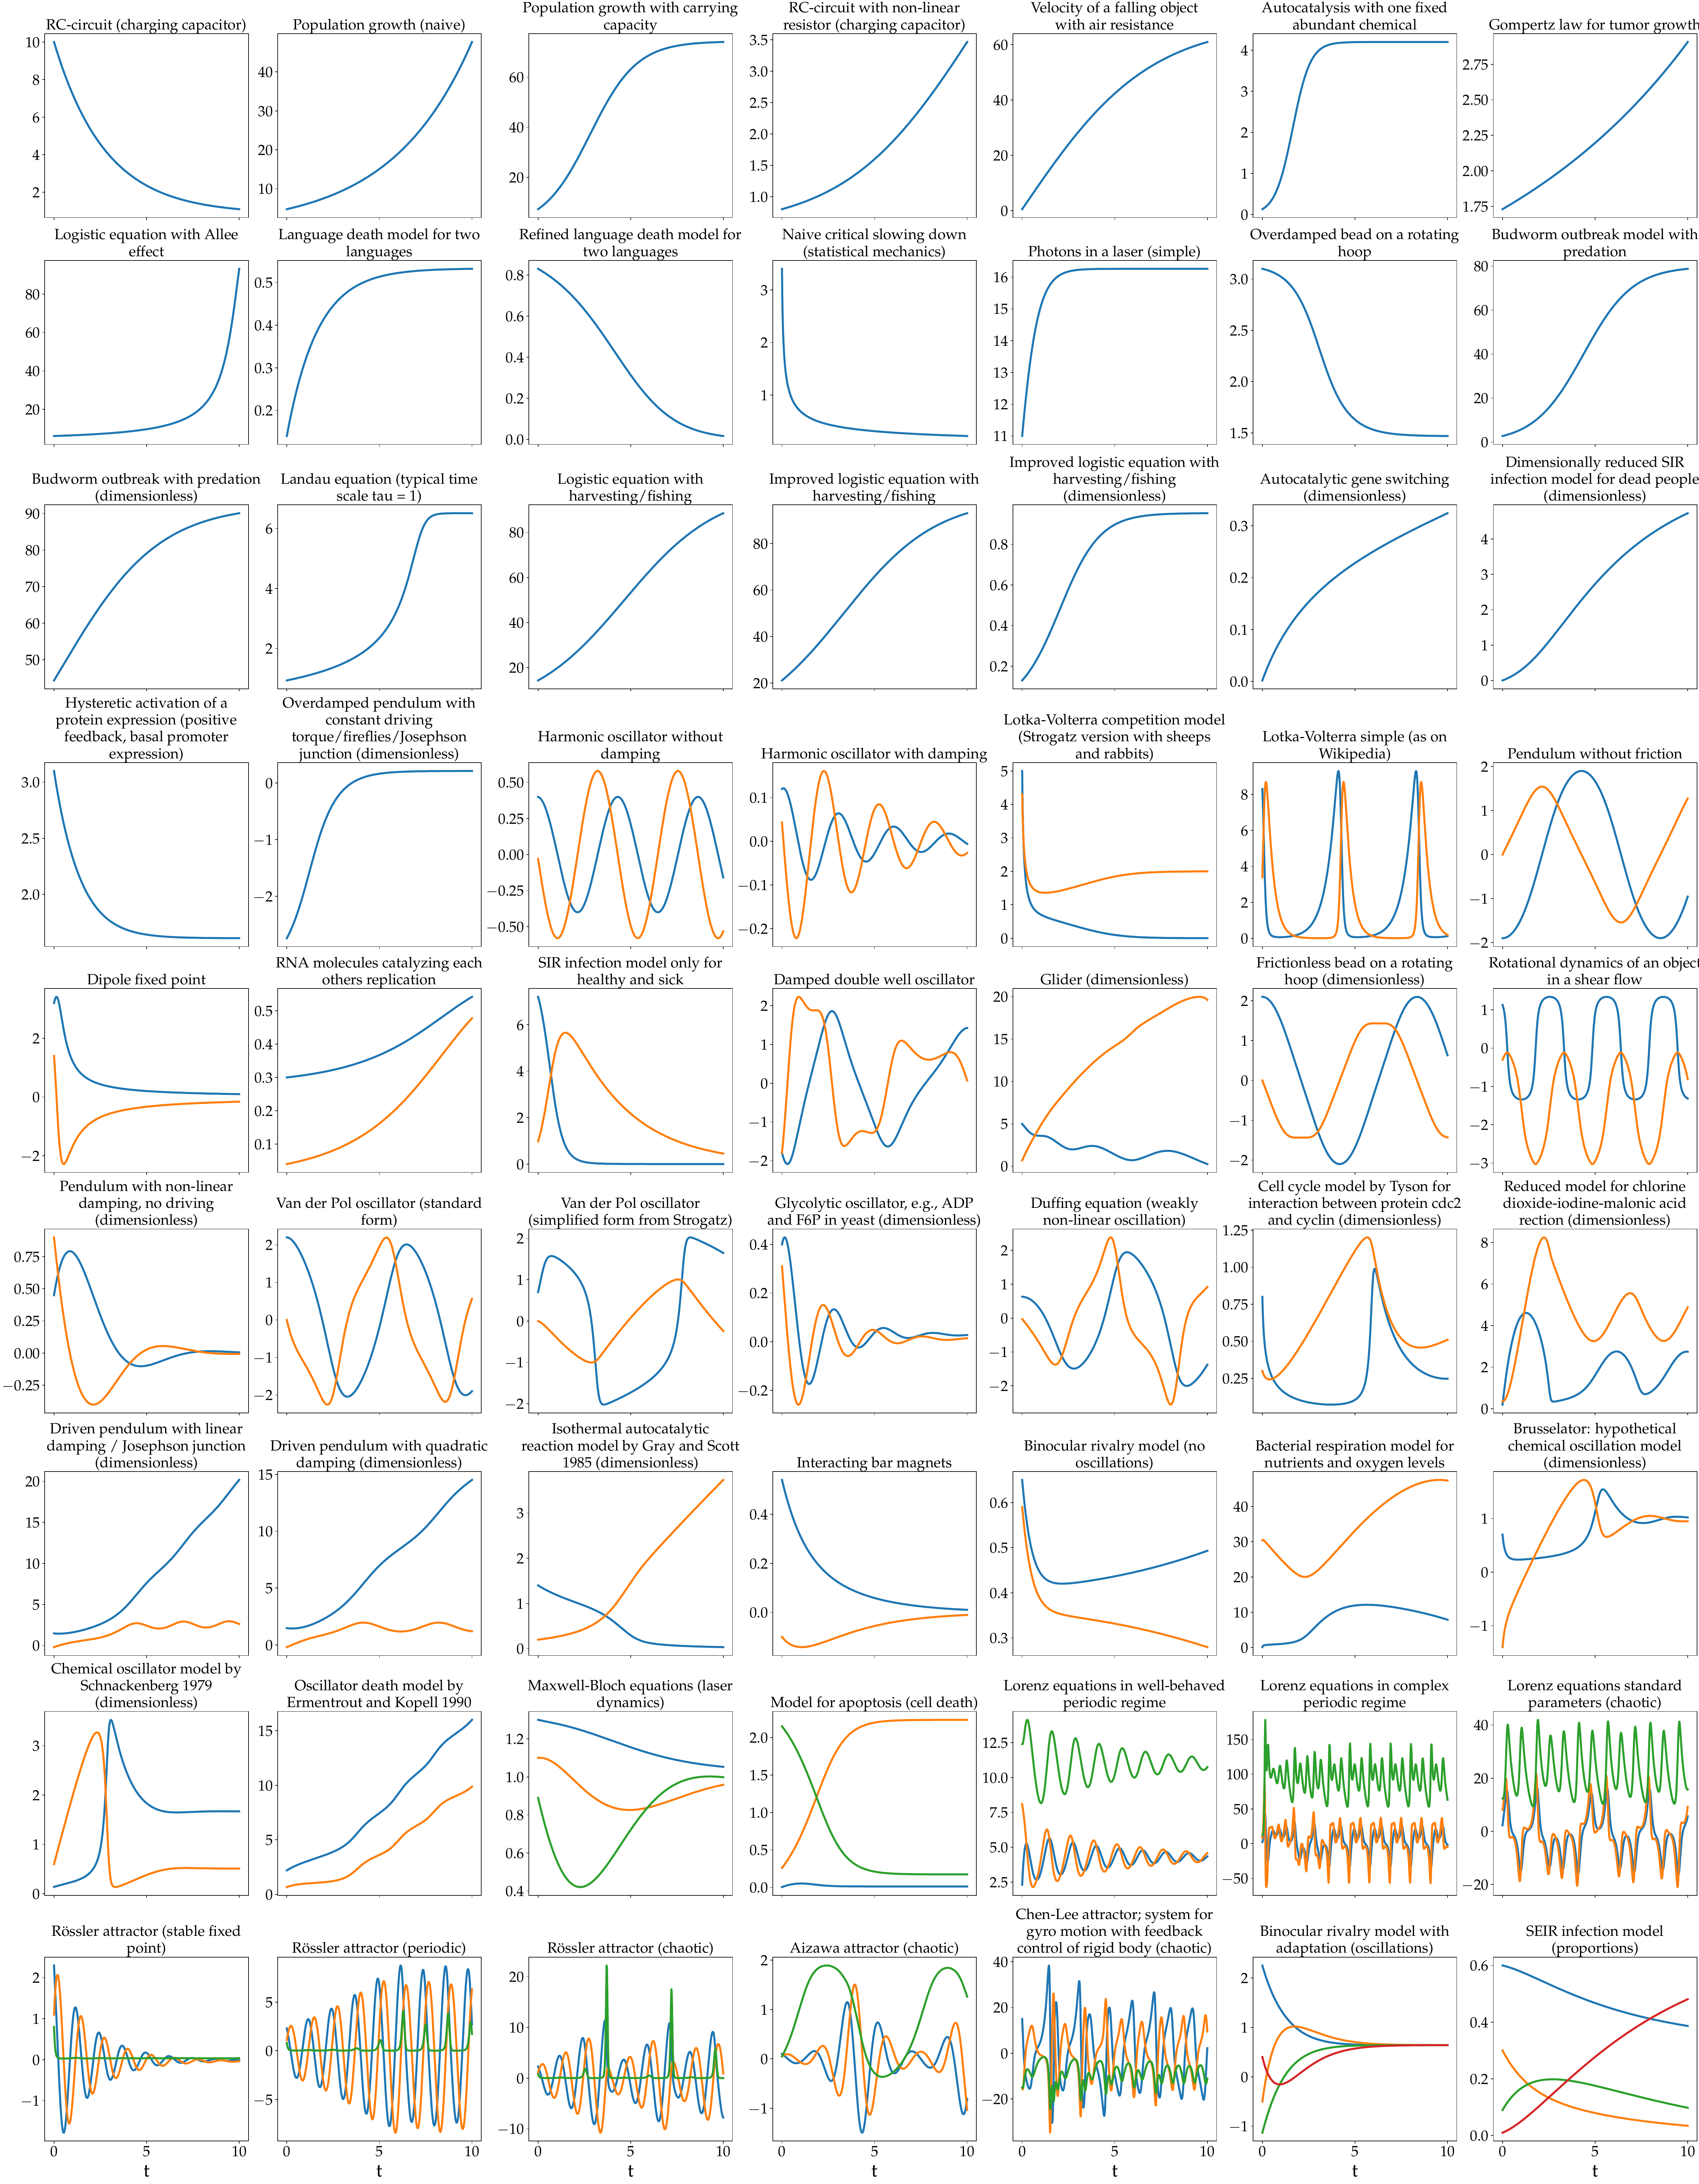}
    \caption{Visualization of ODEs from ODEBench}
\end{figure}



\clearpage
% \input{fig_table_tex/table_lsr_synth}





\clearpage
\section{Boolean Networks}
\label{appendix: BNs}

% \begin{longtable}[ht]      
% \footnotesize                     % or \scriptsize if you need a bit more room
% \centering
% \renewcommand{\arraystretch}{1.1}  % tighter vertical padding

% % Scale to textheight (the longer A4 edge) so nothing spills
% \resizebox{0.8\textheight}{!}{%
%   \begin{tabular}{
%     p{4cm}    % model_name  – wraps in 4 cm
%     >{\centering\arraybackslash}p{0.1cm}  % num_var
%     >{\centering\arraybackslash}p{0.4cm}    % num_inputs
%     >{\centering\arraybackslash}p{0.8cm}  % num_regulars
%     p{4.5cm} % variable_mapping – wraps
%     p{7.5cm} % regulations      – wraps
%   }

\footnotesize
%\begin{adjustbox}{max width=\linewidth,center}  % enable if you need it
\begin{longtable}{
  p{1cm} >{\centering\arraybackslash}p{0.9cm}
  >{\centering\arraybackslash}p{0.3cm} >{\centering\arraybackslash}p{1cm}
  p{3cm} p{7.5cm}}
\caption{Boolean‑network models used in this study}\label{tab:bn-summary}\\

\toprule
model\_name & var & inputs & regulars & variable\_mapping & regulations \\
\midrule
DROSOPHILA-WINGS-AP & 10 & 2 & 8 & x1: v\_Ap, x2: v\_Ap2, x3: v\_Dl, x4: v\_Dl2, x5: v\_Fng, x6: v\_Fng2, x7: v\_N, x8: v\_N2, x9: v\_Ser, x10: v\_Ser2 & x3 = ( NOT x1 AND x7 )
x4 = ( NOT x2 AND x8 )
x5 = x1
x6 = x2
x7 = ( ( NOT x5 AND x10 ) OR ( x5 AND x4 ) )
x8 = ( ( ( ( NOT x3 AND x9 ) AND NOT x6 ) OR ( ( x3 AND NOT x9 ) AND x6 ) ) OR ( x3 AND x9 ) )
x9 = x1
x10 = x2 \\
LAMBDA-PHAGE-LYSOGENY & 7 & 0 & 7 & x1: v\_CII, x2: v\_CI\_b1, x3: v\_CI\_b2, x4: v\_Cro\_b1, x5: v\_Cro\_b2, x6: v\_Cro\_b3, x7: v\_N & x1 = ( ( ( ( ( ( ( NOT x2 AND NOT x4 ) AND x7 ) OR ( ( ( NOT x2 AND x4 ) AND NOT x5 ) AND x7 ) ) OR ( ( ( ( NOT x2 AND x4 ) AND x5 ) AND NOT x6 ) AND x7 ) ) OR ( ( ( x2 AND NOT x3 ) AND NOT x4 ) AND x7 ) ) OR ( ( ( ( x2 AND NOT x3 ) AND x4 ) AND NOT x5 ) AND x7 ) ) OR ( ( ( ( ( x2 AND NOT x3 ) AND x4 ) AND x5 ) AND NOT x6 ) AND x7 ) )
x2 = ( ( ( ( ( NOT x2 AND NOT x4 ) OR ( ( NOT x2 AND x4 ) AND x1 ) ) OR ( ( x2 AND NOT x3 ) AND NOT x4 ) ) OR ( ( ( x2 AND NOT x3 ) AND x4 ) AND x1 ) ) OR ( x2 AND x3 ) )
x3 = ( ( x2 AND NOT x4 ) OR ( ( x2 AND x4 ) AND x1 ) )
x4 = ( ( NOT x2 OR ( x2 AND NOT x3 ) ) OR ( ( ( x2 AND x3 ) AND x4 ) AND x5 ) )
x5 = ( ( ( NOT x2 AND x4 ) OR ( ( x2 AND NOT x3 ) AND x4 ) ) OR ( ( ( ( x2 AND x3 ) AND x4 ) AND x5 ) AND x6 ) )
x6 = ( ( ( ( NOT x2 AND x4 ) AND x5 ) AND NOT x6 ) OR ( ( ( ( x2 AND NOT x3 ) AND x4 ) AND x5 ) AND NOT x6 ) )
x7 = ( ( NOT x2 AND NOT x4 ) OR ( ( NOT x2 AND x4 ) AND NOT x5 ) ) \\
PREDICTING-VARIABILITIES-IN-CARDIAC-GENE & 15 & 2 & 13 & x1: v\_Bmp2, x2: v\_Dkk1, x3: v\_Fgf8, x4: v\_Foxc1\_2, x5: v\_GATAs, x6: v\_Isl1, x7: v\_Mesp1\_, x8: v\_Nkx2\_5\_, x9: v\_Tbx1, x10: v\_Tbx5, x11: v\_canWnt, x12: v\_exogen\_BMP2\_I, x13: v\_exogen\_BMP2\_II, x14: v\_exogen\_CanWnt\_I, x15: v\_exogen\_CanWnt\_II & x1 = ( x13 AND NOT x11 )
x2 = ( ( x11 AND NOT x13 ) OR x7 )
x3 = ( ( x9 AND NOT x7 ) OR ( x4 AND NOT x7 ) )
x4 = ( x11 AND x15 )
x5 = ( ( x7 OR x8 ) OR x10 )
x6 = ( ( ( x7 OR x9 ) OR ( x11 AND x15 ) ) OR x3 )
x7 = ( x11 AND NOT x13 )
x8 = ( ( ( ( x10 OR ( x5 AND x1 ) ) OR ( x6 AND x5 ) ) OR x9 ) OR ( x7 AND x2 ) )
x9 = x4
x10 = ( ( ( x10 AND NOT ( ( x9 OR ( x2 AND ( NOT x10 AND NOT x7 ) ) ) OR x11 ) ) OR ( x7 AND NOT ( ( x9 OR ( x2 AND ( NOT x10 AND NOT x7 ) ) ) OR x11 ) ) ) OR ( x8 AND NOT ( ( x9 OR ( x2 AND ( NOT x10 AND NOT x7 ) ) ) OR x11 ) ) )
x11 = x15
x13 = x12
x15 = x14 \\
HCC1954-BREAST-CELL-LINE-SHORT-TERM & 16 & 5 & 11 & x1: v\_AKT, x2: v\_EGF, x3: v\_ERBB1, x4: v\_ERBB2, x5: v\_ERBB3, x6: v\_ERK1\_2, x7: v\_HRG, x8: v\_MEK1\_2, x9: v\_PDK1, x10: v\_PKCa, x11: v\_PLCg, x12: v\_erlotinib, x13: v\_mTOR, x14: v\_p70S6K, x15: v\_pertuzumab, x16: v\_trastuzumab & x1 = ( ( ( ( x14 OR x13 ) OR x5 ) OR x9 ) OR x1 )
x3 = ( ( ( x2 AND NOT ( x15 OR x12 ) ) OR ( x3 AND NOT ( x15 OR x12 ) ) ) OR ( x11 AND NOT ( x15 OR x12 ) ) )
x4 = ( ( ( x3 AND NOT ( ( x12 OR x16 ) OR x15 ) ) OR ( x4 AND NOT ( ( x12 OR x16 ) OR x15 ) ) ) OR ( x9 AND NOT ( ( x12 OR x16 ) OR x15 ) ) )
x5 = ( ( ( x6 AND NOT ( x12 OR x15 ) ) OR ( x5 AND NOT ( x12 OR x15 ) ) ) OR ( x7 AND NOT ( x12 OR x15 ) ) )
x6 = ( x8 OR x6 )
x8 = ( ( ( ( x3 OR x9 ) OR x8 ) OR x4 ) OR x5 )
x9 = ( ( ( x4 OR x9 ) OR x3 ) OR x5 )
x10 = ( ( x11 OR x10 ) OR x16 )
x11 = ( ( ( x3 OR x4 ) OR x11 ) OR x5 )
x13 = ( x1 OR x13 )
x14 = ( ( ( ( x13 OR x12 ) OR x14 ) OR x1 ) OR x6 ) \\
CHICKEN-SEX-DETERMINATION-REDUCED & 10 & 3 & 7 & x1: v\_AROMATASE, x2: v\_DMRT1\_b1, x3: v\_DMRT1\_b2, x4: v\_FOXL2, x5: v\_HEMGN, x6: v\_OESTROGEN, x7: v\_SOX9, x8: v\_W, x9: v\_Z1, x10: v\_Z2 & x1 = ( ( NOT x4 AND x6 ) OR x4 )
x2 = ( ( ( ( ( ( ( ( ( ( ( ( ( ( ( ( ( ( ( ( ( NOT x9 AND NOT x2 ) AND NOT x5 ) AND x7 ) AND NOT x4 ) OR ( ( ( NOT x9 AND NOT x2 ) AND x5 ) AND NOT x4 ) ) OR ( ( ( ( ( NOT x9 AND x2 ) AND NOT x3 ) AND NOT x5 ) AND x7 ) AND NOT x4 ) ) OR ( ( ( ( NOT x9 AND x2 ) AND NOT x3 ) AND x5 ) AND NOT x4 ) ) OR ( ( NOT x9 AND x2 ) AND x3 ) ) OR ( ( ( ( ( x9 AND NOT x10 ) AND NOT x2 ) AND NOT x5 ) AND x7 ) AND NOT x4 ) ) OR ( ( ( ( x9 AND NOT x10 ) AND NOT x2 ) AND x5 ) AND NOT x4 ) ) OR ( ( ( ( ( ( x9 AND NOT x10 ) AND x2 ) AND NOT x3 ) AND NOT x5 ) AND x7 ) AND NOT x4 ) ) OR ( ( ( ( ( x9 AND NOT x10 ) AND x2 ) AND NOT x3 ) AND x5 ) AND NOT x4 ) ) OR ( ( ( x9 AND NOT x10 ) AND x2 ) AND x3 ) ) OR ( ( ( ( x9 AND x10 ) AND NOT x8 ) AND NOT x2 ) AND NOT x4 ) ) OR ( ( ( ( ( x9 AND x10 ) AND NOT x8 ) AND x2 ) AND NOT x3 ) AND NOT x4 ) ) OR ( ( ( ( x9 AND x10 ) AND NOT x8 ) AND x2 ) AND x3 ) ) OR ( ( ( ( ( ( x9 AND x10 ) AND x8 ) AND NOT x2 ) AND NOT x5 ) AND x7 ) AND NOT x4 ) ) OR ( ( ( ( ( x9 AND x10 ) AND x8 ) AND NOT x2 ) AND x5 ) AND NOT x4 ) ) OR ( ( ( ( ( ( ( x9 AND x10 ) AND x8 ) AND x2 ) AND NOT x3 ) AND NOT x5 ) AND x7 ) AND NOT x4 ) ) OR ( ( ( ( ( ( x9 AND x10 ) AND x8 ) AND x2 ) AND NOT x3 ) AND x5 ) AND NOT x4 ) ) OR ( ( ( ( x9 AND x10 ) AND x8 ) AND x2 ) AND x3 ) )
x3 = ( ( ( ( x2 AND NOT x5 ) AND x7 ) AND NOT x4 ) OR ( ( x2 AND x5 ) AND NOT x4 ) )
x4 = ( ( ( ( NOT x2 AND NOT x7 ) OR ( ( NOT x2 AND x7 ) AND x6 ) ) OR ( ( x2 AND NOT x3 ) AND NOT x7 ) ) OR ( ( ( x2 AND NOT x3 ) AND x7 ) AND x6 ) )
x5 = ( x2 AND NOT x7 )
x6 = x1
x7 = ( ( ( ( NOT x2 AND x7 ) AND NOT x4 ) OR ( ( ( x2 AND NOT x3 ) AND x7 ) AND NOT x4 ) ) OR ( ( x2 AND x3 ) AND NOT x4 ) ) \\
MAMMALIAN-CELL-CYCLE-2006 & 10 & 1 & 9 & x1: v\_Cdc20, x2: v\_Cdh1, x3: v\_CycA, x4: v\_CycB, x5: v\_CycD, x6: v\_CycE, x7: v\_E2F, x8: v\_Rb, x9: v\_UbcH10, x10: v\_p27 & x1 = x4
x2 = ( ( x1 OR ( x10 AND NOT x4 ) ) OR NOT ( ( ( x10 OR x4 ) OR x3 ) OR x1 ) )
x3 = ( ( x3 AND NOT ( ( ( x2 AND x9 ) OR x1 ) OR x8 ) ) OR ( x7 AND NOT ( ( ( x2 AND x9 ) OR x1 ) OR x8 ) ) )
x4 = NOT ( x1 OR x2 )
x6 = ( x7 AND NOT x8 )
x7 = ( ( x10 AND NOT ( x4 OR x8 ) ) OR NOT ( ( ( x10 OR x8 ) OR x4 ) OR x3 ) )
x8 = ( ( x10 AND NOT ( x5 OR x4 ) ) OR NOT ( ( ( ( x6 OR x10 ) OR x4 ) OR x5 ) OR x3 ) )
x9 = ( ( ( ( ( x9 AND ( ( x2 AND ( ( x4 OR x1 ) OR x3 ) ) OR NOT x2 ) ) OR ( x3 AND NOT x2 ) ) OR ( x1 AND NOT x2 ) ) OR ( x4 AND NOT x2 ) ) OR NOT ( ( ( ( x9 OR x2 ) OR x4 ) OR x1 ) OR x3 ) )
x10 = ( ( x10 AND NOT ( ( x5 OR ( x3 AND x6 ) ) OR x4 ) ) OR NOT ( ( ( ( x6 OR x10 ) OR x4 ) OR x5 ) OR x3 ) ) \\
MAMMAL-SEX-DETERMINATION-1-CELL & 19 & 6 & 13 & x1: v\_AF, x2: v\_AS, x3: v\_Dmrt1, x4: v\_Fgf9\_b1, x5: v\_Fgf9\_b2, x6: v\_Foxl2, x7: v\_Gata4, x8: v\_IW, x9: v\_Sf1\_b1, x10: v\_Sf1\_b2, x11: v\_Sox9\_b1, x12: v\_Sox9\_b2, x13: v\_Sry, x14: v\_Wnt4\_b1, x15: v\_Wnt4\_b2, x16: v\_Wt1, x17: v\_Y, x18: v\_b\_cat\_b1, x19: v\_b\_cat\_b2 & x3 = ( ( ( ( ( NOT x7 AND x9 ) AND x11 ) AND x12 ) AND NOT x6 ) OR ( x7 AND NOT x6 ) )
x4 = ( ( ( NOT x11 AND x4 ) OR ( ( x11 AND NOT x12 ) AND x4 ) ) OR ( x11 AND x12 ) )
x5 = ( ( x11 AND x12 ) AND x4 )
x6 = ( x1 AND NOT x3 )
x9 = ( ( ( NOT x16 AND x9 ) AND x10 ) OR x16 )
x10 = ( ( ( x16 AND x9 ) AND x11 ) AND x12 )
x11 = ( ( ( ( ( ( ( NOT x9 AND x11 ) AND x12 ) OR ( ( ( x9 AND NOT x11 ) AND NOT x18 ) AND NOT x6 ) ) OR ( ( ( ( x9 AND NOT x11 ) AND x18 ) AND NOT x19 ) AND NOT x6 ) ) OR ( ( ( ( x9 AND x11 ) AND NOT x12 ) AND NOT x18 ) AND NOT x6 ) ) OR ( ( ( ( ( x9 AND x11 ) AND NOT x12 ) AND x18 ) AND NOT x19 ) AND NOT x6 ) ) OR ( ( x9 AND x11 ) AND x12 ) )
x12 = ( ( ( ( ( ( NOT x13 AND x9 ) AND x11 ) AND NOT x18 ) AND NOT x6 ) OR ( ( ( ( x13 AND x9 ) AND x11 ) AND NOT x18 ) AND NOT x6 ) ) OR ( ( ( ( ( x13 AND x9 ) AND x11 ) AND x18 ) AND NOT x19 ) AND NOT x6 ) )
x13 = ( ( ( ( ( ( x17 AND x16 ) AND x2 ) AND x7 ) AND x9 ) AND NOT x11 ) OR ( ( ( ( ( ( x17 AND x16 ) AND x2 ) AND x7 ) AND x9 ) AND x11 ) AND NOT x12 ) )
x14 = ( ( NOT x8 AND x14 ) OR ( ( x8 AND x14 ) AND x15 ) )
x15 = ( ( NOT x8 AND NOT x4 ) AND x14 )
x18 = ( ( ( ( ( ( ( NOT x11 AND NOT x14 ) AND x18 ) AND x19 ) OR ( NOT x11 AND x14 ) ) OR ( ( ( ( x11 AND NOT x12 ) AND NOT x14 ) AND x18 ) AND x19 ) ) OR ( ( x11 AND NOT x12 ) AND x14 ) ) OR ( ( ( x11 AND x12 ) AND x18 ) AND x19 ) )
x19 = ( ( ( ( NOT x11 AND x14 ) AND x15 ) AND x18 ) OR ( ( ( ( x11 AND NOT x12 ) AND x14 ) AND x15 ) AND x18 ) ) \\
ESCHERICHIA-COLI-TRYPTOPHAN & 16 & 3 & 13 & x1: v\_A, x2: v\_B, x3: v\_C, x4: v\_E, x5: v\_E\_m, x6: v\_L, x7: v\_M\_1, x8: v\_M\_2, x9: v\_P, x10: v\_R, x11: v\_T, x12: v\_W, x13: v\_W\_m, x14: v\_gamma, x15: v\_omega\_e, x16: v\_omega\_em & x1 = ( x8 AND NOT x14 )
x2 = x8
x3 = NOT x14
x4 = ( x7 AND NOT x6 )
x5 = ( x7 OR x4 )
x6 = ( x7 AND x11 )
x7 = NOT x10
x8 = ( x3 AND NOT x9 )
x9 = ( NOT x12 AND NOT x13 )
x10 = x12
x11 = x13
x12 = ( ( x7 AND ( NOT x6 AND NOT x1 ) ) OR ( x15 AND x2 ) )
x13 = ( x7 OR ( x12 OR ( x15 OR ( x16 AND x2 ) ) ) ) \\
SKBR3-BREAST-CELL-LINE-SHORT-TERM & 16 & 5 & 11 & x1: v\_AKT, x2: v\_EGF, x3: v\_ERBB1, x4: v\_ERBB2, x5: v\_ERBB3, x6: v\_ERK1\_2, x7: v\_HRG, x8: v\_MEK1\_2, x9: v\_PDK1, x10: v\_PKCa, x11: v\_PLCg, x12: v\_erlotinib, x13: v\_mTOR, x14: v\_p70S6K, x15: v\_pertuzumab, x16: v\_trastuzumab & x1 = ( ( ( x13 OR x9 ) OR x1 ) OR x5 )
x3 = ( ( ( x3 AND NOT ( x15 OR x12 ) ) OR ( x2 AND NOT ( x15 OR x12 ) ) ) OR ( x11 AND NOT ( x15 OR x12 ) ) )
x4 = ( x4 AND NOT ( ( x16 OR x15 ) OR x12 ) )
x5 = ( ( x5 AND NOT ( x12 OR x15 ) ) OR ( x7 AND NOT ( x12 OR x15 ) ) )
x6 = ( ( ( x9 OR x5 ) OR x8 ) OR x6 )
x8 = ( ( ( x4 OR x5 ) OR x3 ) OR x8 )
x9 = ( ( ( x4 OR x3 ) OR x9 ) OR x5 )
x10 = ( x11 OR x10 )
x11 = ( ( ( x4 OR x5 ) OR x3 ) OR x11 )
x13 = ( x13 OR x1 )
x14 = ( ( ( x14 OR x1 ) OR x13 ) OR x6 ) \\
MAPK-REDUCED-2 & 18 & 4 & 14 & x1: v\_AKT, x2: v\_Apoptosis, x3: v\_DNA\_damage, x4: v\_EGFR, x5: v\_EGFR\_stimulus, x6: v\_ERK, x7: v\_FGFR3, x8: v\_FGFR3\_stimulus, x9: v\_GRB2, x10: v\_Growth\_Arrest, x11: v\_PI3K, x12: v\_Proliferation, x13: v\_RAF, x14: v\_RAS, x15: v\_TGFBR\_stimulus, x16: v\_p21, x17: v\_p38, x18: v\_p53 & x1 = ( NOT x18 AND x11 )
x2 = ( ( ( ( ( ( ( ( NOT x15 AND NOT x3 ) AND NOT x6 ) AND NOT x17 ) AND x18 ) AND NOT x1 ) OR ( ( ( ( ( ( NOT x15 AND NOT x3 ) AND NOT x6 ) AND x17 ) AND x18 ) AND NOT x1 ) AND x14 ) ) OR ( ( ( ( NOT x15 AND x3 ) AND NOT x6 ) AND x18 ) AND NOT x1 ) ) OR ( ( ( x15 AND NOT x6 ) AND x18 ) AND NOT x1 ) )
x4 = ( ( ( ( ( NOT x5 AND x6 ) AND NOT x4 ) AND NOT x7 ) AND NOT x9 ) OR ( ( ( x5 AND NOT x4 ) AND NOT x7 ) AND NOT x9 ) )
x6 = ( ( ( ( ( ( ( ( ( ( NOT x15 AND NOT x3 ) AND NOT x6 ) AND NOT x17 ) AND NOT x18 ) AND x13 ) AND NOT x14 ) OR ( ( ( ( ( ( NOT x15 AND NOT x3 ) AND x6 ) AND NOT x17 ) AND NOT x18 ) AND NOT x13 ) AND x14 ) ) OR ( ( ( ( ( NOT x15 AND NOT x3 ) AND x6 ) AND NOT x17 ) AND NOT x18 ) AND x13 ) ) OR ( ( ( ( ( ( NOT x15 AND NOT x3 ) AND x6 ) AND NOT x17 ) AND x18 ) AND x13 ) AND NOT x14 ) ) OR ( ( ( ( ( ( NOT x15 AND x3 ) AND x6 ) AND NOT x17 ) AND NOT x18 ) AND x13 ) AND NOT x14 ) )
x7 = ( ( ( x8 AND NOT x4 ) AND NOT x7 ) AND NOT x9 )
x9 = ( ( ( ( ( ( ( NOT x15 AND NOT x6 ) AND NOT x4 ) AND x7 ) AND NOT x9 ) OR ( ( NOT x15 AND NOT x6 ) AND x4 ) ) OR ( ( NOT x15 AND x6 ) AND x4 ) ) OR x15 )
x10 = x16
x11 = ( ( NOT x9 AND x11 ) OR x9 )
x12 = ( ( ( ( ( x6 AND NOT x17 ) AND NOT x16 ) AND x1 ) AND x11 ) OR ( ( ( x6 AND x17 ) AND NOT x16 ) AND x11 ) )
x13 = ( ( ( ( ( ( NOT x6 AND NOT x4 ) AND NOT x7 ) AND NOT x1 ) AND x14 ) OR ( ( ( NOT x6 AND NOT x4 ) AND x7 ) AND NOT x1 ) ) OR ( ( NOT x6 AND x4 ) AND NOT x1 ) )
x14 = ( ( ( ( ( ( ( NOT x6 AND NOT x4 ) AND NOT x7 ) AND x9 ) OR ( ( NOT x6 AND NOT x4 ) AND x7 ) ) OR ( NOT x6 AND x4 ) ) OR ( ( x6 AND NOT x4 ) AND x7 ) ) OR ( x6 AND x4 ) )
x16 = ( x18 AND NOT x1 )
x17 = ( ( ( ( ( ( ( ( ( ( ( ( ( ( NOT x15 AND NOT x3 ) AND NOT x6 ) AND NOT x17 ) AND NOT x18 ) AND x14 ) OR ( ( ( ( NOT x15 AND NOT x3 ) AND NOT x6 ) AND NOT x17 ) AND x18 ) ) OR ( ( ( ( ( NOT x15 AND NOT x3 ) AND NOT x6 ) AND x17 ) AND x18 ) AND x14 ) ) OR ( ( ( ( NOT x15 AND NOT x3 ) AND x6 ) AND x18 ) AND x14 ) ) OR ( ( ( NOT x15 AND x3 ) AND NOT x6 ) AND NOT x17 ) ) OR ( ( ( ( ( NOT x15 AND x3 ) AND NOT x6 ) AND x17 ) AND NOT x18 ) AND x14 ) ) OR ( ( ( ( NOT x15 AND x3 ) AND NOT x6 ) AND x17 ) AND x18 ) ) OR ( ( ( ( NOT x15 AND x3 ) AND x6 ) AND NOT x18 ) AND x14 ) ) OR ( ( ( NOT x15 AND x3 ) AND x6 ) AND x18 ) ) OR x15 )
x18 = ( ( ( ( ( ( NOT x3 AND x17 ) OR ( ( ( ( x3 AND NOT x6 ) AND NOT x17 ) AND NOT x18 ) AND NOT x1 ) ) OR ( ( x3 AND NOT x6 ) AND x17 ) ) OR ( ( ( x3 AND x6 ) AND NOT x17 ) AND NOT x18 ) ) OR ( ( ( ( x3 AND x6 ) AND NOT x17 ) AND x18 ) AND x1 ) ) OR ( ( x3 AND x6 ) AND x17 ) ) \\
ASYMMETRIC-CELL-DIVISION-B & 9 & 0 & 9 & x1: v\_CckA, x2: v\_ChpT, x3: v\_ClpXP\_RcdA, x4: v\_CpdR, x5: v\_CtrAb, x6: v\_DivJ, x7: v\_DivK, x8: v\_DivL, x9: v\_PleC & x1 = x8
x2 = x1
x3 = NOT x4
x4 = x2
x5 = ( x2 AND NOT x3 )
x6 = ( x7 AND NOT x9 )
x7 = ( NOT x9 AND x6 )
x8 = NOT x7
x9 = NOT x7 \\
T-LGL-SURVIVAL-NETWORK-2011-REDUCED & 18 & 0 & 18 & x1: v\_Apoptosis\_, x2: v\_BID\_, x3: v\_CREB, x4: v\_CTLA4\_, x5: v\_Caspase, x6: v\_Ceramide\_, x7: v\_DISC\_, x8: v\_FLIP\_, x9: v\_Fas, x10: v\_GPCR\_, x11: v\_IAP\_, x12: v\_IFNG\_, x13: v\_MCL1, x14: v\_P2, x15: v\_S1P, x16: v\_SMAD\_, x17: v\_TCR, x18: v\_sFas & x1 = ( x5 OR x1 )
x2 = NOT ( x13 OR x1 )
x3 = ( x12 AND NOT x1 )
x4 = ( x17 AND NOT x1 )
x5 = ( ( x2 AND NOT ( x11 OR x1 ) ) OR ( x7 AND NOT x1 ) )
x6 = ( x9 AND NOT ( x1 OR x15 ) )
x7 = ( ( x9 AND NOT ( x8 OR x1 ) ) OR ( x6 AND NOT x1 ) )
x8 = NOT ( x1 OR x7 )
x9 = NOT ( x1 OR x18 )
x10 = ( x15 AND NOT x1 )
x11 = NOT ( x2 OR x1 )
x12 = NOT ( ( x14 OR x1 ) OR x16 )
x13 = NOT ( x1 OR x7 )
x14 = ( ( x12 AND NOT x1 ) OR ( x14 AND NOT x1 ) )
x15 = NOT ( x1 OR x6 )
x16 = ( x10 AND NOT x1 )
x17 = NOT ( x1 OR x4 )
x18 = ( x15 AND NOT x1 ) \\
YEAST-HYPHAL-TRANSITION & 19 & 3 & 16 & x1: v\_Brg1, x2: v\_Cyr1, x3: v\_EFG1\_T, x4: v\_ESCRT, x5: v\_Efg1, x6: v\_Efg1\_active, x7: v\_Farnesol, x8: v\_HAG\_T, x9: v\_HATs, x10: v\_HDACs, x11: v\_NRG1\_T, x12: v\_Nrg1\_HAGs, x13: v\_Rim8, x14: v\_Temperature, x15: v\_Ume6, x16: v\_cAMP\_PKA, x17: v\_hyphal\_initiation, x18: v\_hyphal\_maintenance, x19: v\_pH & x1 = NOT x12
x2 = ( NOT x7 AND x14 )
x3 = ( NOT x6 OR ( x6 AND x1 ) )
x4 = x13
x5 = x3
x6 = ( ( ( NOT x4 AND x16 ) AND x5 ) OR ( x4 AND x5 ) )
x8 = ( ( ( NOT x12 AND NOT x1 ) AND x15 ) OR ( NOT x12 AND x1 ) )
x9 = ( x6 AND NOT x10 )
x10 = x1
x11 = ( ( ( ( ( ( ( ( ( ( ( ( ( NOT x4 AND NOT x16 ) AND NOT x1 ) AND NOT x15 ) OR ( ( ( ( NOT x4 AND NOT x16 ) AND NOT x1 ) AND x15 ) AND x17 ) ) OR ( ( ( NOT x4 AND NOT x16 ) AND x1 ) AND x17 ) ) OR ( ( ( ( NOT x4 AND x16 ) AND NOT x6 ) AND NOT x1 ) AND NOT x15 ) ) OR ( ( ( ( ( NOT x4 AND x16 ) AND NOT x6 ) AND NOT x1 ) AND x15 ) AND x17 ) ) OR ( ( ( ( NOT x4 AND x16 ) AND NOT x6 ) AND x1 ) AND x17 ) ) OR ( ( ( NOT x4 AND x16 ) AND x6 ) AND x17 ) ) OR ( ( ( x4 AND NOT x6 ) AND NOT x1 ) AND NOT x15 ) ) OR ( ( ( ( x4 AND NOT x6 ) AND NOT x1 ) AND x15 ) AND x17 ) ) OR ( ( ( x4 AND NOT x6 ) AND x1 ) AND x17 ) ) OR ( ( x4 AND x6 ) AND x17 ) )
x12 = ( ( x11 AND NOT x10 ) OR ( ( x11 AND x10 ) AND x9 ) )
x13 = x19
x15 = ( NOT x12 AND x1 )
x16 = x2
x17 = ( ( ( ( ( NOT x12 AND NOT x1 ) AND x17 ) OR ( ( ( NOT x12 AND x1 ) AND NOT x9 ) AND x17 ) ) OR ( ( NOT x12 AND x1 ) AND x9 ) ) OR ( x12 AND x17 ) )
x18 = ( ( NOT x12 AND x15 ) AND x17 ) \\
DROSOPHILA-GAP-C & 7 & 2 & 5 & x1: v\_Gt, x2: v\_Hb\_b1, x3: v\_Hb\_b2, x4: v\_Hb\_b3, x5: v\_Kni, x6: v\_Kr\_b1, x7: v\_Kr\_b2 & x1 = NOT x6
x3 = ( ( x2 AND x3 ) AND x4 )
x5 = ( ( NOT x1 AND NOT x2 ) OR ( ( NOT x1 AND x2 ) AND NOT x3 ) )
x6 = ( ( ( ( ( ( ( ( ( ( ( ( ( ( NOT x1 AND NOT x2 ) AND x6 ) AND x7 ) OR ( ( NOT x1 AND x2 ) AND NOT x3 ) ) OR ( ( ( NOT x1 AND x2 ) AND x3 ) AND NOT x4 ) ) OR ( ( ( ( ( NOT x1 AND x2 ) AND x3 ) AND x4 ) AND x6 ) AND x7 ) ) OR ( ( ( x1 AND NOT x2 ) AND x6 ) AND x7 ) ) OR ( ( ( ( x1 AND x2 ) AND NOT x3 ) AND NOT x6 ) AND NOT x5 ) ) OR ( ( ( ( ( x1 AND x2 ) AND NOT x3 ) AND x6 ) AND NOT x7 ) AND NOT x5 ) ) OR ( ( ( ( x1 AND x2 ) AND NOT x3 ) AND x6 ) AND x7 ) ) OR ( ( ( ( ( x1 AND x2 ) AND x3 ) AND NOT x4 ) AND NOT x6 ) AND NOT x5 ) ) OR ( ( ( ( ( ( x1 AND x2 ) AND x3 ) AND NOT x4 ) AND x6 ) AND NOT x7 ) AND NOT x5 ) ) OR ( ( ( ( ( x1 AND x2 ) AND x3 ) AND NOT x4 ) AND x6 ) AND x7 ) ) OR ( ( ( ( ( x1 AND x2 ) AND x3 ) AND x4 ) AND x6 ) AND x7 ) )
x7 = ( ( ( ( ( NOT x1 AND x2 ) AND NOT x3 ) AND x6 ) AND NOT x5 ) OR ( ( ( ( ( NOT x1 AND x2 ) AND x3 ) AND NOT x4 ) AND x6 ) AND NOT x5 ) ) \\
CONTROL-OF-PROLIFERATION & 18 & 1 & 17 & x1: v\_AKT, x2: v\_E2F, x3: v\_EIF4F, x4: v\_FOXO3, x5: v\_GFs, x6: v\_MAPK, x7: v\_PI3K, x8: v\_PIP3, x9: v\_PRAS40, x10: v\_Proliferation\_b1, x11: v\_Proliferation\_b2, x12: v\_RAS, x13: v\_RTK, x14: v\_Rb, x15: v\_S6K, x16: v\_TSC, x17: v\_cycE, x18: v\_mTORC1 & x1 = x8
x2 = NOT x14
x3 = x18
x4 = ( NOT x6 OR ( x6 AND NOT x1 ) )
x6 = ( ( NOT x12 AND x8 ) OR x12 )
x7 = ( ( NOT x13 AND x12 ) OR x13 )
x8 = x7
x9 = NOT x1
x10 = ( ( ( ( ( ( NOT x2 AND NOT x3 ) AND x10 ) AND x11 ) OR ( ( ( ( NOT x2 AND x3 ) AND NOT x15 ) AND x10 ) AND x11 ) ) OR ( ( NOT x2 AND x3 ) AND x15 ) ) OR x2 )
x11 = ( ( ( x2 AND x3 ) AND x15 ) AND x10 )
x12 = x13
x13 = ( ( ( ( ( NOT x6 AND NOT x4 ) AND NOT x15 ) AND x5 ) OR ( ( NOT x6 AND x4 ) AND x5 ) ) OR ( ( x6 AND x4 ) AND x5 ) )
x14 = NOT x17
x15 = x18
x16 = ( NOT x6 AND NOT x1 )
x17 = ( ( ( ( NOT x4 AND NOT x1 ) AND x2 ) OR ( NOT x4 AND x1 ) ) OR ( x4 AND x2 ) )
x18 = ( NOT x16 AND NOT x9 ) \\
MAMMALIAN-CELL-CYCLE & 20 & 1 & 19 & x1: v\_Akt1, x2: v\_CDK2, x3: v\_CDK4, x4: v\_CDK6, x5: v\_CycD1, x6: v\_CycE1, x7: v\_EGF, x8: v\_ERa, x9: v\_ErbB1, x10: v\_ErbB1\_2, x11: v\_ErbB1\_3, x12: v\_ErbB2, x13: v\_ErbB2\_3, x14: v\_ErbB3, x15: v\_IGF1R, x16: v\_MEK1, x17: v\_cMYC, x18: v\_p21, x19: v\_p27, x20: v\_pRB & x1 = ( ( ( ( x13 OR x15 ) OR x10 ) OR x11 ) OR x9 )
x2 = ( x6 AND NOT ( x18 OR x19 ) )
x3 = ( x5 AND NOT ( x18 OR x19 ) )
x4 = x5
x5 = ( ( x1 AND ( x17 AND x8 ) ) OR ( x16 AND ( x8 AND x17 ) ) )
x6 = x17
x8 = ( x1 OR x16 )
x9 = x7
x10 = ( x9 AND x12 )
x11 = ( x9 AND x14 )
x12 = x7
x13 = ( x12 AND x14 )
x14 = x7
x15 = ( ( x8 AND NOT x13 ) OR ( x1 AND NOT x13 ) )
x16 = ( ( ( ( x13 OR x10 ) OR x15 ) OR x11 ) OR x9 )
x17 = ( ( x16 OR x1 ) OR x8 )
x18 = ( x8 AND NOT ( ( x3 OR x1 ) OR x17 ) )
x19 = ( x8 AND NOT ( ( ( x17 OR x3 ) OR x1 ) OR x2 ) )
x20 = ( ( x3 AND x4 ) OR ( x2 AND ( x4 AND x3 ) ) ) \\
CARDIAC-DEVELOPMENT & 15 & 2 & 13 & x1: v\_Bmp2, x2: v\_Dkk1, x3: v\_Fgf8, x4: v\_Foxc1\_2, x5: v\_GATAs, x6: v\_Isl1, x7: v\_Mesp1, x8: v\_Nkx2\_5, x9: v\_Tbx1, x10: v\_Tbx5, x11: v\_canWnt, x12: v\_exogen\_BMP2\_I, x13: v\_exogen\_BMP2\_II, x14: v\_exogen\_CanWnt\_I, x15: v\_exogen\_canWnt\_II & x1 = ( x13 AND NOT x11 )
x2 = ( x7 OR ( x11 AND NOT x13 ) )
x3 = ( ( x9 AND NOT x7 ) OR ( x4 AND NOT x7 ) )
x4 = ( x11 AND x15 )
x5 = ( ( x8 OR x10 ) OR x7 )
x6 = ( ( ( x7 OR x9 ) OR x3 ) OR ( x11 AND x15 ) )
x7 = ( x11 AND NOT x13 )
x8 = ( ( ( ( x10 OR x9 ) OR ( x7 AND x2 ) ) OR ( x1 AND x5 ) ) OR ( x6 AND x5 ) )
x9 = x4
x10 = ( ( ( x10 AND NOT ( ( x11 OR ( x2 AND ( NOT x10 AND NOT x7 ) ) ) OR x9 ) ) OR ( x8 AND NOT ( ( x11 OR ( x2 AND ( NOT x10 AND NOT x7 ) ) ) OR x9 ) ) ) OR ( x7 AND NOT ( ( x11 OR ( x2 AND ( NOT x10 AND NOT x7 ) ) ) OR x9 ) ) )
x11 = x15
x13 = x12
x15 = x14 \\
METABOLIC-INTERACTIONS-IN-GUT-MICROBIOME & 12 & 4 & 8 & x1: v\_Akkermansia\_, x2: v\_Barnesiella, x3: v\_Blautia, x4: v\_Clindamycin\_, x5: v\_Clostridium\_difficile, x6: v\_Coprobacillus, x7: v\_Enterobacteriaceae, x8: v\_Enterococcus, x9: v\_Lachnospiraceae, x10: v\_Lachnospiraceae\_other\_, x11: v\_Mollicutes, x12: v\_Other & x1 = x6
x2 = ( ( ( x10 AND NOT x4 ) OR ( x12 AND NOT x4 ) ) OR ( x9 AND NOT x4 ) )
x3 = ( ( ( ( x6 AND NOT x3 ) OR x8 ) OR ( x3 AND NOT x6 ) ) OR x3 )
x5 = ( x5 AND NOT x2 )
x8 = ( ( ( ( x7 OR x11 ) OR x3 ) OR x5 ) OR NOT ( ( ( ( x7 OR x5 ) OR x6 ) OR x3 ) OR x11 ) )
x9 = ( ( ( x9 AND NOT x4 ) OR ( x10 AND NOT x4 ) ) OR ( x12 AND NOT x4 ) )
x10 = ( ( ( x9 AND NOT x4 ) OR ( x12 AND NOT x4 ) ) OR ( x10 AND NOT x4 ) )
x12 = ( ( ( x12 AND NOT x4 ) OR ( x10 AND NOT x4 ) ) OR ( x9 AND NOT x4 ) ) \\
MORPHOGENETIC-CHECKPOINT & 12 & 1 & 11 & x1: v\_BUD, x2: v\_Clb2\_b1, x3: v\_Clb2\_b2, x4: v\_Hsl1, x5: v\_MASS\_b1, x6: v\_MASS\_b2, x7: v\_Mih1\_b1, x8: v\_Mih1\_b2, x9: v\_Mpk1, x10: v\_SBF, x11: v\_Swe1\_b1, x12: v\_Swe1\_b2 & x1 = x5
x2 = ( ( ( NOT x2 AND x5 ) OR ( ( x2 AND NOT x3 ) AND x5 ) ) OR ( x2 AND x3 ) )
x3 = ( ( ( ( ( ( ( NOT x11 AND x2 ) AND x5 ) OR ( ( ( ( ( x11 AND NOT x12 ) AND NOT x7 ) AND x2 ) AND x5 ) AND x6 ) ) OR ( ( ( ( ( ( x11 AND NOT x12 ) AND x7 ) AND NOT x8 ) AND x2 ) AND x5 ) AND x6 ) ) OR ( ( ( ( ( x11 AND NOT x12 ) AND x7 ) AND x8 ) AND x2 ) AND x5 ) ) OR ( ( ( ( ( ( x11 AND x12 ) AND x7 ) AND NOT x8 ) AND x2 ) AND x5 ) AND x6 ) ) OR ( ( ( ( ( x11 AND x12 ) AND x7 ) AND x8 ) AND x2 ) AND x5 ) )
x4 = x1
x6 = ( x5 AND x6 )
x7 = ( ( ( ( ( ( NOT x7 AND NOT x2 ) AND NOT x9 ) OR ( NOT x7 AND x2 ) ) OR ( ( ( x7 AND NOT x8 ) AND NOT x2 ) AND NOT x9 ) ) OR ( ( x7 AND NOT x8 ) AND x2 ) ) OR ( x7 AND x8 ) )
x8 = ( ( x7 AND x2 ) AND NOT x9 )
x9 = NOT x1
x10 = ( ( NOT x2 AND x5 ) OR ( ( x2 AND NOT x3 ) AND x5 ) )
x11 = ( ( ( ( ( ( ( ( ( NOT x10 AND x11 ) AND x12 ) OR ( ( x10 AND NOT x11 ) AND NOT x2 ) ) OR ( ( ( x10 AND NOT x11 ) AND x2 ) AND NOT x3 ) ) OR ( ( ( ( x10 AND NOT x11 ) AND x2 ) AND x3 ) AND NOT x4 ) ) OR ( ( ( x10 AND x11 ) AND NOT x12 ) AND NOT x2 ) ) OR ( ( ( ( x10 AND x11 ) AND NOT x12 ) AND x2 ) AND NOT x3 ) ) OR ( ( ( ( ( x10 AND x11 ) AND NOT x12 ) AND x2 ) AND x3 ) AND NOT x4 ) ) OR ( ( x10 AND x11 ) AND x12 ) )
x12 = ( ( ( ( x10 AND x11 ) AND NOT x2 ) AND NOT x4 ) OR ( ( ( ( x10 AND x11 ) AND x2 ) AND NOT x3 ) AND NOT x4 ) ) \\
CHICKEN-SEX-DETERMINATION & 15 & 3 & 12 & x1: v\_AMH, x2: v\_AROMA, x3: v\_B\_CATENIN, x4: v\_DMRT1\_b1, x5: v\_DMRT1\_b2, x6: v\_ESTRO, x7: v\_FGF9, x8: v\_FOXL2, x9: v\_HEMGN, x10: v\_SF1, x11: v\_SOX9, x12: v\_W, x13: v\_WNT4, x14: v\_Z1, x15: v\_Z2 & x1 = ( ( ( NOT x11 AND NOT x6 ) AND x10 ) OR ( x11 AND NOT x6 ) )
x2 = ( ( NOT x8 AND x10 ) OR x8 )
x3 = ( NOT x11 AND x13 )
x4 = ( ( ( ( ( ( ( ( ( ( ( ( ( ( ( ( ( ( ( ( ( NOT x14 AND NOT x4 ) AND NOT x9 ) AND x11 ) AND NOT x8 ) OR ( ( ( NOT x14 AND NOT x4 ) AND x9 ) AND NOT x8 ) ) OR ( ( ( ( ( NOT x14 AND x4 ) AND NOT x5 ) AND NOT x9 ) AND x11 ) AND NOT x8 ) ) OR ( ( ( ( NOT x14 AND x4 ) AND NOT x5 ) AND x9 ) AND NOT x8 ) ) OR ( ( NOT x14 AND x4 ) AND x5 ) ) OR ( ( ( ( ( x14 AND NOT x15 ) AND NOT x4 ) AND NOT x9 ) AND x11 ) AND NOT x8 ) ) OR ( ( ( ( x14 AND NOT x15 ) AND NOT x4 ) AND x9 ) AND NOT x8 ) ) OR ( ( ( ( ( ( x14 AND NOT x15 ) AND x4 ) AND NOT x5 ) AND NOT x9 ) AND x11 ) AND NOT x8 ) ) OR ( ( ( ( ( x14 AND NOT x15 ) AND x4 ) AND NOT x5 ) AND x9 ) AND NOT x8 ) ) OR ( ( ( x14 AND NOT x15 ) AND x4 ) AND x5 ) ) OR ( ( ( ( x14 AND x15 ) AND NOT x12 ) AND NOT x4 ) AND NOT x8 ) ) OR ( ( ( ( ( x14 AND x15 ) AND NOT x12 ) AND x4 ) AND NOT x5 ) AND NOT x8 ) ) OR ( ( ( ( x14 AND x15 ) AND NOT x12 ) AND x4 ) AND x5 ) ) OR ( ( ( ( ( ( x14 AND x15 ) AND x12 ) AND NOT x4 ) AND NOT x9 ) AND x11 ) AND NOT x8 ) ) OR ( ( ( ( ( x14 AND x15 ) AND x12 ) AND NOT x4 ) AND x9 ) AND NOT x8 ) ) OR ( ( ( ( ( ( ( x14 AND x15 ) AND x12 ) AND x4 ) AND NOT x5 ) AND NOT x9 ) AND x11 ) AND NOT x8 ) ) OR ( ( ( ( ( ( x14 AND x15 ) AND x12 ) AND x4 ) AND NOT x5 ) AND x9 ) AND NOT x8 ) ) OR ( ( ( ( x14 AND x15 ) AND x12 ) AND x4 ) AND x5 ) )
x5 = ( ( ( ( x4 AND NOT x9 ) AND x11 ) AND NOT x8 ) OR ( ( x4 AND x9 ) AND NOT x8 ) )
x6 = x2
x7 = x11
x8 = ( ( ( ( ( NOT x4 AND NOT x6 ) AND NOT x1 ) OR ( NOT x4 AND x6 ) ) OR ( ( ( x4 AND NOT x5 ) AND NOT x6 ) AND NOT x1 ) ) OR ( ( x4 AND NOT x5 ) AND x6 ) )
x9 = ( x4 AND NOT x11 )
x10 = x6
x11 = ( ( ( ( ( NOT x4 AND x11 ) AND NOT x8 ) AND NOT x3 ) OR ( ( ( ( x4 AND NOT x5 ) AND x11 ) AND NOT x8 ) AND NOT x3 ) ) OR ( ( x4 AND x5 ) AND NOT x8 ) )
x13 = NOT x7 \\
EGGSHELL-PATTERNING-PHENOMOENOLOGICAL & 8 & 4 & 4 & x1: v\_BMP, x2: v\_EGF\_b1, x3: v\_EGF\_b2, x4: v\_Floor, x5: v\_Operculum, x6: v\_Roof, x7: v\_Roof\_adj, x8: v\_anterior & x3 = ( x2 AND x3 )
x4 = ( ( ( ( ( x2 AND NOT x3 ) AND x1 ) AND x7 ) AND x8 ) OR ( ( ( x2 AND x3 ) AND x7 ) AND x8 ) )
x5 = ( ( ( ( ( x2 AND NOT x3 ) AND x1 ) AND NOT x7 ) AND x8 ) OR ( ( ( x2 AND x3 ) AND NOT x7 ) AND x8 ) )
x6 = ( ( ( x2 AND NOT x3 ) AND NOT x1 ) AND x8 ) \\
OXIDATIVE-STRESS-PATHWAY & 19 & 1 & 18 & x1: v\_ARE, x2: v\_ATM, x3: v\_Akt, x4: v\_Bach1, x5: v\_Bad, x6: v\_Bcl2, x7: v\_GSK3b, x8: v\_Keap1, x9: v\_Mdm2, x10: v\_Nrf2, x11: v\_PI3K, x12: v\_PIP2, x13: v\_PIP3, x14: v\_PKC, x15: v\_PTEN, x16: v\_ROS, x17: v\_Ras, x18: v\_Stress, x19: v\_p53 & x1 = ( x10 AND NOT ( ( x7 OR x4 ) OR x1 ) )
x2 = x16
x3 = x13
x4 = NOT x16
x5 = NOT x3
x6 = NOT ( x19 OR x5 )
x7 = NOT x3
x8 = ( ( x10 AND NOT x4 ) OR ( x8 AND NOT x4 ) )
x9 = ( ( x19 AND NOT x2 ) OR ( x3 AND NOT x2 ) )
x10 = ( ( x14 OR x3 ) OR NOT ( ( x3 OR x8 ) OR x14 ) )
x11 = x17
x12 = x11
x13 = ( x12 AND NOT x15 )
x14 = ( x16 AND ( NOT x1 OR NOT x1 ) )
x15 = NOT x16
x16 = ( x18 AND NOT x1 )
x17 = x16
x19 = ( x2 AND NOT x9 ) \\
CORTICAL-AREA-DEVELOPMENT & 5 & 0 & 5 & x1: v\_Coup\_fti, x2: v\_Emx2, x3: v\_Fgf8, x4: v\_Pax6, x5: v\_Sp8 & x1 = ( NOT ( x3 OR x5 ) OR NOT ( x5 OR x3 ) )
x2 = ( x1 AND NOT ( ( x3 OR x5 ) OR x4 ) )
x3 = ( ( x3 AND x5 ) AND NOT x2 )
x4 = ( x5 AND NOT ( x2 OR x1 ) )
x5 = ( x3 AND NOT x2 ) \\
BUDDING-YEAST-EXIT-MODULE & 16 & 5 & 11 & x1: v\_Bub2\_Bfa1, x2: v\_Cdc14, x3: v\_Cdc15, x4: v\_Cdc20, x5: v\_Cdc5Polo, x6: v\_Cdh1, x7: v\_Clb2\_b1, x8: v\_Clb2\_b2, x9: v\_Net1\_b1, x10: v\_Net1\_b2, x11: v\_PP2ACdc55\_b1, x12: v\_PP2ACdc55\_b2, x13: v\_SecurinPds1, x14: v\_SeparaseEsp1\_b1, x15: v\_SeparaseEsp1\_b2, x16: v\_Tem1 & x1 = ( ( ( NOT x11 AND NOT x5 ) OR ( ( x11 AND NOT x12 ) AND NOT x5 ) ) OR ( x11 AND x12 ) )
x3 = ( ( ( NOT x7 OR ( x7 AND NOT x8 ) ) OR ( ( ( x7 AND x8 ) AND NOT x9 ) AND x2 ) ) OR ( ( ( ( x7 AND x8 ) AND x9 ) AND NOT x10 ) AND x2 ) )
x4 = NOT x6
x5 = ( x7 AND NOT x6 )
x6 = ( ( ( ( ( ( NOT x7 AND NOT x9 ) AND NOT x2 ) AND x6 ) OR ( ( NOT x7 AND NOT x9 ) AND x2 ) ) OR ( ( NOT x7 AND x9 ) AND x6 ) ) OR ( ( ( x7 AND NOT x8 ) AND NOT x9 ) AND x2 ) )
x7 = ( ( ( NOT x7 AND NOT x6 ) OR ( ( x7 AND NOT x8 ) AND NOT x6 ) ) OR ( x7 AND x8 ) )
x8 = ( ( x7 AND NOT x4 ) AND NOT x6 )
x9 = ( ( ( ( ( ( ( ( ( ( ( ( ( ( ( ( ( ( ( ( ( ( ( ( ( ( ( ( ( NOT x7 AND NOT x11 ) AND NOT x1 ) AND NOT x16 ) AND NOT x9 ) AND x2 ) OR ( ( ( ( ( ( NOT x7 AND NOT x11 ) AND NOT x1 ) AND NOT x16 ) AND x9 ) AND NOT x10 ) AND x2 ) ) OR ( ( ( ( ( NOT x7 AND NOT x11 ) AND NOT x1 ) AND NOT x16 ) AND x9 ) AND x10 ) ) OR ( ( ( ( ( ( NOT x7 AND NOT x11 ) AND NOT x1 ) AND x16 ) AND NOT x3 ) AND NOT x9 ) AND x2 ) ) OR ( ( ( ( ( ( ( NOT x7 AND NOT x11 ) AND NOT x1 ) AND x16 ) AND NOT x3 ) AND x9 ) AND NOT x10 ) AND x2 ) ) OR ( ( ( ( ( ( NOT x7 AND NOT x11 ) AND NOT x1 ) AND x16 ) AND NOT x3 ) AND x9 ) AND x10 ) ) OR ( ( ( ( ( ( NOT x7 AND NOT x11 ) AND NOT x1 ) AND x16 ) AND x3 ) AND x9 ) AND x10 ) ) OR ( ( ( ( NOT x7 AND NOT x11 ) AND x1 ) AND NOT x9 ) AND x2 ) ) OR ( ( ( ( ( NOT x7 AND NOT x11 ) AND x1 ) AND x9 ) AND NOT x10 ) AND x2 ) ) OR ( ( ( ( NOT x7 AND NOT x11 ) AND x1 ) AND x9 ) AND x10 ) ) OR ( ( ( NOT x7 AND x11 ) AND NOT x1 ) AND NOT x16 ) ) OR ( ( ( ( NOT x7 AND x11 ) AND NOT x1 ) AND x16 ) AND NOT x3 ) ) OR ( ( ( ( ( ( NOT x7 AND x11 ) AND NOT x1 ) AND x16 ) AND x3 ) AND x9 ) AND x10 ) ) OR ( ( NOT x7 AND x11 ) AND x1 ) ) OR ( ( ( ( x7 AND NOT x8 ) AND NOT x11 ) AND x9 ) AND x10 ) ) OR ( ( ( ( x7 AND NOT x8 ) AND x11 ) AND NOT x1 ) AND NOT x16 ) ) OR ( ( ( ( ( x7 AND NOT x8 ) AND x11 ) AND NOT x1 ) AND x16 ) AND NOT x3 ) ) OR ( ( ( ( ( ( ( x7 AND NOT x8 ) AND x11 ) AND NOT x1 ) AND x16 ) AND x3 ) AND x9 ) AND x10 ) ) OR ( ( ( x7 AND NOT x8 ) AND x11 ) AND x1 ) ) OR ( ( ( ( x7 AND x8 ) AND NOT x11 ) AND x9 ) AND x10 ) ) OR ( ( ( ( ( x7 AND x8 ) AND x11 ) AND NOT x12 ) AND x9 ) AND x10 ) ) OR ( ( ( ( ( x7 AND x8 ) AND x11 ) AND x12 ) AND NOT x1 ) AND NOT x16 ) ) OR ( ( ( ( ( ( x7 AND x8 ) AND x11 ) AND x12 ) AND NOT x1 ) AND x16 ) AND NOT x3 ) ) OR ( ( ( ( ( ( ( ( x7 AND x8 ) AND x11 ) AND x12 ) AND NOT x1 ) AND x16 ) AND x3 ) AND x9 ) AND x10 ) ) OR ( ( ( ( x7 AND x8 ) AND x11 ) AND x12 ) AND x1 ) )
x10 = ( ( ( ( ( ( ( ( ( NOT x7 AND x11 ) AND NOT x1 ) AND NOT x16 ) AND x9 ) OR ( ( ( ( ( NOT x7 AND x11 ) AND NOT x1 ) AND x16 ) AND NOT x3 ) AND x9 ) ) OR ( ( ( NOT x7 AND x11 ) AND x1 ) AND x9 ) ) OR ( ( ( ( ( x7 AND x11 ) AND x12 ) AND NOT x1 ) AND NOT x16 ) AND x9 ) ) OR ( ( ( ( ( ( x7 AND x11 ) AND x12 ) AND NOT x1 ) AND x16 ) AND NOT x3 ) AND x9 ) ) OR ( ( ( ( x7 AND x11 ) AND x12 ) AND x1 ) AND x9 ) )
x12 = ( ( ( ( NOT x13 AND NOT x14 ) AND x11 ) OR ( ( x13 AND NOT x14 ) AND x11 ) ) OR ( ( ( x13 AND x14 ) AND NOT x15 ) AND x11 ) )
x13 = NOT x4 \\
ASYMMETRIC-CELL-DIVISION-A & 5 & 0 & 5 & x1: v\_CcrM, x2: v\_CtrA, x3: v\_DnaA, x4: v\_GcrA, x5: v\_SciP & x1 = ( ( x2 AND NOT x1 ) AND NOT x5 )
x2 = ( ( ( ( NOT x2 AND x4 ) AND NOT x1 ) AND NOT x5 ) OR ( ( x2 AND NOT x1 ) AND NOT x5 ) )
x3 = ( ( ( x2 AND NOT x4 ) AND NOT x3 ) AND x1 )
x4 = ( NOT x2 AND x3 )
x5 = ( x2 AND NOT x3 ) \\
BODY-SEGMENTATION-IN-DROSOPHILA-2013 & 17 & 3 & 14 & x1: v\_CIA, x2: v\_CIR, x3: v\_CI\_protein, x4: v\_EN\_protein, x5: v\_HH\_protein, x6: v\_PH, x7: v\_PTC\_protein, x8: v\_SLP, x9: v\_SMO, x10: v\_WG\_external, x11: v\_WG\_protein, x12: v\_ci, x13: v\_en, x14: v\_hh, x15: v\_hh\_external, x16: v\_ptc, x17: v\_wg & x1 = ( ( x15 AND x3 ) OR ( x3 AND NOT x7 ) )
x2 = ( ( x3 AND x7 ) AND NOT x15 )
x3 = x12
x4 = x13
x5 = x14
x6 = ( x7 AND x15 )
x7 = ( ( x7 AND NOT x15 ) OR x16 )
x9 = ( x15 OR NOT ( x15 OR x7 ) )
x11 = x17
x12 = NOT x4
x13 = ( x10 AND NOT x8 )
x14 = ( x4 AND NOT x2 )
x16 = ( x1 AND NOT ( x2 OR x4 ) )
x17 = ( ( ( x17 AND ( x8 OR x1 ) ) AND NOT x2 ) OR ( ( x1 AND x8 ) AND NOT x2 ) ) \\
DROSOPHILA-GAP-D & 7 & 2 & 5 & x1: v\_Gt, x2: v\_Hb\_b1, x3: v\_Hb\_b2, x4: v\_Hb\_b3, x5: v\_Kni, x6: v\_Kr\_b1, x7: v\_Kr\_b2 & x1 = ( NOT x2 AND NOT x6 )
x2 = ( x2 AND x3 )
x3 = ( ( x2 AND x3 ) AND x4 )
x5 = ( ( NOT x1 AND NOT x2 ) OR ( ( NOT x1 AND x2 ) AND NOT x3 ) )
x6 = ( x6 AND x7 ) \\
DROSOPHILA-DPP-PATHWAY & 18 & 8 & 10 & x1: v\_Brk, x2: v\_Dad, x3: v\_Dpp\_b1, x4: v\_Dpp\_b2, x5: v\_Gbb, x6: v\_MadMed\_b1, x7: v\_MadMed\_b2, x8: v\_Nej, x9: v\_Punt, x10: v\_Sax, x11: v\_Scw, x12: v\_Shn, x13: v\_Sog, x14: v\_Targets, x15: v\_Tkv\_b1, x16: v\_Tkv\_b2, x17: v\_Tld, x18: v\_Tsg & x1 = ( NOT x12 AND NOT x6 )
x2 = ( ( NOT x1 AND x6 ) AND x7 )
x4 = ( x3 AND x4 )
x6 = ( ( ( ( ( ( ( ( NOT x15 AND NOT x10 ) AND x6 ) AND x7 ) OR ( ( NOT x15 AND x10 ) AND NOT x2 ) ) OR ( ( ( ( NOT x15 AND x10 ) AND x2 ) AND x6 ) AND x7 ) ) OR ( ( x15 AND NOT x16 ) AND NOT x2 ) ) OR ( ( ( ( x15 AND NOT x16 ) AND x2 ) AND x6 ) AND x7 ) ) OR ( x15 AND x16 ) )
x7 = ( ( ( x15 AND x16 ) AND NOT x2 ) AND x6 )
x10 = ( ( ( ( ( ( NOT x11 AND NOT x5 ) AND NOT x13 ) AND x3 ) AND x9 ) OR ( ( ( NOT x11 AND x5 ) AND NOT x13 ) AND x9 ) ) OR ( ( x11 AND NOT x13 ) AND x9 ) )
x13 = NOT x17
x14 = ( ( NOT x1 AND x6 ) AND x8 )
x15 = ( ( ( ( ( ( ( ( ( ( ( ( ( ( ( ( ( ( ( ( NOT x11 AND NOT x5 ) AND NOT x13 ) AND NOT x3 ) AND x15 ) AND x16 ) OR ( ( ( ( ( ( NOT x11 AND NOT x5 ) AND NOT x13 ) AND x3 ) AND NOT x18 ) AND NOT x15 ) AND x9 ) ) OR ( ( ( ( ( ( ( NOT x11 AND NOT x5 ) AND NOT x13 ) AND x3 ) AND NOT x18 ) AND x15 ) AND NOT x16 ) AND x9 ) ) OR ( ( ( ( ( ( NOT x11 AND NOT x5 ) AND NOT x13 ) AND x3 ) AND NOT x18 ) AND x15 ) AND x16 ) ) OR ( ( ( ( ( ( NOT x11 AND NOT x5 ) AND NOT x13 ) AND x3 ) AND x18 ) AND x15 ) AND x16 ) ) OR ( ( ( ( NOT x11 AND NOT x5 ) AND x13 ) AND x15 ) AND x16 ) ) OR ( ( ( ( ( NOT x11 AND x5 ) AND NOT x13 ) AND NOT x18 ) AND NOT x15 ) AND x9 ) ) OR ( ( ( ( ( ( NOT x11 AND x5 ) AND NOT x13 ) AND NOT x18 ) AND x15 ) AND NOT x16 ) AND x9 ) ) OR ( ( ( ( ( NOT x11 AND x5 ) AND NOT x13 ) AND NOT x18 ) AND x15 ) AND x16 ) ) OR ( ( ( ( ( NOT x11 AND x5 ) AND NOT x13 ) AND x18 ) AND x15 ) AND x16 ) ) OR ( ( ( ( NOT x11 AND x5 ) AND x13 ) AND x15 ) AND x16 ) ) OR ( ( ( ( x11 AND NOT x13 ) AND NOT x18 ) AND NOT x15 ) AND x9 ) ) OR ( ( ( ( ( x11 AND NOT x13 ) AND NOT x18 ) AND x15 ) AND NOT x16 ) AND x9 ) ) OR ( ( ( ( x11 AND NOT x13 ) AND NOT x18 ) AND x15 ) AND x16 ) ) OR ( ( ( ( x11 AND NOT x13 ) AND x18 ) AND x15 ) AND x16 ) ) OR ( ( ( x11 AND x13 ) AND x15 ) AND x16 ) )
x16 = ( ( ( ( ( NOT x13 AND x3 ) AND x4 ) AND NOT x18 ) AND x15 ) AND x9 ) \\
DROSOPHILA-GAP-B & 7 & 3 & 4 & x1: v\_Gt, x2: v\_Hb\_b1, x3: v\_Hb\_b2, x4: v\_Hb\_b3, x5: v\_Kni, x6: v\_Kr\_b1, x7: v\_Kr\_b2 & x1 = NOT x6
x3 = x2
x6 = ( ( ( ( ( ( ( ( ( ( ( ( ( ( NOT x1 AND NOT x2 ) AND x6 ) AND x7 ) OR ( ( NOT x1 AND x2 ) AND NOT x3 ) ) OR ( ( ( NOT x1 AND x2 ) AND x3 ) AND NOT x4 ) ) OR ( ( ( ( ( NOT x1 AND x2 ) AND x3 ) AND x4 ) AND x6 ) AND x7 ) ) OR ( ( ( x1 AND NOT x2 ) AND x6 ) AND x7 ) ) OR ( ( ( ( x1 AND x2 ) AND NOT x3 ) AND NOT x6 ) AND NOT x5 ) ) OR ( ( ( ( ( x1 AND x2 ) AND NOT x3 ) AND x6 ) AND NOT x7 ) AND NOT x5 ) ) OR ( ( ( ( x1 AND x2 ) AND NOT x3 ) AND x6 ) AND x7 ) ) OR ( ( ( ( ( x1 AND x2 ) AND x3 ) AND NOT x4 ) AND NOT x6 ) AND NOT x5 ) ) OR ( ( ( ( ( ( x1 AND x2 ) AND x3 ) AND NOT x4 ) AND x6 ) AND NOT x7 ) AND NOT x5 ) ) OR ( ( ( ( ( x1 AND x2 ) AND x3 ) AND NOT x4 ) AND x6 ) AND x7 ) ) OR ( ( ( ( ( x1 AND x2 ) AND x3 ) AND x4 ) AND x6 ) AND x7 ) )
x7 = ( ( ( ( ( NOT x1 AND x2 ) AND NOT x3 ) AND x6 ) AND NOT x5 ) OR ( ( ( ( ( NOT x1 AND x2 ) AND x3 ) AND NOT x4 ) AND x6 ) AND NOT x5 ) ) \\
DROSOPHILA-CELL-CYCLE & 14 & 3 & 11 & x1: v\_Ago, x2: v\_CycA, x3: v\_CycB, x4: v\_CycD, x5: v\_CycE, x6: v\_Dap, x7: v\_E2F, x8: v\_Fzr, x9: v\_Fzy, x10: v\_Notch, x11: v\_Rb, x12: v\_Rux, x13: v\_Stg, x14: v\_Wee1 & x2 = ( ( ( NOT x11 AND x7 ) AND NOT x9 ) AND NOT x8 )
x3 = ( ( ( NOT x9 AND NOT x8 ) AND NOT x14 ) OR ( ( ( NOT x9 AND NOT x8 ) AND x14 ) AND x13 ) )
x5 = ( ( ( NOT x11 AND x7 ) AND NOT x6 ) OR ( ( ( NOT x11 AND x7 ) AND x6 ) AND NOT x1 ) )
x6 = ( ( NOT x5 AND NOT x10 ) OR x5 )
x7 = ( ( ( ( ( NOT x11 AND NOT x2 ) AND NOT x12 ) AND NOT x3 ) OR ( ( NOT x11 AND NOT x2 ) AND x12 ) ) OR ( ( NOT x11 AND x2 ) AND x12 ) )
x8 = ( ( ( ( ( ( ( ( NOT x5 AND NOT x2 ) AND NOT x12 ) AND NOT x3 ) OR ( ( NOT x5 AND NOT x2 ) AND x12 ) ) OR ( ( NOT x5 AND x2 ) AND x12 ) ) OR ( ( ( ( x5 AND NOT x2 ) AND NOT x12 ) AND NOT x3 ) AND x10 ) ) OR ( ( ( x5 AND NOT x2 ) AND x12 ) AND x10 ) ) OR ( ( ( x5 AND x2 ) AND x12 ) AND x10 ) )
x9 = ( NOT x12 AND x3 )
x11 = ( ( ( ( ( ( NOT x4 AND NOT x5 ) AND NOT x2 ) AND NOT x12 ) AND NOT x3 ) OR ( ( ( NOT x4 AND NOT x5 ) AND NOT x2 ) AND x12 ) ) OR ( ( ( NOT x4 AND NOT x5 ) AND x2 ) AND x12 ) )
x12 = ( ( ( ( ( ( ( ( NOT x4 AND NOT x2 ) AND NOT x12 ) AND NOT x3 ) OR ( ( NOT x4 AND NOT x2 ) AND x12 ) ) OR ( ( ( NOT x4 AND x2 ) AND x12 ) AND NOT x3 ) ) OR ( ( ( ( x4 AND NOT x5 ) AND NOT x2 ) AND NOT x12 ) AND NOT x3 ) ) OR ( ( ( x4 AND NOT x5 ) AND NOT x2 ) AND x12 ) ) OR ( ( ( ( x4 AND NOT x5 ) AND x2 ) AND x12 ) AND NOT x3 ) )
x13 = ( ( ( ( ( ( NOT x11 AND NOT x7 ) AND NOT x12 ) AND x3 ) AND NOT x10 ) OR ( ( NOT x11 AND x7 ) AND NOT x10 ) ) OR ( ( ( x11 AND NOT x12 ) AND x3 ) AND NOT x10 ) )
x14 = ( ( NOT x12 AND NOT x3 ) OR x12 ) \\
MAPK-REDUCED-1 & 17 & 4 & 13 & x1: v\_AKT, x2: v\_Apoptosis, x3: v\_DNA\_damage, x4: v\_EGFR, x5: v\_EGFR\_stimulus, x6: v\_ERK, x7: v\_FGFR3, x8: v\_FGFR3\_stimulus, x9: v\_FRS2, x10: v\_Growth\_Arrest, x11: v\_MSK, x12: v\_PI3K, x13: v\_PTEN, x14: v\_Proliferation, x15: v\_TGFBR\_stimulus, x16: v\_p14, x17: v\_p53 & x1 = ( x12 AND NOT x13 )
x2 = ( ( ( ( ( ( ( ( ( ( ( ( ( NOT x15 AND NOT x3 ) AND NOT x6 ) AND x17 ) AND NOT x4 ) AND NOT x7 ) AND NOT x9 ) AND NOT x1 ) AND NOT x11 ) OR ( ( ( ( ( ( ( NOT x15 AND NOT x3 ) AND NOT x6 ) AND x17 ) AND NOT x4 ) AND NOT x7 ) AND x9 ) AND NOT x1 ) ) OR ( ( ( ( ( ( NOT x15 AND NOT x3 ) AND NOT x6 ) AND x17 ) AND NOT x4 ) AND x7 ) AND NOT x1 ) ) OR ( ( ( ( ( NOT x15 AND NOT x3 ) AND NOT x6 ) AND x17 ) AND x4 ) AND NOT x1 ) ) OR ( ( ( ( NOT x15 AND x3 ) AND NOT x6 ) AND x17 ) AND NOT x1 ) ) OR ( ( ( x15 AND NOT x6 ) AND x17 ) AND NOT x1 ) )
x4 = ( ( ( ( ( ( NOT x5 AND NOT x15 ) AND x6 ) AND NOT x4 ) AND NOT x7 ) AND NOT x9 ) OR ( ( ( ( x5 AND NOT x15 ) AND NOT x4 ) AND NOT x7 ) AND NOT x9 ) )
x6 = ( ( ( ( ( ( ( ( ( ( ( NOT x15 AND NOT x3 ) AND NOT x6 ) AND NOT x17 ) AND NOT x4 ) AND NOT x7 ) AND x9 ) AND x11 ) OR ( ( ( ( ( ( NOT x15 AND NOT x3 ) AND NOT x6 ) AND NOT x17 ) AND NOT x4 ) AND x7 ) AND x11 ) ) OR ( ( ( ( ( NOT x15 AND NOT x3 ) AND NOT x6 ) AND NOT x17 ) AND x4 ) AND x11 ) ) OR ( ( ( ( ( ( NOT x15 AND NOT x3 ) AND x6 ) AND NOT x17 ) AND NOT x4 ) AND x7 ) AND x11 ) ) OR ( ( ( ( ( NOT x15 AND NOT x3 ) AND x6 ) AND NOT x17 ) AND x4 ) AND x11 ) )
x7 = ( ( ( ( x8 AND NOT x15 ) AND NOT x4 ) AND NOT x7 ) AND NOT x9 )
x9 = ( ( ( ( NOT x15 AND NOT x6 ) AND NOT x4 ) AND x7 ) AND NOT x9 )
x10 = ( x17 AND NOT x1 )
x11 = ( ( ( ( ( ( ( ( ( ( ( ( ( ( ( ( ( ( ( ( ( NOT x15 AND NOT x3 ) AND NOT x6 ) AND NOT x17 ) AND NOT x4 ) AND NOT x7 ) AND x9 ) AND NOT x11 ) OR ( ( ( ( ( ( NOT x15 AND NOT x3 ) AND NOT x6 ) AND NOT x17 ) AND NOT x4 ) AND x7 ) AND NOT x11 ) ) OR ( ( ( ( ( NOT x15 AND NOT x3 ) AND NOT x6 ) AND NOT x17 ) AND x4 ) AND NOT x11 ) ) OR ( ( ( ( ( ( ( NOT x15 AND NOT x3 ) AND NOT x6 ) AND x17 ) AND NOT x4 ) AND NOT x7 ) AND NOT x9 ) AND NOT x11 ) ) OR ( ( ( ( ( ( NOT x15 AND NOT x3 ) AND NOT x6 ) AND x17 ) AND NOT x4 ) AND NOT x7 ) AND x9 ) ) OR ( ( ( ( ( NOT x15 AND NOT x3 ) AND NOT x6 ) AND x17 ) AND NOT x4 ) AND x7 ) ) OR ( ( ( ( NOT x15 AND NOT x3 ) AND NOT x6 ) AND x17 ) AND x4 ) ) OR ( ( NOT x15 AND NOT x3 ) AND x6 ) ) OR ( ( ( ( ( ( ( NOT x15 AND x3 ) AND NOT x6 ) AND NOT x17 ) AND NOT x4 ) AND NOT x7 ) AND NOT x9 ) AND NOT x11 ) ) OR ( ( ( ( ( ( NOT x15 AND x3 ) AND NOT x6 ) AND NOT x17 ) AND NOT x4 ) AND NOT x7 ) AND x9 ) ) OR ( ( ( ( ( NOT x15 AND x3 ) AND NOT x6 ) AND NOT x17 ) AND NOT x4 ) AND x7 ) ) OR ( ( ( ( NOT x15 AND x3 ) AND NOT x6 ) AND NOT x17 ) AND x4 ) ) OR ( ( ( NOT x15 AND x3 ) AND NOT x6 ) AND x17 ) ) OR ( ( NOT x15 AND x3 ) AND x6 ) ) OR x15 )
x12 = ( ( ( ( ( ( NOT x15 AND NOT x4 ) AND NOT x9 ) AND x12 ) OR ( ( NOT x15 AND NOT x4 ) AND x9 ) ) OR ( NOT x15 AND x4 ) ) OR x15 )
x13 = x17
x14 = ( ( ( ( ( ( ( ( ( ( ( NOT x15 AND NOT x3 ) AND x6 ) AND x12 ) AND x1 ) AND x11 ) OR ( ( ( ( ( ( ( ( NOT x15 AND x3 ) AND x6 ) AND NOT x17 ) AND NOT x4 ) AND NOT x7 ) AND x12 ) AND x1 ) AND x11 ) ) OR ( ( ( ( ( ( ( NOT x15 AND x3 ) AND x6 ) AND NOT x17 ) AND NOT x4 ) AND x7 ) AND x12 ) AND x11 ) ) OR ( ( ( ( ( ( NOT x15 AND x3 ) AND x6 ) AND NOT x17 ) AND x4 ) AND x12 ) AND x11 ) ) OR ( ( ( ( ( ( NOT x15 AND x3 ) AND x6 ) AND x17 ) AND x12 ) AND x1 ) AND x11 ) ) OR ( ( ( ( x15 AND x6 ) AND NOT x17 ) AND x12 ) AND x11 ) ) OR ( ( ( ( ( x15 AND x6 ) AND x17 ) AND x12 ) AND x1 ) AND x11 ) )
x16 = ( ( ( ( ( ( ( ( ( ( ( ( ( ( ( ( ( ( ( ( ( ( ( NOT x15 AND NOT x3 ) AND NOT x6 ) AND NOT x17 ) AND x1 ) AND x11 ) OR ( ( ( ( ( ( ( ( NOT x15 AND NOT x3 ) AND NOT x6 ) AND x17 ) AND NOT x4 ) AND NOT x7 ) AND NOT x9 ) AND x1 ) AND x11 ) ) OR ( ( ( ( ( ( ( NOT x15 AND NOT x3 ) AND NOT x6 ) AND x17 ) AND NOT x4 ) AND NOT x7 ) AND x9 ) AND x11 ) ) OR ( ( ( ( ( ( NOT x15 AND NOT x3 ) AND NOT x6 ) AND x17 ) AND NOT x4 ) AND x7 ) AND x11 ) ) OR ( ( ( ( ( NOT x15 AND NOT x3 ) AND NOT x6 ) AND x17 ) AND x4 ) AND x11 ) ) OR ( ( ( ( ( NOT x15 AND NOT x3 ) AND x6 ) AND NOT x17 ) AND x1 ) AND x11 ) ) OR ( ( ( ( ( ( ( NOT x15 AND NOT x3 ) AND x6 ) AND x17 ) AND NOT x4 ) AND NOT x7 ) AND x1 ) AND x11 ) ) OR ( ( ( ( ( ( NOT x15 AND NOT x3 ) AND x6 ) AND x17 ) AND NOT x4 ) AND x7 ) AND x11 ) ) OR ( ( ( ( ( NOT x15 AND NOT x3 ) AND x6 ) AND x17 ) AND x4 ) AND x11 ) ) OR ( ( ( ( ( ( ( ( NOT x15 AND x3 ) AND NOT x6 ) AND NOT x17 ) AND NOT x4 ) AND NOT x7 ) AND NOT x9 ) AND x1 ) AND x11 ) ) OR ( ( ( ( ( ( ( NOT x15 AND x3 ) AND NOT x6 ) AND NOT x17 ) AND NOT x4 ) AND NOT x7 ) AND x9 ) AND x11 ) ) OR ( ( ( ( ( ( NOT x15 AND x3 ) AND NOT x6 ) AND NOT x17 ) AND NOT x4 ) AND x7 ) AND x11 ) ) OR ( ( ( ( ( NOT x15 AND x3 ) AND NOT x6 ) AND NOT x17 ) AND x4 ) AND x11 ) ) OR ( ( ( ( NOT x15 AND x3 ) AND NOT x6 ) AND x17 ) AND x11 ) ) OR ( ( ( ( ( ( ( NOT x15 AND x3 ) AND x6 ) AND NOT x17 ) AND NOT x4 ) AND NOT x7 ) AND x1 ) AND x11 ) ) OR ( ( ( ( ( ( NOT x15 AND x3 ) AND x6 ) AND NOT x17 ) AND NOT x4 ) AND x7 ) AND x11 ) ) OR ( ( ( ( ( NOT x15 AND x3 ) AND x6 ) AND NOT x17 ) AND x4 ) AND x11 ) ) OR ( ( ( ( NOT x15 AND x3 ) AND x6 ) AND x17 ) AND x11 ) ) OR ( x15 AND x11 ) )
x17 = ( ( ( ( ( ( ( ( ( ( ( ( ( ( ( ( ( ( ( ( ( ( ( ( ( ( ( ( ( ( ( ( ( ( ( ( ( ( ( ( ( NOT x15 AND NOT x3 ) AND NOT x6 ) AND NOT x17 ) AND NOT x4 ) AND NOT x7 ) AND x9 ) AND NOT x1 ) AND NOT x11 ) OR ( ( ( ( ( ( ( ( ( NOT x15 AND NOT x3 ) AND NOT x6 ) AND NOT x17 ) AND NOT x4 ) AND NOT x7 ) AND x9 ) AND x1 ) AND NOT x11 ) AND x16 ) ) OR ( ( ( ( ( ( ( NOT x15 AND NOT x3 ) AND NOT x6 ) AND NOT x17 ) AND NOT x4 ) AND x7 ) AND NOT x1 ) AND NOT x11 ) ) OR ( ( ( ( ( ( ( ( NOT x15 AND NOT x3 ) AND NOT x6 ) AND NOT x17 ) AND NOT x4 ) AND x7 ) AND x1 ) AND NOT x11 ) AND x16 ) ) OR ( ( ( ( ( ( NOT x15 AND NOT x3 ) AND NOT x6 ) AND NOT x17 ) AND x4 ) AND NOT x1 ) AND NOT x11 ) ) OR ( ( ( ( ( ( ( NOT x15 AND NOT x3 ) AND NOT x6 ) AND NOT x17 ) AND x4 ) AND x1 ) AND NOT x11 ) AND x16 ) ) OR ( ( ( ( ( ( ( ( NOT x15 AND NOT x3 ) AND NOT x6 ) AND x17 ) AND NOT x4 ) AND NOT x7 ) AND NOT x9 ) AND NOT x11 ) AND x16 ) ) OR ( ( ( ( ( ( ( NOT x15 AND NOT x3 ) AND NOT x6 ) AND x17 ) AND NOT x4 ) AND NOT x7 ) AND x9 ) AND x16 ) ) OR ( ( ( ( ( ( NOT x15 AND NOT x3 ) AND NOT x6 ) AND x17 ) AND NOT x4 ) AND x7 ) AND x16 ) ) OR ( ( ( ( ( NOT x15 AND NOT x3 ) AND NOT x6 ) AND x17 ) AND x4 ) AND x16 ) ) OR ( ( ( ( ( ( ( NOT x15 AND NOT x3 ) AND x6 ) AND NOT x17 ) AND NOT x4 ) AND x7 ) AND NOT x1 ) AND NOT x11 ) ) OR ( ( ( ( ( ( ( ( NOT x15 AND NOT x3 ) AND x6 ) AND NOT x17 ) AND NOT x4 ) AND x7 ) AND x1 ) AND NOT x11 ) AND x16 ) ) OR ( ( ( ( ( ( NOT x15 AND NOT x3 ) AND x6 ) AND NOT x17 ) AND x4 ) AND NOT x1 ) AND NOT x11 ) ) OR ( ( ( ( ( ( ( NOT x15 AND NOT x3 ) AND x6 ) AND NOT x17 ) AND x4 ) AND x1 ) AND NOT x11 ) AND x16 ) ) OR ( ( ( ( ( ( ( NOT x15 AND NOT x3 ) AND x6 ) AND x17 ) AND NOT x4 ) AND NOT x7 ) AND NOT x11 ) AND x16 ) ) OR ( ( ( ( ( ( NOT x15 AND NOT x3 ) AND x6 ) AND x17 ) AND NOT x4 ) AND x7 ) AND x16 ) ) OR ( ( ( ( ( NOT x15 AND NOT x3 ) AND x6 ) AND x17 ) AND x4 ) AND x16 ) ) OR ( ( ( ( ( ( ( NOT x15 AND x3 ) AND NOT x6 ) AND NOT x17 ) AND NOT x4 ) AND NOT x7 ) AND NOT x9 ) AND NOT x1 ) ) OR ( ( ( ( ( ( ( ( NOT x15 AND x3 ) AND NOT x6 ) AND NOT x17 ) AND NOT x4 ) AND NOT x7 ) AND NOT x9 ) AND x1 ) AND NOT x11 ) ) OR ( ( ( ( ( ( ( ( ( NOT x15 AND x3 ) AND NOT x6 ) AND NOT x17 ) AND NOT x4 ) AND NOT x7 ) AND NOT x9 ) AND x1 ) AND x11 ) AND x16 ) ) OR ( ( ( ( ( ( NOT x15 AND x3 ) AND NOT x6 ) AND NOT x17 ) AND NOT x4 ) AND NOT x7 ) AND x9 ) ) OR ( ( ( ( ( NOT x15 AND x3 ) AND NOT x6 ) AND NOT x17 ) AND NOT x4 ) AND x7 ) ) OR ( ( ( ( NOT x15 AND x3 ) AND NOT x6 ) AND NOT x17 ) AND x4 ) ) OR ( ( ( NOT x15 AND x3 ) AND NOT x6 ) AND x17 ) ) OR ( ( ( ( ( ( NOT x15 AND x3 ) AND x6 ) AND NOT x17 ) AND NOT x4 ) AND NOT x7 ) AND NOT x1 ) ) OR ( ( ( ( ( ( ( NOT x15 AND x3 ) AND x6 ) AND NOT x17 ) AND NOT x4 ) AND NOT x7 ) AND x1 ) AND NOT x11 ) ) OR ( ( ( ( ( ( ( ( NOT x15 AND x3 ) AND x6 ) AND NOT x17 ) AND NOT x4 ) AND NOT x7 ) AND x1 ) AND x11 ) AND x16 ) ) OR ( ( ( ( ( NOT x15 AND x3 ) AND x6 ) AND NOT x17 ) AND NOT x4 ) AND x7 ) ) OR ( ( ( ( NOT x15 AND x3 ) AND x6 ) AND NOT x17 ) AND x4 ) ) OR ( ( ( NOT x15 AND x3 ) AND x6 ) AND x17 ) ) OR ( ( ( x15 AND NOT x3 ) AND NOT x17 ) AND NOT x1 ) ) OR ( ( ( ( x15 AND NOT x3 ) AND NOT x17 ) AND x1 ) AND x16 ) ) OR ( ( ( x15 AND NOT x3 ) AND x17 ) AND x16 ) ) OR ( x15 AND x3 ) ) \\
BUDDING-YEAST-CELL-CYCLE-2009 & 18 & 0 & 18 & x1: v\_B, x2: v\_CD, x3: v\_CKI, x4: v\_Cdc14, x5: v\_Cdc20, x6: v\_Cdh1, x7: v\_Clb2, x8: v\_Clb5, x9: v\_Cln2, x10: v\_Cln3, x11: v\_FEAR, x12: v\_M, x13: v\_MEN, x14: v\_S, x15: v\_SFF, x16: v\_SMBF, x17: v\_Swi5, x18: v\_Yhp1 & x1 = ( ( ( x9 AND NOT x2 ) OR ( x1 AND NOT x2 ) ) OR ( x8 AND NOT x2 ) )
x2 = ( ( x12 AND ( x4 AND x11 ) ) AND NOT x2 )
x3 = ( ( ( x17 AND NOT ( ( x7 OR x9 ) OR x8 ) ) OR ( x3 AND NOT ( ( x7 OR x9 ) OR x8 ) ) ) OR ( x4 AND x17 ) )
x4 = ( x11 AND x13 )
x5 = ( x12 AND ( x15 AND x7 ) )
x6 = ( x4 OR NOT ( ( ( x4 OR x8 ) OR x9 ) OR x7 ) )
x7 = ( ( ( x1 AND ( NOT x5 OR NOT x6 ) ) AND NOT x3 ) OR ( ( x7 AND ( ( NOT x5 OR NOT x6 ) AND x15 ) ) AND NOT x3 ) )
x8 = ( x16 AND ( NOT x5 OR ( NOT x3 AND NOT x5 ) ) )
x9 = x16
x10 = NOT x18
x11 = x5
x12 = ( ( x12 AND NOT x2 ) OR ( ( x14 AND x7 ) AND NOT x2 ) )
x13 = ( x11 AND x7 )
x14 = ( ( ( x8 AND NOT x2 ) OR ( x7 AND NOT x2 ) ) OR ( x14 AND NOT x2 ) )
x15 = ( ( x7 AND x15 ) OR ( ( x1 AND ( NOT x5 OR NOT x6 ) ) AND NOT x3 ) )
x16 = ( ( ( x10 AND NOT x7 ) OR ( x16 AND NOT x7 ) ) OR ( x9 AND NOT x7 ) )
x17 = ( ( x4 AND x15 ) OR ( x15 AND NOT x7 ) )
x18 = x16 \\
REGULATION-OF-L-ARABINOSE-OPERON & 13 & 4 & 9 & x1: v\_A, x2: v\_Ae, x3: v\_Aem, x4: v\_Am, x5: v\_C, x6: v\_E, x7: v\_Ge, x8: v\_L, x9: v\_MS, x10: v\_MT, x11: v\_S\_2\_Ara\_, x12: v\_S\_7\_Ara\_, x13: v\_T & x1 = ( x2 AND x13 )
x4 = ( ( x3 AND x13 ) OR x2 )
x5 = NOT x7
x6 = x9
x8 = ( x11 AND NOT x12 )
x9 = ( x12 AND x5 )
x10 = ( x12 AND x5 )
x12 = ( x11 AND ( x1 OR x4 ) )
x13 = x10 \\
HEPATOCELLULAR-CARCINOMA-REDUCED & 19 & 0 & 19 & x1: v\_AKT, x2: v\_AXIN2, x3: v\_Bcatenin\_memb, x4: v\_Bcatenin\_nuc, x5: v\_Dest\_compl, x6: v\_Ecadherin, x7: v\_GLI, x8: v\_GSK3B, x9: v\_MEK, x10: v\_NOTCH, x11: v\_SMAD, x12: v\_SNAI1, x13: v\_SNAI2, x14: v\_SOS\_GRB2, x15: v\_TGFBR, x16: v\_TWIST1, x17: v\_ZEB1, x18: v\_ZEB2, x19: v\_miR200 & x1 = ( x11 OR ( x14 OR ( NOT x8 OR x4 ) ) )
x2 = ( x2 OR x4 )
x3 = ( x6 AND NOT x4 )
x4 = ( NOT x5 AND ( NOT x3 AND ( x11 OR ( x7 OR NOT x6 ) ) ) )
x5 = ( ( x8 AND ( x2 AND x4 ) ) OR ( x8 AND x5 ) )
x6 = ( x3 AND ( NOT x12 OR ( ( NOT x10 AND NOT x11 ) OR ( NOT x17 OR ( NOT x18 OR ( NOT x16 OR NOT x13 ) ) ) ) ) )
x7 = ( x4 OR ( x11 OR x7 ) )
x8 = ( NOT x7 AND NOT x1 )
x9 = ( x14 OR ( NOT x8 OR ( x4 OR NOT ( NOT x9 OR NOT x12 ) ) ) )
x10 = ( x14 OR ( NOT x8 OR ( x4 OR x11 ) ) )
x11 = ( ( x9 OR x15 ) AND ( x17 OR NOT x18 ) )
x12 = ( x7 OR ( x11 OR ( x4 OR ( x15 OR ( x10 OR ( x9 OR ( x1 OR NOT x8 ) ) ) ) ) ) )
x13 = ( x9 OR ( x4 OR ( x13 OR x16 ) ) )
x14 = ( ( x4 OR x15 ) AND NOT x9 )
x15 = ( x12 OR ( x16 OR x7 ) )
x16 = ( x1 OR ( x4 OR x12 ) )
x17 = ( x12 AND NOT x19 )
x18 = ( x12 AND NOT x19 )
x19 = ( NOT x12 AND ( NOT x17 AND NOT x18 ) ) \\
MAPK-REDUCED-3 & 16 & 4 & 12 & x1: v\_Apoptosis, x2: v\_DNA\_damage, x3: v\_EGFR\_stimulus, x4: v\_ERK, x5: v\_FGFR3\_stimulus, x6: v\_GADD45, x7: v\_GRB2, x8: v\_Growth\_Arrest, x9: v\_JNK, x10: v\_MDM2, x11: v\_PI3K, x12: v\_PLCG, x13: v\_Proliferation, x14: v\_RAS, x15: v\_TGFBR\_stimulus, x16: v\_p38 & x1 = ( ( ( ( ( ( NOT x2 AND NOT x4 ) AND x16 ) AND x9 ) AND NOT x10 ) OR ( ( ( ( x2 AND NOT x4 ) AND NOT x16 ) AND x9 ) AND NOT x10 ) ) OR ( ( ( x2 AND NOT x4 ) AND x16 ) AND x9 ) )
x4 = ( ( ( ( ( ( ( ( ( ( ( ( ( NOT x2 AND NOT x4 ) AND NOT x16 ) AND NOT x9 ) AND NOT x12 ) AND x14 ) OR ( ( ( ( ( NOT x2 AND NOT x4 ) AND NOT x16 ) AND NOT x9 ) AND x12 ) AND NOT x11 ) ) OR ( ( ( ( ( ( NOT x2 AND NOT x4 ) AND NOT x16 ) AND NOT x9 ) AND x12 ) AND x11 ) AND x14 ) ) OR ( ( ( ( NOT x2 AND x4 ) AND NOT x16 ) AND NOT x9 ) AND x14 ) ) OR ( ( ( ( ( x2 AND NOT x4 ) AND NOT x16 ) AND NOT x9 ) AND NOT x12 ) AND x14 ) ) OR ( ( ( ( ( x2 AND NOT x4 ) AND NOT x16 ) AND NOT x9 ) AND x12 ) AND NOT x11 ) ) OR ( ( ( ( ( ( ( x2 AND NOT x4 ) AND NOT x16 ) AND NOT x9 ) AND x12 ) AND x11 ) AND NOT x14 ) AND NOT x10 ) ) OR ( ( ( ( ( ( x2 AND NOT x4 ) AND NOT x16 ) AND NOT x9 ) AND x12 ) AND x11 ) AND x14 ) ) OR ( ( ( ( x2 AND x4 ) AND NOT x16 ) AND NOT x9 ) AND x14 ) )
x6 = ( ( ( ( ( ( NOT x15 AND NOT x2 ) AND x16 ) AND NOT x10 ) OR ( ( ( NOT x15 AND x2 ) AND NOT x16 ) AND NOT x10 ) ) OR ( ( NOT x15 AND x2 ) AND x16 ) ) OR x15 )
x7 = ( ( ( ( ( ( ( ( ( ( NOT x3 AND NOT x5 ) AND NOT x15 ) AND x4 ) AND NOT x7 ) AND NOT x12 ) OR ( ( NOT x3 AND NOT x5 ) AND x15 ) ) OR ( ( ( ( NOT x3 AND x5 ) AND NOT x15 ) AND NOT x7 ) AND NOT x12 ) ) OR ( ( NOT x3 AND x5 ) AND x15 ) ) OR ( ( ( x3 AND NOT x15 ) AND NOT x7 ) AND NOT x12 ) ) OR ( x3 AND x15 ) )
x8 = ( ( ( ( NOT x2 AND x16 ) AND NOT x10 ) OR ( ( x2 AND NOT x16 ) AND NOT x10 ) ) OR ( x2 AND x16 ) )
x9 = ( ( ( ( ( ( ( ( ( ( ( ( ( ( ( ( ( ( ( NOT x15 AND NOT x2 ) AND NOT x4 ) AND NOT x16 ) AND NOT x6 ) AND x14 ) OR ( ( ( ( NOT x15 AND NOT x2 ) AND NOT x4 ) AND NOT x16 ) AND x6 ) ) OR ( ( ( ( ( NOT x15 AND NOT x2 ) AND NOT x4 ) AND x16 ) AND x6 ) AND x14 ) ) OR ( ( ( ( NOT x15 AND NOT x2 ) AND x4 ) AND x6 ) AND x14 ) ) OR ( ( ( NOT x15 AND x2 ) AND NOT x4 ) AND NOT x16 ) ) OR ( ( ( ( ( NOT x15 AND x2 ) AND NOT x4 ) AND x16 ) AND NOT x6 ) AND x14 ) ) OR ( ( ( ( NOT x15 AND x2 ) AND NOT x4 ) AND x16 ) AND x6 ) ) OR ( ( ( ( NOT x15 AND x2 ) AND x4 ) AND NOT x6 ) AND x14 ) ) OR ( ( ( NOT x15 AND x2 ) AND x4 ) AND x6 ) ) OR ( ( ( x15 AND NOT x2 ) AND NOT x4 ) AND NOT x16 ) ) OR ( ( ( ( ( x15 AND NOT x2 ) AND NOT x4 ) AND x16 ) AND NOT x6 ) AND x14 ) ) OR ( ( ( ( x15 AND NOT x2 ) AND NOT x4 ) AND x16 ) AND x6 ) ) OR ( ( ( ( x15 AND NOT x2 ) AND x4 ) AND NOT x6 ) AND x14 ) ) OR ( ( ( x15 AND NOT x2 ) AND x4 ) AND x6 ) ) OR ( x15 AND x2 ) )
x10 = ( ( ( ( ( ( NOT x2 AND NOT x4 ) AND NOT x16 ) AND x11 ) OR ( ( ( ( x2 AND NOT x4 ) AND NOT x16 ) AND NOT x11 ) AND NOT x10 ) ) OR ( ( ( x2 AND NOT x4 ) AND NOT x16 ) AND x11 ) ) OR ( ( ( x2 AND x4 ) AND NOT x16 ) AND NOT x10 ) )
x11 = ( ( NOT x7 AND x11 ) OR x7 )
x12 = ( ( ( ( ( ( NOT x3 AND NOT x5 ) AND x4 ) AND NOT x7 ) AND NOT x12 ) OR ( ( ( NOT x3 AND x5 ) AND NOT x7 ) AND NOT x12 ) ) OR ( ( x3 AND NOT x7 ) AND NOT x12 ) )
x13 = ( ( ( ( ( NOT x2 AND x4 ) AND NOT x16 ) AND x11 ) OR ( ( ( ( NOT x2 AND x4 ) AND x16 ) AND x11 ) AND x10 ) ) OR ( ( ( ( x2 AND x4 ) AND NOT x16 ) AND x11 ) AND x10 ) )
x14 = ( ( ( ( NOT x4 AND NOT x7 ) AND x12 ) OR ( NOT x4 AND x7 ) ) OR ( x4 AND x12 ) )
x16 = ( ( ( ( ( ( ( ( ( ( ( ( ( ( ( ( ( ( ( NOT x15 AND NOT x2 ) AND NOT x4 ) AND NOT x16 ) AND NOT x6 ) AND x14 ) OR ( ( ( ( NOT x15 AND NOT x2 ) AND NOT x4 ) AND NOT x16 ) AND x6 ) ) OR ( ( ( ( ( NOT x15 AND NOT x2 ) AND NOT x4 ) AND x16 ) AND x6 ) AND x14 ) ) OR ( ( ( ( NOT x15 AND NOT x2 ) AND x4 ) AND x6 ) AND x14 ) ) OR ( ( ( NOT x15 AND x2 ) AND NOT x4 ) AND NOT x16 ) ) OR ( ( ( ( ( NOT x15 AND x2 ) AND NOT x4 ) AND x16 ) AND NOT x6 ) AND x14 ) ) OR ( ( ( ( NOT x15 AND x2 ) AND NOT x4 ) AND x16 ) AND x6 ) ) OR ( ( ( ( NOT x15 AND x2 ) AND x4 ) AND NOT x6 ) AND x14 ) ) OR ( ( ( NOT x15 AND x2 ) AND x4 ) AND x6 ) ) OR ( ( ( x15 AND NOT x2 ) AND NOT x4 ) AND NOT x16 ) ) OR ( ( ( ( ( x15 AND NOT x2 ) AND NOT x4 ) AND x16 ) AND NOT x6 ) AND x14 ) ) OR ( ( ( ( x15 AND NOT x2 ) AND NOT x4 ) AND x16 ) AND x6 ) ) OR ( ( ( ( x15 AND NOT x2 ) AND x4 ) AND NOT x6 ) AND x14 ) ) OR ( ( ( x15 AND NOT x2 ) AND x4 ) AND x6 ) ) OR ( x15 AND x2 ) ) \\
LAC-OPERON & 13 & 3 & 10 & x1: v\_A, x2: v\_Am, x3: v\_B, x4: v\_C, x5: v\_Ge, x6: v\_L, x7: v\_Le, x8: v\_Lem, x9: v\_Lm, x10: v\_M, x11: v\_P, x12: v\_R, x13: v\_Rm & x1 = ( x6 AND x3 )
x2 = ( x9 OR x6 )
x3 = x10
x4 = NOT x5
x6 = ( ( x7 AND x11 ) AND NOT x5 )
x9 = ( ( ( x8 AND x11 ) AND NOT x5 ) OR ( x7 AND NOT x5 ) )
x10 = ( x4 AND NOT ( x12 OR x13 ) )
x11 = x10
x12 = NOT ( x2 OR x1 )
x13 = ( x12 OR NOT ( ( x12 OR x2 ) OR x1 ) ) \\
CD4-T-CELL-DIFFERENTIATION-AND-PLASTICITY & 18 & 6 & 12 & x1: v\_BCL6, x2: v\_FOXP3, x3: v\_GATA3, x4: v\_IFNG, x5: v\_IFNGe, x6: v\_IL10, x7: v\_IL10e, x8: v\_IL2, x9: v\_IL21, x10: v\_IL21e, x11: v\_IL2e, x12: v\_IL4, x13: v\_IL4e, x14: v\_IL9, x15: v\_RORGT, x16: v\_TBET, x17: v\_TGFB, x18: v\_TGFBe & x1 = ( x9 AND NOT ( ( x8 OR x16 ) OR x17 ) )
x2 = ( ( x8 AND ( x2 OR x17 ) ) AND NOT ( x9 OR x15 ) )
x3 = ( ( ( x12 AND x8 ) AND NOT ( ( ( ( x16 OR x1 ) OR x17 ) OR x4 ) OR x9 ) ) OR ( x3 AND NOT ( ( ( ( x16 OR x1 ) OR x17 ) OR x4 ) OR x9 ) ) )
x4 = ( ( ( x5 AND NOT ( ( ( x9 OR x12 ) OR x6 ) OR x14 ) ) OR ( x16 AND NOT ( ( ( ( ( ( x9 OR x12 ) OR x1 ) OR x6 ) OR x14 ) OR x17 ) OR x3 ) ) ) OR ( x4 AND NOT ( ( ( ( ( ( x9 OR x12 ) OR x1 ) OR x6 ) OR x14 ) OR x17 ) OR x3 ) ) )
x6 = ( ( x6 AND ( ( ( x3 OR x4 ) OR x9 ) OR x17 ) ) OR x7 )
x8 = ( ( x11 AND NOT ( ( x9 OR x4 ) OR x6 ) ) OR ( x8 AND NOT ( ( ( x9 OR x2 ) OR x4 ) OR x6 ) ) )
x9 = ( ( ( ( x10 AND NOT ( ( ( ( x12 OR x4 ) OR x8 ) OR x14 ) OR x6 ) ) OR ( x1 AND NOT ( ( ( ( x12 OR x4 ) OR x8 ) OR x14 ) OR x6 ) ) ) OR ( x15 AND NOT ( ( ( ( x12 OR x4 ) OR x8 ) OR x14 ) OR x6 ) ) ) OR ( x9 AND NOT ( ( ( ( x12 OR x4 ) OR x8 ) OR x14 ) OR x6 ) ) )
x12 = ( ( x13 AND NOT ( x9 OR x4 ) ) OR ( ( x3 AND ( x8 OR x12 ) ) AND NOT ( ( x16 OR x9 ) OR x4 ) ) )
x14 = ( ( x12 AND ( ( x8 AND x6 ) OR x17 ) ) AND NOT ( x9 OR x4 ) )
x15 = ( ( x9 AND x17 ) AND NOT ( ( ( x16 OR x3 ) OR x1 ) OR x2 ) )
x16 = ( ( x4 AND NOT ( ( ( ( x14 OR x3 ) OR x1 ) OR x9 ) OR x12 ) ) OR ( x16 AND NOT ( ( ( ( x14 OR x3 ) OR x1 ) OR x9 ) OR x12 ) ) )
x17 = ( ( x18 OR ( x2 AND NOT x9 ) ) OR ( x17 AND NOT x9 ) ) \\
HUMAN-GONADAL-SEX-DETERMINATION & 19 & 0 & 19 & x1: v\_AMH, x2: v\_CBX2, x3: v\_CTNNB1, x4: v\_DHH, x5: v\_DKK1, x6: v\_DMRT1, x7: v\_FGF9, x8: v\_FOXL2, x9: v\_GATA4, x10: v\_NR0B1, x11: v\_NR5A1, x12: v\_PGD2, x13: v\_RSPO1, x14: v\_SOX9, x15: v\_SRY, x16: v\_UGR, x17: v\_WNT4, x18: v\_WT1mKTS, x19: v\_WT1pKTS & x1 = ( ( x14 AND ( ( ( x9 AND x18 ) AND x11 ) OR ( x9 AND x11 ) ) ) AND NOT ( x10 AND x3 ) )
x2 = ( x16 AND NOT ( x10 AND ( x17 AND x3 ) ) )
x3 = ( ( x13 AND NOT ( x15 OR ( x14 AND x1 ) ) ) OR ( x17 AND NOT ( x15 OR ( x14 AND x1 ) ) ) )
x4 = x14
x5 = ( x15 OR x14 )
x6 = ( ( x14 AND NOT x8 ) OR ( x15 AND NOT x8 ) )
x7 = ( x14 AND NOT x17 )
x8 = ( ( x17 AND x3 ) AND NOT ( x14 OR x6 ) )
x9 = ( ( ( x15 OR x16 ) OR x17 ) OR x11 )
x10 = ( ( x18 AND NOT ( x11 AND x14 ) ) OR ( ( x17 AND x3 ) AND NOT ( x11 AND x14 ) ) )
x11 = ( ( ( ( x9 AND NOT ( x10 AND x17 ) ) OR ( x16 AND NOT ( x10 AND x17 ) ) ) OR ( x2 AND NOT ( x10 AND x17 ) ) ) OR ( x18 AND NOT ( x10 AND x17 ) ) )
x12 = x14
x13 = ( ( x17 AND NOT x5 ) OR ( x3 AND NOT x5 ) )
x14 = ( ( ( ( ( ( x9 AND ( x15 AND x11 ) ) AND NOT ( ( x3 OR x8 ) OR x17 ) ) OR ( ( x2 AND x15 ) AND NOT ( ( x3 OR x8 ) OR x17 ) ) ) OR ( ( x7 AND x14 ) AND NOT ( ( x3 OR x8 ) OR x17 ) ) ) OR ( x12 AND NOT ( ( x3 OR x8 ) OR x17 ) ) ) OR ( x15 AND NOT ( ( x3 OR x8 ) OR x17 ) ) )
x15 = ( ( ( ( ( x9 AND ( ( x11 AND x2 ) AND x19 ) ) AND NOT x3 ) OR ( x15 AND NOT x3 ) ) OR ( ( x2 AND ( x18 AND x11 ) ) AND NOT x3 ) ) OR ( x14 AND NOT x3 ) )
x16 = ( x16 AND NOT ( x11 OR x17 ) )
x17 = ( ( ( ( x9 AND NOT ( x7 OR x5 ) ) OR ( x3 AND NOT ( x7 OR x5 ) ) ) OR ( x13 AND NOT ( x7 OR x5 ) ) ) OR ( x10 AND NOT ( x7 OR x5 ) ) )
x18 = ( x16 OR x9 )
x19 = ( ( x16 AND NOT ( x17 AND x3 ) ) OR ( x9 AND NOT ( x17 AND x3 ) ) ) \\
COLORECTAL-TUMORIGENESIS-REVERSION-SWITCH & 17 & 0 & 17 & x1: v\_BHLHE40, x2: v\_CDX2, x3: v\_DDIT3, x4: v\_FOSL2, x5: v\_FOXO3, x6: v\_JUN, x7: v\_KLF4, x8: v\_KLF5, x9: v\_KLF6, x10: v\_MAFF, x11: v\_MYC, x12: v\_NFIA, x13: v\_NFIL3, x14: v\_RELB, x15: v\_SMARCA4, x16: v\_SREBF1, x17: v\_YY1 & x1 = ( x9 OR x1 )
x2 = ( x11 OR ( x2 OR x2 ) )
x3 = ( x3 OR ( x8 OR ( x3 OR ( x6 OR ( ( x13 AND x3 ) OR x3 ) ) ) ) )
x4 = ( ( x1 OR x8 ) AND NOT x11 )
x5 = ( x5 AND x6 )
x6 = ( ( x8 AND ( x13 AND NOT x17 ) ) OR ( ( x8 AND ( x3 AND NOT x17 ) ) OR ( ( ( x5 OR x13 ) AND NOT x17 ) OR ( ( ( x8 OR x13 ) AND NOT x17 ) OR ( ( x3 AND ( x13 AND NOT x17 ) ) OR ( ( ( x8 OR x3 ) AND NOT x17 ) OR ( ( x3 AND NOT x17 ) OR ( ( x8 AND NOT x17 ) OR ( ( x13 AND NOT x17 ) OR ( ( ( x3 OR x13 ) AND NOT x17 ) OR ( ( ( x5 OR x3 ) AND NOT x17 ) OR ( ( x8 OR x5 ) AND NOT x17 ) ) ) ) ) ) ) ) ) ) ) )
x7 = ( ( x1 OR x5 ) AND NOT x11 )
x8 = ( ( x6 AND ( x14 AND NOT x17 ) ) OR ( ( x14 AND NOT x17 ) OR ( ( x6 AND NOT x17 ) OR ( ( ( x6 OR x14 ) AND NOT x17 ) OR ( ( ( x5 OR x14 ) AND NOT x17 ) OR ( ( ( x6 OR x5 ) AND NOT x17 ) OR ( ( ( x4 OR x14 ) AND NOT x17 ) OR ( ( x6 OR x4 ) AND NOT x17 ) ) ) ) ) ) ) )
x9 = ( ( x9 AND x10 ) OR x9 )
x10 = ( x5 OR x1 )
x11 = ( x2 OR ( x15 OR x2 ) )
x12 = ( x11 OR ( x16 AND x11 ) )
x13 = ( x3 OR ( x3 OR x6 ) )
x14 = ( x8 OR ( x14 OR x14 ) )
x15 = x11
x16 = ( x17 OR ( x12 OR x17 ) )
x17 = ( x17 OR ( x16 OR ( x17 OR ( x11 OR x17 ) ) ) ) \\
NEUROTRANSMITTER-SIGNALING-PATHWAY & 16 & 2 & 14 & x1: v\_Adenylate\_cyclase, x2: v\_COMT, x3: v\_Calcineurin, x4: v\_Calcium, x5: v\_DARPP32, x6: v\_Dopamine, x7: v\_Dopamine\_Receptor\_1, x8: v\_Dopamine\_Receptor\_2, x9: v\_Exocytosis, x10: v\_Glutamate, x11: v\_Glutamate\_Receptor, x12: v\_Packaging\_Proteins, x13: v\_Phospholipase\_C, x14: v\_Protein\_Kinase\_A, x15: v\_Protein\_Phosphatase\_1, x16: v\_Tryosine\_hydroxylase & x1 = ( x7 AND NOT x8 )
x2 = x6
x3 = x4
x4 = ( x13 OR x11 )
x5 = ( x14 AND NOT x3 )
x6 = ( x16 AND NOT x2 )
x7 = x6
x8 = x6
x9 = x12
x11 = ( ( x14 AND x10 ) AND NOT x15 )
x12 = x11
x13 = x8
x14 = x1
x15 = NOT x5 \\
JNK-PATHWAY & 19 & 6 & 13 & x1: v\_3a, x2: v\_3b, x3: v\_7a, x4: v\_AP\_1\_complex, x5: v\_ATF2\_phosphorylated, x6: v\_Apoptosis\_phenotype, x7: v\_Autophagy\_phenotype, x8: v\_BCL2\_phosphorylated, x9: v\_Innate\_Immunity\_phenotype, x10: v\_MAP2K4\_phosphorylated, x11: v\_MAP2K7\_phosphorylated, x12: v\_MEKK1\_4\_complex, x13: v\_MLK1\_2\_3\_complex, x14: v\_S, x15: v\_SARS\_CoV\_1\_proteins\_complex, x16: v\_TP53\_phosphorylated, x17: v\_TP53\_signalling\_phenotype, x18: v\_csa12\_JNK\_complex\_cell, x19: v\_csa1\_JNK\_complex\_cell & x4 = ( x19 OR x2 )
x5 = x19
x6 = NOT x8
x7 = x8
x8 = x19
x9 = x4
x10 = ( x12 OR x15 )
x11 = ( x13 OR x15 )
x12 = x15
x13 = x15
x16 = x19
x17 = x16
x19 = ( ( ( ( ( x10 OR x11 ) OR x3 ) OR x1 ) AND x18 ) OR ( x18 AND x14 ) ) \\
MIR-9-NEUROGENESIS & 6 & 0 & 6 & x1: v\_Neural\_Precursor, x2: v\_Progenitor, x3: v\_elavl3\_HuC, x4: v\_her6, x5: v\_miR\_9, x6: v\_zic5 & x1 = x3
x2 = ( ( NOT x4 AND x6 ) OR x4 )
x3 = ( NOT x5 AND NOT x2 )
x4 = ( NOT x5 AND NOT x1 )
x5 = ( NOT x4 AND NOT x1 )
x6 = ( NOT x5 AND NOT x1 ) \\
DROSOPHILA-JAK-STAT-PATHWAY & 19 & 12 & 7 & x1: v\_Brwd3, x2: v\_Dome, x3: v\_ET, x4: v\_Hop\_b1, x5: v\_Hop\_b2, x6: v\_Hrs, x7: v\_Ken, x8: v\_NStat92E, x9: v\_OS, x10: v\_Ptp61F, x11: v\_Socs36E, x12: v\_Socs44A, x13: v\_Stam, x14: v\_Stat92E\_b1, x15: v\_Stat92E\_b2, x16: v\_Su\_var, x17: v\_Targets, x18: v\_Upd2, x19: v\_Upd3 & x2 = ( ( ( ( NOT x9 AND NOT x18 ) AND x19 ) OR ( NOT x9 AND x18 ) ) OR x9 )
x4 = ( ( ( ( ( ( ( ( NOT x2 AND x4 ) AND x5 ) OR ( ( ( x2 AND NOT x3 ) AND NOT x6 ) AND NOT x11 ) ) OR ( ( ( ( ( x2 AND NOT x3 ) AND NOT x6 ) AND x11 ) AND x4 ) AND x5 ) ) OR ( ( ( ( x2 AND NOT x3 ) AND x6 ) AND NOT x13 ) AND NOT x11 ) ) OR ( ( ( ( ( ( x2 AND NOT x3 ) AND x6 ) AND NOT x13 ) AND x11 ) AND x4 ) AND x5 ) ) OR ( ( ( x2 AND NOT x3 ) AND x6 ) AND x13 ) ) OR ( ( ( x2 AND x3 ) AND x4 ) AND x5 ) )
x5 = ( ( ( ( ( x2 AND NOT x3 ) AND x6 ) AND x13 ) AND NOT x11 ) AND x4 )
x11 = ( x14 AND x15 )
x14 = ( ( ( ( ( ( ( ( NOT x4 AND x14 ) AND x15 ) OR ( ( ( ( ( x4 AND NOT x12 ) AND NOT x10 ) AND NOT x1 ) AND NOT x7 ) AND NOT x16 ) ) OR ( ( ( ( ( ( ( x4 AND NOT x12 ) AND NOT x10 ) AND NOT x1 ) AND NOT x7 ) AND x16 ) AND x14 ) AND x15 ) ) OR ( ( ( ( ( ( x4 AND NOT x12 ) AND NOT x10 ) AND NOT x1 ) AND x7 ) AND x14 ) AND x15 ) ) OR ( ( ( ( ( x4 AND NOT x12 ) AND NOT x10 ) AND x1 ) AND x14 ) AND x15 ) ) OR ( ( ( ( x4 AND NOT x12 ) AND x10 ) AND x14 ) AND x15 ) ) OR ( ( ( x4 AND x12 ) AND x14 ) AND x15 ) )
x15 = ( ( ( ( ( ( ( x4 AND x5 ) AND NOT x12 ) AND NOT x10 ) AND NOT x1 ) AND NOT x7 ) AND NOT x16 ) AND x14 )
x17 = ( x14 AND NOT x8 ) \\
TUMOUR-CELL-INVASION-AND-MIGRATION-REDUCED & 20 & 2 & 18 & x1: v\_AKT1, x2: v\_AKT2, x3: v\_Apoptosis, x4: v\_CCA, x5: v\_DNAdamage, x6: v\_ECMicroenv, x7: v\_EMT, x8: v\_EMTreg, x9: v\_ERK\_pthw, x10: v\_Ecadh, x11: v\_GF, x12: v\_Invasion, x13: v\_Metastasis, x14: v\_Migration, x15: v\_Notch\_pthw, x16: v\_TGFb\_pthw, x17: v\_WNT\_pthw, x18: v\_miRNA, x19: v\_p53, x20: v\_p63\_73 & x1 = ( ( ( ( ( ( ( ( ( ( NOT x11 AND NOT x16 ) AND NOT x15 ) AND x17 ) AND NOT x19 ) AND x8 ) AND NOT x18 ) AND NOT x10 ) OR ( ( ( ( ( ( NOT x11 AND NOT x16 ) AND x15 ) AND x17 ) AND NOT x19 ) AND NOT x18 ) AND NOT x10 ) ) OR ( ( ( ( ( NOT x11 AND x16 ) AND x17 ) AND NOT x19 ) AND NOT x18 ) AND NOT x10 ) ) OR ( ( ( ( x11 AND x17 ) AND NOT x19 ) AND NOT x18 ) AND NOT x10 ) )
x2 = ( ( NOT x19 AND x8 ) AND NOT x18 )
x3 = ( ( ( ( ( ( ( NOT x19 AND NOT x8 ) AND NOT x20 ) AND NOT x1 ) AND NOT x9 ) AND x18 ) OR ( ( ( ( NOT x19 AND NOT x8 ) AND x20 ) AND NOT x1 ) AND NOT x9 ) ) OR ( ( ( x19 AND NOT x8 ) AND NOT x1 ) AND NOT x9 ) )
x4 = ( ( ( ( ( ( ( ( ( ( ( ( ( ( ( ( ( ( ( ( ( ( ( ( ( ( NOT x16 AND NOT x19 ) AND NOT x8 ) AND NOT x20 ) AND NOT x1 ) AND NOT x2 ) AND x18 ) OR ( ( ( ( ( ( NOT x16 AND NOT x19 ) AND NOT x8 ) AND NOT x20 ) AND NOT x1 ) AND x2 ) AND NOT x9 ) ) OR ( ( ( ( ( ( ( NOT x16 AND NOT x19 ) AND NOT x8 ) AND NOT x20 ) AND NOT x1 ) AND x2 ) AND x9 ) AND x18 ) ) OR ( ( ( ( ( NOT x16 AND NOT x19 ) AND NOT x8 ) AND x20 ) AND NOT x1 ) AND NOT x9 ) ) OR ( ( ( ( ( ( NOT x16 AND NOT x19 ) AND NOT x8 ) AND x20 ) AND NOT x1 ) AND x9 ) AND x18 ) ) OR ( ( ( NOT x16 AND NOT x19 ) AND x8 ) AND NOT x1 ) ) OR ( ( ( ( NOT x16 AND x19 ) AND NOT x8 ) AND NOT x1 ) AND NOT x9 ) ) OR ( ( ( ( ( NOT x16 AND x19 ) AND NOT x8 ) AND NOT x1 ) AND x9 ) AND x18 ) ) OR ( ( ( NOT x16 AND x19 ) AND x8 ) AND NOT x1 ) ) OR ( ( ( ( ( ( ( x16 AND NOT x15 ) AND NOT x19 ) AND NOT x8 ) AND NOT x20 ) AND NOT x1 ) AND NOT x2 ) AND x18 ) ) OR ( ( ( ( ( ( ( x16 AND NOT x15 ) AND NOT x19 ) AND NOT x8 ) AND NOT x20 ) AND NOT x1 ) AND x2 ) AND NOT x9 ) ) OR ( ( ( ( ( ( ( ( x16 AND NOT x15 ) AND NOT x19 ) AND NOT x8 ) AND NOT x20 ) AND NOT x1 ) AND x2 ) AND x9 ) AND x18 ) ) OR ( ( ( ( ( ( x16 AND NOT x15 ) AND NOT x19 ) AND NOT x8 ) AND x20 ) AND NOT x1 ) AND NOT x9 ) ) OR ( ( ( ( ( ( ( x16 AND NOT x15 ) AND NOT x19 ) AND NOT x8 ) AND x20 ) AND NOT x1 ) AND x9 ) AND x18 ) ) OR ( ( ( ( x16 AND NOT x15 ) AND NOT x19 ) AND x8 ) AND NOT x1 ) ) OR ( ( ( ( ( x16 AND NOT x15 ) AND x19 ) AND NOT x8 ) AND NOT x1 ) AND NOT x9 ) ) OR ( ( ( ( ( ( x16 AND NOT x15 ) AND x19 ) AND NOT x8 ) AND NOT x1 ) AND x9 ) AND x18 ) ) OR ( ( ( ( x16 AND NOT x15 ) AND x19 ) AND x8 ) AND NOT x1 ) ) OR ( ( ( ( x16 AND x15 ) AND NOT x8 ) AND NOT x1 ) AND NOT x9 ) ) OR ( ( ( ( ( x16 AND x15 ) AND NOT x8 ) AND NOT x1 ) AND x9 ) AND x18 ) ) OR ( ( ( x16 AND x15 ) AND x8 ) AND NOT x1 ) )
x7 = ( x8 AND NOT x10 )
x8 = ( ( ( ( ( ( NOT x15 AND NOT x17 ) AND NOT x19 ) AND x8 ) AND NOT x18 ) OR ( ( ( NOT x15 AND x17 ) AND NOT x19 ) AND NOT x18 ) ) OR ( ( x15 AND NOT x19 ) AND NOT x18 ) )
x9 = ( ( ( ( ( ( ( NOT x11 AND NOT x16 ) AND NOT x15 ) AND x8 ) AND NOT x1 ) OR ( ( ( NOT x11 AND NOT x16 ) AND x15 ) AND NOT x1 ) ) OR ( ( NOT x11 AND x16 ) AND NOT x1 ) ) OR ( x11 AND NOT x1 ) )
x10 = ( NOT x8 AND NOT x2 )
x11 = ( ( ( NOT x11 AND x8 ) AND NOT x10 ) OR ( x11 AND NOT x10 ) )
x12 = ( ( ( NOT x16 AND x17 ) OR ( ( x16 AND NOT x17 ) AND x8 ) ) OR ( x16 AND x17 ) )
x13 = x14
x14 = ( ( ( ( ( ( x12 AND x7 ) AND NOT x20 ) AND NOT x1 ) AND x2 ) AND x9 ) AND NOT x18 )
x15 = ( ( ( x6 AND NOT x19 ) AND NOT x20 ) AND NOT x18 )
x16 = ( ( ( ( NOT x6 AND x15 ) AND NOT x17 ) AND NOT x18 ) OR ( ( x6 AND NOT x17 ) AND NOT x18 ) )
x17 = ( ( ( ( ( ( ( NOT x15 AND NOT x17 ) AND NOT x19 ) AND NOT x8 ) AND NOT x20 ) AND NOT x1 ) AND NOT x18 ) AND NOT x10 )
x18 = ( ( ( ( ( NOT x19 AND NOT x8 ) AND x20 ) AND NOT x1 ) AND NOT x2 ) OR ( ( ( x19 AND NOT x8 ) AND NOT x1 ) AND NOT x2 ) )
x19 = ( ( ( ( ( ( ( ( NOT x5 AND NOT x15 ) AND x17 ) AND NOT x8 ) AND NOT x20 ) AND NOT x1 ) AND NOT x2 ) OR ( ( ( ( ( NOT x5 AND x15 ) AND NOT x8 ) AND NOT x20 ) AND NOT x1 ) AND NOT x2 ) ) OR ( ( ( ( x5 AND NOT x8 ) AND NOT x20 ) AND NOT x1 ) AND NOT x2 ) )
x20 = ( ( ( ( ( x5 AND NOT x15 ) AND NOT x19 ) AND NOT x8 ) AND NOT x1 ) AND NOT x2 ) \\
P53-MDM2-NETWORK & 6 & 1 & 5 & x1: v\_DNAdam, x2: v\_Mdm2cyt\_b1, x3: v\_Mdm2cyt\_b2, x4: v\_Mdm2nuc, x5: v\_p53\_b1, x6: v\_p53\_b2 & x1 = ( ( NOT x5 AND x1 ) OR ( ( x5 AND NOT x6 ) AND x1 ) )
x3 = ( ( x5 AND x6 ) AND x2 )
x4 = ( ( ( ( ( NOT x5 AND x2 ) AND NOT x3 ) AND NOT x1 ) OR ( ( NOT x5 AND x2 ) AND x3 ) ) OR ( ( x5 AND x2 ) AND x3 ) )
x5 = ( ( ( NOT x5 AND NOT x4 ) OR ( ( x5 AND NOT x6 ) AND NOT x4 ) ) OR ( x5 AND x6 ) )
x6 = ( x5 AND NOT x4 ) \\
DROSOPHILA-GAP-A & 7 & 2 & 5 & x1: v\_Gt, x2: v\_Hb\_b1, x3: v\_Hb\_b2, x4: v\_Hb\_b3, x5: v\_Kni, x6: v\_Kr\_b1, x7: v\_Kr\_b2 & x1 = NOT x6
x3 = x2
x4 = ( x2 AND x3 )
x6 = ( ( ( ( ( ( ( ( ( ( ( ( ( ( NOT x1 AND NOT x2 ) AND x6 ) AND x7 ) OR ( ( NOT x1 AND x2 ) AND NOT x3 ) ) OR ( ( ( NOT x1 AND x2 ) AND x3 ) AND NOT x4 ) ) OR ( ( ( ( ( NOT x1 AND x2 ) AND x3 ) AND x4 ) AND x6 ) AND x7 ) ) OR ( ( ( x1 AND NOT x2 ) AND x6 ) AND x7 ) ) OR ( ( ( ( x1 AND x2 ) AND NOT x3 ) AND NOT x6 ) AND NOT x5 ) ) OR ( ( ( ( ( x1 AND x2 ) AND NOT x3 ) AND x6 ) AND NOT x7 ) AND NOT x5 ) ) OR ( ( ( ( x1 AND x2 ) AND NOT x3 ) AND x6 ) AND x7 ) ) OR ( ( ( ( ( x1 AND x2 ) AND x3 ) AND NOT x4 ) AND NOT x6 ) AND NOT x5 ) ) OR ( ( ( ( ( ( x1 AND x2 ) AND x3 ) AND NOT x4 ) AND x6 ) AND NOT x7 ) AND NOT x5 ) ) OR ( ( ( ( ( x1 AND x2 ) AND x3 ) AND NOT x4 ) AND x6 ) AND x7 ) ) OR ( ( ( ( ( x1 AND x2 ) AND x3 ) AND x4 ) AND x6 ) AND x7 ) )
x7 = ( ( ( ( ( NOT x1 AND x2 ) AND NOT x3 ) AND x6 ) AND NOT x5 ) OR ( ( ( ( ( NOT x1 AND x2 ) AND x3 ) AND NOT x4 ) AND x6 ) AND NOT x5 ) ) \\
TOLL-PATHWAY-OF-DROSOPHILA & 11 & 2 & 9 & x1: v\_Cactus, x2: v\_Dif, x3: v\_Dorsal, x4: v\_MyD88, x5: v\_Nec, x6: v\_Pelle, x7: v\_Slmb, x8: v\_Spz, x9: v\_Targets, x10: v\_Toll, x11: v\_Tube & x1 = NOT ( x6 AND x7 )
x2 = NOT x1
x3 = NOT x1
x4 = x10
x6 = x11
x8 = NOT x5
x9 = ( x3 OR x2 )
x10 = x8
x11 = x4 \\
SEGMENT-POLARITY-1-CELL & 19 & 2 & 17 & x1: v\_Ci1, x2: v\_Ciact\_b1, x3: v\_Ciact\_b2, x4: v\_Cirep, x5: v\_Dsh, x6: v\_En, x7: v\_Fz, x8: v\_Hh, x9: v\_Hh\_ext, x10: v\_Nkd\_b1, x11: v\_Nkd\_b2, x12: v\_Pka\_b1, x13: v\_Pka\_b2, x14: v\_Ptc\_b1, x15: v\_Ptc\_b2, x16: v\_Slp, x17: v\_Wg\_b1, x18: v\_Wg\_b2, x19: v\_Wg\_ext & x1 = NOT x6
x2 = ( ( ( ( ( ( ( ( NOT x5 AND NOT x1 ) AND x2 ) AND x3 ) OR ( ( ( NOT x5 AND x1 ) AND NOT x2 ) AND NOT x12 ) ) OR ( ( ( ( NOT x5 AND x1 ) AND x2 ) AND NOT x3 ) AND NOT x12 ) ) OR ( ( ( NOT x5 AND x1 ) AND x2 ) AND x3 ) ) OR ( ( ( x5 AND NOT x1 ) AND x2 ) AND x3 ) ) OR ( x5 AND x1 ) )
x3 = ( ( ( x5 AND x1 ) AND x2 ) AND NOT x12 )
x4 = ( ( ( NOT x5 AND x1 ) AND x12 ) AND x13 )
x5 = x7
x6 = ( x5 AND NOT x16 )
x7 = ( ( NOT x17 AND x19 ) OR x17 )
x8 = ( x6 AND NOT x4 )
x10 = ( ( ( NOT x10 AND NOT x6 ) OR ( ( x10 AND NOT x11 ) AND NOT x6 ) ) OR ( x10 AND x11 ) )
x11 = ( ( x5 AND x10 ) AND NOT x6 )
x12 = ( ( ( NOT x12 AND x14 ) OR ( ( x12 AND NOT x13 ) AND x14 ) ) OR ( x12 AND x13 ) )
x13 = ( x12 AND x14 )
x14 = ( ( ( ( ( NOT x6 AND NOT x14 ) AND NOT x9 ) OR ( ( ( NOT x6 AND x14 ) AND NOT x15 ) AND NOT x9 ) ) OR ( ( NOT x6 AND x14 ) AND x15 ) ) OR ( ( x6 AND x14 ) AND x15 ) )
x15 = ( ( ( NOT x6 AND x2 ) AND x14 ) AND NOT x9 )
x16 = ( x5 AND NOT x6 )
x17 = ( ( ( ( ( ( ( ( ( ( NOT x17 AND x16 ) AND NOT x10 ) AND NOT x6 ) AND x2 ) OR ( ( ( ( ( NOT x17 AND x16 ) AND x10 ) AND NOT x11 ) AND NOT x6 ) AND x2 ) ) OR ( ( ( ( ( ( NOT x17 AND x16 ) AND x10 ) AND x11 ) AND NOT x6 ) AND x2 ) AND x3 ) ) OR ( ( ( ( ( x17 AND NOT x18 ) AND x16 ) AND NOT x10 ) AND NOT x6 ) AND x2 ) ) OR ( ( ( ( ( ( x17 AND NOT x18 ) AND x16 ) AND x10 ) AND NOT x11 ) AND NOT x6 ) AND x2 ) ) OR ( ( ( ( ( ( ( x17 AND NOT x18 ) AND x16 ) AND x10 ) AND x11 ) AND NOT x6 ) AND x2 ) AND x3 ) ) OR ( x17 AND x18 ) )
x18 = ( ( ( ( x17 AND x16 ) AND NOT x6 ) AND x2 ) AND x3 ) \\
BT474-BREAST-CELL-LINE-SHORT-TERM & 16 & 5 & 11 & x1: v\_AKT, x2: v\_EGF, x3: v\_ERBB1, x4: v\_ERBB2, x5: v\_ERBB3, x6: v\_ERK1\_2, x7: v\_HRG, x8: v\_MEK1\_2, x9: v\_PDK1, x10: v\_PKCa, x11: v\_PLCg, x12: v\_erlotinib, x13: v\_mTOR, x14: v\_p70S6K, x15: v\_pertuzumab, x16: v\_trastuzumab & x1 = ( ( ( x5 OR x9 ) OR x13 ) OR x1 )
x3 = ( ( ( x3 AND NOT ( x12 OR x15 ) ) OR ( x2 AND NOT ( x12 OR x15 ) ) ) OR ( x11 AND NOT ( x12 OR x15 ) ) )
x4 = ( ( ( x5 AND NOT ( ( x12 OR x16 ) OR x15 ) ) OR ( x4 AND NOT ( ( x12 OR x16 ) OR x15 ) ) ) OR ( x2 AND NOT ( ( x12 OR x16 ) OR x15 ) ) )
x5 = ( ( x7 AND NOT ( ( x15 OR x15 ) OR x12 ) ) OR ( x5 AND NOT ( ( x15 OR x15 ) OR x12 ) ) )
x6 = ( ( ( x8 OR x6 ) OR x15 ) OR x2 )
x8 = ( ( ( x5 OR x3 ) OR x8 ) OR x4 )
x9 = ( ( ( ( x3 OR x9 ) OR x5 ) OR x8 ) OR x4 )
x10 = ( x11 OR x10 )
x11 = ( ( ( ( x3 OR x11 ) OR x4 ) OR x5 ) OR x2 )
x13 = ( ( x1 OR x13 ) OR x15 )
x14 = ( ( ( x14 OR x1 ) OR x6 ) OR x13 ) \\
PAIR-RULE-MODULE & 11 & 0 & 11 & x1: v\_Eve\_b1, x2: v\_Eve\_b2, x3: v\_Eve\_b3, x4: v\_Ftz\_b1, x5: v\_Ftz\_b2, x6: v\_Odd, x7: v\_Ppa, x8: v\_Prd\_b1, x9: v\_Prd\_b2, x10: v\_Run, x11: v\_Slp & x1 = ( ( ( ( ( ( NOT x1 AND x8 ) AND NOT x11 ) AND NOT x6 ) OR ( ( ( x1 AND NOT x2 ) AND NOT x10 ) AND NOT x11 ) ) OR ( ( ( ( x1 AND NOT x2 ) AND x10 ) AND NOT x11 ) AND NOT x6 ) ) OR ( x1 AND x2 ) )
x2 = ( ( ( ( ( ( ( x1 AND NOT x2 ) AND x8 ) AND NOT x10 ) AND NOT x11 ) AND NOT x6 ) OR ( ( ( ( ( ( x1 AND x2 ) AND NOT x3 ) AND x8 ) AND NOT x10 ) AND NOT x11 ) AND NOT x6 ) ) OR ( ( x1 AND x2 ) AND x3 ) )
x3 = ( ( ( ( ( x1 AND x2 ) AND x8 ) AND NOT x10 ) AND NOT x11 ) AND NOT x6 )
x4 = ( ( ( ( ( ( ( ( ( ( ( NOT x1 AND NOT x11 ) AND NOT x4 ) AND NOT x6 ) OR ( ( ( ( NOT x1 AND NOT x11 ) AND x4 ) AND NOT x5 ) AND NOT x6 ) ) OR ( ( ( NOT x1 AND NOT x11 ) AND x4 ) AND x5 ) ) OR ( ( ( NOT x1 AND x11 ) AND x4 ) AND x5 ) ) OR ( ( ( ( x1 AND NOT x2 ) AND NOT x11 ) AND NOT x4 ) AND NOT x6 ) ) OR ( ( ( ( ( x1 AND NOT x2 ) AND NOT x11 ) AND x4 ) AND NOT x5 ) AND NOT x6 ) ) OR ( ( ( ( x1 AND NOT x2 ) AND NOT x11 ) AND x4 ) AND x5 ) ) OR ( ( ( ( x1 AND NOT x2 ) AND x11 ) AND x4 ) AND x5 ) ) OR ( ( ( x1 AND x2 ) AND x4 ) AND x5 ) )
x5 = ( ( ( ( NOT x1 AND NOT x11 ) AND x4 ) AND NOT x6 ) OR ( ( ( ( x1 AND NOT x2 ) AND NOT x11 ) AND x4 ) AND NOT x6 ) )
x6 = ( NOT x1 AND NOT x8 )
x7 = ( NOT x1 OR ( x1 AND NOT x2 ) )
x8 = ( ( ( NOT x8 AND NOT x6 ) OR ( ( x8 AND NOT x9 ) AND NOT x6 ) ) OR ( x8 AND x9 ) )
x9 = ( ( x8 AND NOT x7 ) AND NOT x6 )
x10 = ( ( ( NOT x1 AND x8 ) AND NOT x6 ) OR ( ( ( x1 AND NOT x2 ) AND x8 ) AND NOT x6 ) )
x11 = ( ( ( NOT x1 AND NOT x4 ) AND NOT x6 ) OR ( ( ( x1 AND NOT x2 ) AND NOT x4 ) AND NOT x6 ) ) \\
BUDDING-YEAST-CELL-CYCLE & 20 & 4 & 16 & x1: v\_BuddingCP, x2: v\_Cdc14, x3: v\_Cdc20, x4: v\_Cdh1, x5: v\_Clb2, x6: v\_Clb5, x7: v\_Cln2, x8: v\_Cln3, x9: v\_FEAR, x10: v\_MEN, x11: v\_SFF, x12: v\_SMBF, x13: v\_Sic1, x14: v\_Size, x15: v\_SpindleCP, x16: v\_Start, x17: v\_Swe1, x18: v\_Swi5, x19: v\_Whi5, x20: v\_Yhp1 & x2 = ( x10 AND x9 )
x3 = ( x15 AND ( x5 AND x11 ) )
x4 = ( x2 OR NOT ( ( ( x6 OR x2 ) OR x5 ) OR x7 ) )
x5 = ( ( x11 AND NOT ( ( ( x4 AND x3 ) OR ( x3 AND x4 ) ) OR x17 ) ) OR NOT ( ( ( ( x17 OR x11 ) OR x4 ) OR x3 ) OR x13 ) )
x6 = ( x12 AND NOT ( x13 OR x3 ) )
x7 = ( x12 AND x16 )
x8 = ( x14 AND NOT x20 )
x9 = x3
x10 = ( x9 AND x5 )
x11 = x5
x12 = ( NOT ( x5 OR x19 ) OR NOT ( x19 OR x5 ) )
x13 = ( ( ( x18 AND NOT ( ( ( x6 AND NOT x2 ) OR ( x5 AND NOT x2 ) ) OR ( x7 AND NOT x2 ) ) ) OR ( x13 AND NOT ( ( ( x6 AND NOT x2 ) OR ( x5 AND NOT x2 ) ) OR ( x7 AND NOT x2 ) ) ) ) OR NOT ( ( ( ( ( x18 OR x6 ) OR x2 ) OR x5 ) OR x7 ) OR x13 ) )
x17 = ( NOT x1 OR NOT x1 )
x18 = ( ( x2 AND ( x11 AND NOT x18 ) ) AND NOT x5 )
x19 = ( NOT ( ( x7 AND x16 ) OR ( x8 AND x16 ) ) OR NOT ( ( x16 OR x8 ) OR x7 ) )
x20 = x12 \\
AGS-CELL-FATE-DECISION-REDUCED & 14 & 2 & 12 & x1: v\_AKT, x2: v\_Antisurvival\_b1, x3: v\_Antisurvival\_b2, x4: v\_Antisurvival\_b3, x5: v\_ERK, x6: v\_GSK3, x7: v\_MEK, x8: v\_PI3K, x9: v\_Prosurvival\_b1, x10: v\_Prosurvival\_b2, x11: v\_Prosurvival\_b3, x12: v\_TAK1, x13: v\_betacatenin, x14: v\_p38alpha & x1 = ( ( ( ( ( ( ( ( ( ( ( NOT x5 AND NOT x12 ) AND NOT x1 ) AND NOT x8 ) AND x6 ) OR ( ( ( NOT x5 AND NOT x12 ) AND NOT x1 ) AND x8 ) ) OR ( ( ( NOT x5 AND NOT x12 ) AND x1 ) AND x8 ) ) OR ( ( ( ( NOT x5 AND x12 ) AND x8 ) AND NOT x6 ) AND x13 ) ) OR ( ( ( NOT x5 AND x12 ) AND x8 ) AND x6 ) ) OR ( ( x5 AND NOT x12 ) AND x8 ) ) OR ( ( ( ( x5 AND x12 ) AND x8 ) AND NOT x6 ) AND x13 ) ) OR ( ( ( x5 AND x12 ) AND x8 ) AND x6 ) )
x2 = ( ( ( ( ( NOT x5 AND NOT x14 ) OR ( ( NOT x5 AND x14 ) AND NOT x1 ) ) OR ( ( ( ( NOT x5 AND x14 ) AND x1 ) AND x2 ) AND x3 ) ) OR ( x5 AND NOT x1 ) ) OR ( ( ( x5 AND x1 ) AND x2 ) AND x3 ) )
x3 = ( ( ( ( ( ( ( ( ( ( ( ( ( NOT x5 AND NOT x12 ) AND NOT x1 ) AND x2 ) OR ( ( ( ( ( NOT x5 AND NOT x12 ) AND x1 ) AND x2 ) AND x3 ) AND x4 ) ) OR ( ( ( ( ( NOT x5 AND x12 ) AND NOT x14 ) AND x2 ) AND x3 ) AND x4 ) ) OR ( ( ( ( ( ( ( NOT x5 AND x12 ) AND x14 ) AND NOT x1 ) AND NOT x8 ) AND x2 ) AND x3 ) AND x4 ) ) OR ( ( ( ( ( ( ( ( ( NOT x5 AND x12 ) AND x14 ) AND NOT x1 ) AND x8 ) AND NOT x6 ) AND NOT x13 ) AND x2 ) AND x3 ) AND x4 ) ) OR ( ( ( ( ( ( ( NOT x5 AND x12 ) AND x14 ) AND NOT x1 ) AND x8 ) AND NOT x6 ) AND x13 ) AND x2 ) ) OR ( ( ( ( ( ( NOT x5 AND x12 ) AND x14 ) AND NOT x1 ) AND x8 ) AND x6 ) AND x2 ) ) OR ( ( ( ( ( ( NOT x5 AND x12 ) AND x14 ) AND x1 ) AND x2 ) AND x3 ) AND x4 ) ) OR ( ( ( x5 AND NOT x12 ) AND NOT x1 ) AND x2 ) ) OR ( ( ( ( ( x5 AND NOT x12 ) AND x1 ) AND x2 ) AND x3 ) AND x4 ) ) OR ( ( ( ( x5 AND x12 ) AND x2 ) AND x3 ) AND x4 ) )
x4 = ( ( ( ( ( ( NOT x5 AND NOT x12 ) AND x14 ) AND NOT x1 ) AND x8 ) AND x2 ) AND x3 )
x5 = ( ( ( NOT x7 AND NOT x5 ) AND NOT x1 ) OR x7 )
x7 = ( ( ( ( ( NOT x5 OR ( x5 AND NOT x12 ) ) OR ( ( x5 AND x12 ) AND NOT x14 ) ) OR ( ( ( x5 AND x12 ) AND x14 ) AND NOT x1 ) ) OR ( ( ( ( ( x5 AND x12 ) AND x14 ) AND x1 ) AND NOT x6 ) AND x13 ) ) OR ( ( ( ( x5 AND x12 ) AND x14 ) AND x1 ) AND x6 ) )
x8 = ( ( ( NOT x5 OR ( x5 AND NOT x12 ) ) OR ( ( ( x5 AND x12 ) AND NOT x6 ) AND x13 ) ) OR ( ( x5 AND x12 ) AND x6 ) )
x9 = ( ( ( ( ( ( ( ( ( NOT x5 AND NOT x12 ) OR ( ( ( ( NOT x5 AND x12 ) AND NOT x13 ) AND x9 ) AND x10 ) ) OR ( ( NOT x5 AND x12 ) AND x13 ) ) OR ( x5 AND NOT x12 ) ) OR ( ( ( ( ( x5 AND x12 ) AND NOT x8 ) AND NOT x13 ) AND x9 ) AND x10 ) ) OR ( ( ( x5 AND x12 ) AND NOT x8 ) AND x13 ) ) OR ( ( ( ( ( ( x5 AND x12 ) AND x8 ) AND NOT x6 ) AND NOT x13 ) AND x9 ) AND x10 ) ) OR ( ( ( ( x5 AND x12 ) AND x8 ) AND NOT x6 ) AND x13 ) ) OR ( ( ( x5 AND x12 ) AND x8 ) AND x6 ) )
x10 = ( ( ( NOT x12 AND x9 ) OR ( ( ( ( x12 AND NOT x13 ) AND x9 ) AND x10 ) AND x11 ) ) OR ( ( x12 AND x13 ) AND x9 ) )
x11 = ( ( ( ( ( x5 AND NOT x12 ) AND x8 ) AND x9 ) AND x10 ) OR ( ( ( ( ( x5 AND x12 ) AND x8 ) AND x13 ) AND x9 ) AND x10 ) )
x12 = NOT x14
x14 = ( NOT x5 AND NOT x14 ) \\
HEMATOPOIESIS-AGING & 15 & 0 & 15 & x1: v\_Bclaf1, x2: v\_CDK46CycD, x3: v\_CIPKIP, x4: v\_Cebpa, x5: v\_Egr1, x6: v\_Fli1, x7: v\_Gata1, x8: v\_Gata2, x9: v\_Ikzf1, x10: v\_Junb, x11: v\_Klf1, x12: v\_Myc, x13: v\_Spi1, x14: v\_Tal1, x15: v\_Zfpm1 & x1 = x12
x2 = ( x1 OR x12 )
x3 = x10
x4 = ( ( x8 AND NOT x9 ) OR ( x13 AND NOT x9 ) )
x5 = ( x8 AND x10 )
x6 = ( x10 OR ( x7 AND NOT x11 ) )
x7 = ( x6 OR ( ( x8 AND NOT x13 ) OR ( x7 AND ( NOT x9 AND NOT x13 ) ) ) )
x8 = ( ( x8 AND ( NOT x7 AND NOT x15 ) ) OR ( x5 AND ( NOT x7 AND ( NOT x15 AND NOT x13 ) ) ) )
x9 = x8
x10 = ( x5 OR x12 )
x11 = ( x7 AND NOT x6 )
x12 = ( x4 AND x1 )
x13 = ( ( x13 AND NOT x7 ) OR ( x4 AND ( NOT x7 AND NOT x8 ) ) )
x14 = ( x7 AND NOT x13 )
x15 = x7 \\
BOOLEAN-CELL-CYCLE & 14 & 2 & 12 & x1: v\_Cdc20, x2: v\_Cdh1, x3: v\_CycA, x4: v\_CycB, x5: v\_CycD, x6: v\_CycE, x7: v\_E2F, x8: v\_Rb1, x9: v\_Rb2, x10: v\_Skp2, x11: v\_UbcH10, x12: v\_p27\_1\_b1, x13: v\_p27\_1\_b2, x14: v\_p27\_2 & x1 = x4
x2 = ( ( ( ( NOT x3 AND NOT x4 ) OR ( ( NOT x3 AND x4 ) AND x12 ) ) OR ( ( x3 AND x12 ) AND NOT x10 ) ) OR ( ( ( x3 AND x12 ) AND x10 ) AND x14 ) )
x3 = ( ( ( ( ( ( ( ( ( ( ( NOT x7 AND x3 ) AND NOT x1 ) AND NOT x2 ) OR ( ( ( ( NOT x7 AND x3 ) AND NOT x1 ) AND x2 ) AND NOT x11 ) ) OR ( ( ( NOT x7 AND x3 ) AND x1 ) AND NOT x11 ) ) OR ( ( ( ( x7 AND NOT x3 ) AND NOT x1 ) AND NOT x2 ) AND NOT x8 ) ) OR ( ( ( ( ( x7 AND NOT x3 ) AND NOT x1 ) AND x2 ) AND NOT x11 ) AND NOT x8 ) ) OR ( ( ( ( x7 AND NOT x3 ) AND x1 ) AND NOT x11 ) AND NOT x8 ) ) OR ( ( ( x7 AND x3 ) AND NOT x1 ) AND NOT x2 ) ) OR ( ( ( ( x7 AND x3 ) AND NOT x1 ) AND x2 ) AND NOT x11 ) ) OR ( ( ( x7 AND x3 ) AND x1 ) AND NOT x11 ) )
x4 = ( ( NOT x1 AND NOT x2 ) OR ( ( x1 AND NOT x2 ) AND NOT x11 ) )
x6 = ( ( NOT x9 AND x7 ) OR ( ( x9 AND x7 ) AND NOT x8 ) )
x7 = ( ( ( ( ( ( ( ( ( ( ( ( ( NOT x9 AND NOT x3 ) AND NOT x4 ) OR ( ( ( NOT x9 AND NOT x3 ) AND x4 ) AND NOT x1 ) ) OR ( ( ( NOT x9 AND x3 ) AND NOT x4 ) AND NOT x10 ) ) OR ( ( ( ( NOT x9 AND x3 ) AND NOT x4 ) AND x10 ) AND x14 ) ) OR ( ( ( ( NOT x9 AND x3 ) AND x4 ) AND NOT x1 ) AND NOT x10 ) ) OR ( ( ( ( ( NOT x9 AND x3 ) AND x4 ) AND NOT x1 ) AND x10 ) AND x14 ) ) OR ( ( ( x9 AND NOT x3 ) AND NOT x4 ) AND NOT x8 ) ) OR ( ( ( ( x9 AND NOT x3 ) AND x4 ) AND NOT x1 ) AND NOT x8 ) ) OR ( ( ( ( x9 AND x3 ) AND NOT x4 ) AND NOT x10 ) AND NOT x8 ) ) OR ( ( ( ( ( x9 AND x3 ) AND NOT x4 ) AND x10 ) AND NOT x8 ) AND x14 ) ) OR ( ( ( ( ( x9 AND x3 ) AND x4 ) AND NOT x1 ) AND NOT x10 ) AND NOT x8 ) ) OR ( ( ( ( ( ( x9 AND x3 ) AND x4 ) AND NOT x1 ) AND x10 ) AND NOT x8 ) AND x14 ) )
x8 = ( ( ( ( ( ( ( NOT x9 AND NOT x6 ) AND NOT x3 ) AND NOT x4 ) OR ( ( ( ( NOT x9 AND NOT x6 ) AND NOT x3 ) AND x4 ) AND x12 ) ) OR ( ( ( NOT x9 AND NOT x6 ) AND x3 ) AND x12 ) ) OR ( ( NOT x9 AND x6 ) AND x12 ) ) OR x9 )
x9 = ( ( ( ( ( ( ( ( NOT x5 AND NOT x6 ) AND NOT x3 ) AND NOT x4 ) AND x8 ) OR ( ( ( ( ( NOT x5 AND NOT x6 ) AND NOT x3 ) AND x4 ) AND x12 ) AND x8 ) ) OR ( ( ( ( NOT x5 AND NOT x6 ) AND x3 ) AND x12 ) AND x8 ) ) OR ( ( ( ( NOT x5 AND x6 ) AND NOT x3 ) AND x12 ) AND x8 ) ) OR ( ( ( ( ( NOT x5 AND x6 ) AND x3 ) AND NOT x4 ) AND x12 ) AND x8 ) )
x10 = ( ( NOT x9 OR ( x9 AND NOT x2 ) ) OR ( ( x9 AND x2 ) AND NOT x8 ) )
x11 = ( ( ( ( ( ( ( ( ( NOT x3 AND NOT x4 ) AND NOT x1 ) AND NOT x2 ) OR ( ( ( NOT x3 AND NOT x4 ) AND x1 ) AND NOT x2 ) ) OR ( ( ( ( NOT x3 AND NOT x4 ) AND x1 ) AND x2 ) AND x11 ) ) OR ( ( NOT x3 AND x4 ) AND NOT x2 ) ) OR ( ( ( NOT x3 AND x4 ) AND x2 ) AND x11 ) ) OR ( x3 AND NOT x2 ) ) OR ( ( x3 AND x2 ) AND x11 ) )
x12 = ( ( ( ( ( ( ( ( ( ( ( ( ( ( ( ( ( ( ( ( ( ( ( NOT x5 AND NOT x12 ) AND x14 ) OR ( ( ( NOT x5 AND x12 ) AND NOT x13 ) AND x14 ) ) OR ( ( NOT x5 AND x12 ) AND x13 ) ) OR ( ( ( x5 AND NOT x6 ) AND NOT x3 ) AND NOT x4 ) ) OR ( ( ( ( ( x5 AND NOT x6 ) AND NOT x3 ) AND x4 ) AND NOT x12 ) AND NOT x10 ) ) OR ( ( ( ( ( ( x5 AND NOT x6 ) AND NOT x3 ) AND x4 ) AND NOT x12 ) AND x10 ) AND x14 ) ) OR ( ( ( ( ( ( x5 AND NOT x6 ) AND NOT x3 ) AND x4 ) AND x12 ) AND NOT x13 ) AND NOT x10 ) ) OR ( ( ( ( ( ( ( x5 AND NOT x6 ) AND NOT x3 ) AND x4 ) AND x12 ) AND NOT x13 ) AND x10 ) AND x14 ) ) OR ( ( ( ( ( x5 AND NOT x6 ) AND NOT x3 ) AND x4 ) AND x12 ) AND x13 ) ) OR ( ( ( ( ( x5 AND NOT x6 ) AND x3 ) AND NOT x4 ) AND NOT x12 ) AND NOT x10 ) ) OR ( ( ( ( ( ( x5 AND NOT x6 ) AND x3 ) AND NOT x4 ) AND NOT x12 ) AND x10 ) AND x14 ) ) OR ( ( ( ( x5 AND NOT x6 ) AND x3 ) AND NOT x4 ) AND x12 ) ) OR ( ( ( ( ( x5 AND NOT x6 ) AND x3 ) AND x4 ) AND NOT x12 ) AND NOT x10 ) ) OR ( ( ( ( ( ( x5 AND NOT x6 ) AND x3 ) AND x4 ) AND NOT x12 ) AND x10 ) AND x14 ) ) OR ( ( ( ( ( ( x5 AND NOT x6 ) AND x3 ) AND x4 ) AND x12 ) AND NOT x13 ) AND NOT x10 ) ) OR ( ( ( ( ( ( ( x5 AND NOT x6 ) AND x3 ) AND x4 ) AND x12 ) AND NOT x13 ) AND x10 ) AND x14 ) ) OR ( ( ( ( ( x5 AND NOT x6 ) AND x3 ) AND x4 ) AND x12 ) AND x13 ) ) OR ( ( ( x5 AND x6 ) AND NOT x12 ) AND NOT x10 ) ) OR ( ( ( ( x5 AND x6 ) AND NOT x12 ) AND x10 ) AND x14 ) ) OR ( ( ( ( x5 AND x6 ) AND x12 ) AND NOT x13 ) AND NOT x10 ) ) OR ( ( ( ( ( x5 AND x6 ) AND x12 ) AND NOT x13 ) AND x10 ) AND x14 ) ) OR ( ( ( x5 AND x6 ) AND x12 ) AND x13 ) )
x14 = ( ( ( ( ( ( ( ( NOT x5 AND NOT x6 ) AND NOT x4 ) AND x12 ) OR ( ( ( ( NOT x5 AND NOT x6 ) AND x4 ) AND x12 ) AND NOT x10 ) ) OR ( ( ( ( ( NOT x5 AND x6 ) AND NOT x3 ) AND NOT x4 ) AND x12 ) AND NOT x10 ) ) OR ( ( ( ( ( ( NOT x5 AND x6 ) AND NOT x3 ) AND NOT x4 ) AND x12 ) AND x10 ) AND x14 ) ) OR ( ( ( ( ( NOT x5 AND x6 ) AND NOT x3 ) AND x4 ) AND x12 ) AND NOT x10 ) ) OR ( ( ( ( NOT x5 AND x6 ) AND x3 ) AND x12 ) AND NOT x10 ) ) \\
CELL-CYCLE-TRANSCRIPTION & 9 & 0 & 9 & x1: v\_ACE2, x2: v\_CLN3, x3: v\_HCM1, x4: v\_MBF, x5: v\_SBF, x6: v\_SFF, x7: v\_SWI5, x8: v\_YHP1, x9: v\_YOX1 & x1 = x6
x2 = ( ( x7 AND x1 ) AND NOT ( x9 OR x8 ) )
x3 = ( x4 AND x5 )
x4 = x2
x5 = ( ( x4 AND NOT ( x8 OR x9 ) ) OR ( x2 AND NOT ( x8 OR x9 ) ) )
x6 = ( x5 AND x3 )
x7 = x6
x8 = ( x5 OR x4 )
x9 = ( x4 AND x5 ) \\
ARABIDOPSIS-THALIANA-CELL-CYCLE & 14 & 0 & 14 & x1: v\_APC\_C, x2: v\_CDKB1\_1, x3: v\_CYCA2\_3, x4: v\_CYCB1\_1, x5: v\_CYCD3\_1, x6: v\_E2Fa, x7: v\_E2Fb, x8: v\_E2Fc, x9: v\_E2Fe, x10: v\_KRP1, x11: v\_MYB3R1\_4, x12: v\_MYB77, x13: v\_RBR, x14: v\_SCF & x1 = ( ( ( x12 AND NOT x9 ) OR ( x11 AND NOT x9 ) ) OR ( x6 AND NOT ( x9 OR x13 ) ) )
x2 = ( ( x12 OR ( ( x7 AND ( NOT x13 OR ( x5 AND NOT x10 ) ) ) AND NOT x8 ) ) OR x11 )
x3 = ( ( x11 AND NOT x1 ) OR ( x12 AND NOT x1 ) )
x4 = ( ( ( x11 AND NOT x1 ) OR ( ( x7 AND ( ( x5 AND NOT x10 ) OR NOT x13 ) ) AND NOT ( x1 OR x8 ) ) ) OR ( x12 AND NOT x1 ) )
x5 = NOT x14
x6 = ( ( ( ( x2 AND ( ( NOT x8 AND NOT x3 ) AND NOT x6 ) ) OR ( x3 AND ( ( NOT x8 AND NOT x2 ) AND NOT x6 ) ) ) OR ( x6 AND NOT ( x2 AND x3 ) ) ) OR NOT ( ( ( x8 OR x2 ) OR x3 ) OR x6 ) )
x7 = ( x6 AND NOT x13 )
x8 = ( ( x11 AND NOT ( ( x14 AND x5 ) AND NOT x10 ) ) OR ( x6 AND NOT ( x13 OR ( ( x14 AND x5 ) AND NOT x10 ) ) ) )
x9 = ( ( ( ( ( ( ( ( ( ( ( ( ( ( ( ( ( ( x7 AND ( NOT x13 OR ( NOT x10 AND x5 ) ) ) OR x12 ) OR ( x5 AND ( ( ( ( NOT x10 AND NOT x12 ) AND NOT x8 ) AND NOT x7 ) AND NOT x13 ) ) ) OR ( x13 AND ( ( ( ( NOT x10 AND NOT x12 ) AND NOT x8 ) AND NOT x5 ) AND NOT x7 ) ) ) OR ( ( x5 AND ( x7 AND x13 ) ) AND ( ( NOT x10 AND NOT x12 ) AND NOT x8 ) ) ) OR ( ( x5 AND ( x10 AND x7 ) ) AND ( ( NOT x12 AND NOT x8 ) AND NOT x13 ) ) ) OR ( ( x5 AND x10 ) AND ( ( ( NOT x12 AND NOT x8 ) AND NOT x7 ) AND NOT x13 ) ) ) OR ( x10 AND ( ( ( ( NOT x12 AND NOT x8 ) AND NOT x5 ) AND NOT x7 ) AND NOT x13 ) ) ) OR ( ( x13 AND x10 ) AND ( ( ( NOT x12 AND NOT x8 ) AND NOT x5 ) AND NOT x7 ) ) ) OR ( ( x5 AND x13 ) AND ( ( ( NOT x10 AND NOT x12 ) AND NOT x8 ) AND NOT x7 ) ) ) OR ( ( x7 AND ( x10 AND x13 ) ) AND ( ( NOT x12 AND NOT x8 ) AND NOT x5 ) ) ) OR ( ( x7 AND ( x10 AND x8 ) ) AND ( ( NOT x12 AND NOT x5 ) AND NOT x13 ) ) ) OR ( ( x5 AND ( ( x10 AND x7 ) AND x13 ) ) AND ( NOT x12 AND NOT x8 ) ) ) OR ( ( x7 AND x10 ) AND ( ( ( NOT x12 AND NOT x8 ) AND NOT x5 ) AND NOT x13 ) ) ) OR ( x7 AND ( ( ( ( NOT x10 AND NOT x12 ) AND NOT x8 ) AND NOT x5 ) AND NOT x13 ) ) ) OR ( ( x5 AND ( x10 AND x13 ) ) AND ( ( NOT x12 AND NOT x8 ) AND NOT x7 ) ) ) OR ( ( x7 AND x13 ) AND ( ( ( NOT x10 AND NOT x12 ) AND NOT x8 ) AND NOT x5 ) ) ) OR NOT ( ( ( ( ( x10 OR x12 ) OR x8 ) OR x5 ) OR x7 ) OR x13 ) )
x10 = ( ( x12 AND NOT ( x2 AND ( x3 AND x14 ) ) ) OR ( x11 AND NOT ( x2 AND ( x3 AND x14 ) ) ) )
x11 = ( x12 OR ( ( x11 AND x4 ) AND NOT x10 ) )
x12 = ( x7 AND ( ( x5 AND NOT x10 ) OR NOT x13 ) )
x13 = ( ( ( x6 AND ( x10 OR NOT x5 ) ) AND NOT ( x13 AND ( x10 OR NOT x5 ) ) ) OR ( x11 AND ( x10 OR NOT x5 ) ) )
x14 = ( ( x11 AND NOT x1 ) OR ( ( x7 AND ( NOT x13 OR ( x5 AND NOT x10 ) ) ) AND NOT x1 ) ) \\
FANCONI-ANEMIA-AND-CHECKPOINT-RECOVERY & 15 & 0 & 15 & x1: v\_ADD, x2: v\_ATM, x3: v\_ATR, x4: v\_CHKREC, x5: v\_DSB\_, x6: v\_FAHRR, x7: v\_FANCD2I, x8: v\_FAcore, x9: v\_HRR2, x10: v\_ICL, x11: v\_NHEJ, x12: v\_NUC1, x13: v\_NUC2, x14: v\_TLS, x15: v\_p53 & x1 = ( ( ( x12 AND NOT x14 ) OR ( x13 AND NOT x14 ) ) OR ( ( x12 AND x13 ) AND NOT x14 ) )
x2 = ( ( x3 AND NOT ( x8 OR x4 ) ) OR ( x5 AND NOT ( x8 OR x4 ) ) )
x3 = ( ( x10 AND NOT x4 ) OR ( x2 AND NOT x4 ) )
x4 = ( ( ( ( ( x14 AND NOT x5 ) OR ( x9 AND NOT x5 ) ) OR ( x6 AND NOT x5 ) ) OR ( x11 AND NOT x5 ) ) OR NOT ( ( ( ( ( ( ( x10 OR x11 ) OR x6 ) OR x1 ) OR x4 ) OR x5 ) OR x9 ) OR x14 ) )
x5 = ( ( x12 AND NOT ( ( x6 OR x9 ) OR x11 ) ) OR ( x13 AND NOT ( ( x6 OR x9 ) OR x11 ) ) )
x6 = ( ( x7 AND x5 ) AND NOT ( x11 AND x4 ) )
x7 = ( ( x8 AND ( ( x5 AND ( x2 OR x3 ) ) OR ( x2 OR x3 ) ) ) AND NOT x4 )
x8 = ( ( x10 AND ( x2 OR x3 ) ) AND NOT x4 )
x9 = ( ( ( x14 AND ( x13 AND x5 ) ) AND NOT ( ( x11 OR x4 ) OR x6 ) ) OR ( ( x13 AND ( ( x10 AND x11 ) AND x5 ) ) AND NOT ( x4 OR x6 ) ) )
x10 = ( x10 AND NOT x5 )
x11 = ( ( x13 AND x5 ) AND NOT ( ( x9 OR x6 ) OR x4 ) )
x12 = ( x7 AND x10 )
x13 = ( ( ( x10 AND ( x2 OR x3 ) ) AND NOT ( x8 AND x7 ) ) OR ( ( x12 AND ( x10 AND x15 ) ) AND NOT ( x8 AND x7 ) ) )
x14 = ( ( ( x8 AND x1 ) AND NOT x4 ) OR ( x1 AND NOT x4 ) )
x15 = ( ( ( x11 AND NOT x4 ) OR ( x2 AND NOT x4 ) ) OR ( x3 AND NOT x4 ) ) \\
ROOT-STEM-CELL-2010 & 10 & 2 & 8 & x1: v\_ARF, x2: v\_AUXIAA, x3: v\_AUXIN, x4: v\_CLEX, x5: v\_JKD, x6: v\_MGP, x7: v\_PLT, x8: v\_SCR, x9: v\_SHR, x10: v\_WOX5 & x1 = NOT x2
x2 = NOT x3
x4 = ( x9 AND x4 )
x5 = ( x9 AND x8 )
x6 = ( ( x9 AND x8 ) AND NOT x10 )
x7 = x1
x8 = ( x9 AND x8 )
x10 = ( ( ( x1 AND x9 ) AND x8 ) AND NOT x4 ) \\
DROSOPHILA-NOTCH-PATHWAY & 13 & 6 & 7 & x1: v\_CtBP, x2: v\_Da, x3: v\_Delta, x4: v\_E\_Spl\_b1, x5: v\_E\_Spl\_b2, x6: v\_Emc, x7: v\_Gro, x8: v\_H, x9: v\_Mam, x10: v\_Nicd, x11: v\_Notch, x12: v\_Twi\_b1, x13: v\_Twi\_b2 & x4 = ( ( ( ( ( ( ( ( ( NOT x10 OR ( ( ( ( x10 AND NOT x4 ) AND NOT x8 ) AND NOT x7 ) AND NOT x1 ) ) OR ( ( ( ( ( x10 AND NOT x4 ) AND NOT x8 ) AND NOT x7 ) AND x1 ) AND NOT x9 ) ) OR ( ( ( ( x10 AND NOT x4 ) AND NOT x8 ) AND x7 ) AND NOT x9 ) ) OR ( ( ( x10 AND NOT x4 ) AND x8 ) AND NOT x9 ) ) OR ( ( ( ( ( x10 AND x4 ) AND NOT x5 ) AND NOT x8 ) AND NOT x7 ) AND NOT x1 ) ) OR ( ( ( ( ( ( x10 AND x4 ) AND NOT x5 ) AND NOT x8 ) AND NOT x7 ) AND x1 ) AND NOT x9 ) ) OR ( ( ( ( ( x10 AND x4 ) AND NOT x5 ) AND NOT x8 ) AND x7 ) AND NOT x9 ) ) OR ( ( ( ( x10 AND x4 ) AND NOT x5 ) AND x8 ) AND NOT x9 ) ) OR ( ( x10 AND x4 ) AND x5 ) )
x5 = ( ( ( ( ( x10 AND x4 ) AND NOT x8 ) AND NOT x7 ) AND NOT x1 ) AND x9 )
x6 = x10
x10 = x11
x11 = x3
x12 = ( ( ( ( ( ( ( ( ( NOT x6 AND NOT x2 ) AND x12 ) AND x13 ) OR ( NOT x6 AND x2 ) ) OR ( ( ( ( x6 AND NOT x4 ) AND NOT x2 ) AND x12 ) AND x13 ) ) OR ( ( x6 AND NOT x4 ) AND x2 ) ) OR ( ( ( ( ( x6 AND x4 ) AND NOT x5 ) AND NOT x2 ) AND x12 ) AND x13 ) ) OR ( ( ( x6 AND x4 ) AND NOT x5 ) AND x2 ) ) OR ( ( ( ( x6 AND x4 ) AND x5 ) AND x12 ) AND x13 ) )
x13 = ( ( ( NOT x6 AND x2 ) AND x12 ) OR ( ( ( x6 AND NOT x4 ) AND x2 ) AND x12 ) ) \\
FISSION-YEAST-2008 & 10 & 1 & 9 & x1: v\_Cdc25, x2: v\_Cdc2\_Cdc13, x3: v\_Cdc2\_Cdc13\_A, x4: v\_PP, x5: v\_Rum1, x6: v\_SK, x7: v\_Slp1, x8: v\_Start, x9: v\_Ste9, x10: v\_Wee1\_Mik1 & x1 = ( ( ( ( NOT x2 AND x1 ) AND NOT x4 ) OR ( ( x2 AND NOT x1 ) AND NOT x4 ) ) OR ( x2 AND x1 ) )
x2 = ( ( NOT x9 AND NOT x5 ) AND NOT x7 )
x3 = ( ( ( ( NOT x9 AND NOT x5 ) AND NOT x7 ) AND NOT x10 ) AND x1 )
x4 = x7
x5 = ( ( ( ( ( ( ( ( NOT x6 AND NOT x2 ) AND NOT x5 ) AND NOT x3 ) AND x4 ) OR ( ( ( NOT x6 AND NOT x2 ) AND x5 ) AND NOT x3 ) ) OR ( ( ( ( NOT x6 AND NOT x2 ) AND x5 ) AND x3 ) AND x4 ) ) OR ( ( ( ( NOT x6 AND x2 ) AND x5 ) AND NOT x3 ) AND x4 ) ) OR ( ( ( ( x6 AND NOT x2 ) AND x5 ) AND NOT x3 ) AND x4 ) )
x6 = x8
x7 = x3
x9 = ( ( ( ( ( ( ( ( NOT x6 AND NOT x2 ) AND NOT x9 ) AND NOT x3 ) AND x4 ) OR ( ( ( NOT x6 AND NOT x2 ) AND x9 ) AND NOT x3 ) ) OR ( ( ( ( NOT x6 AND NOT x2 ) AND x9 ) AND x3 ) AND x4 ) ) OR ( ( ( ( NOT x6 AND x2 ) AND x9 ) AND NOT x3 ) AND x4 ) ) OR ( ( ( ( x6 AND NOT x2 ) AND x9 ) AND NOT x3 ) AND x4 ) )
x10 = ( ( ( ( NOT x2 AND NOT x10 ) AND x4 ) OR ( NOT x2 AND x10 ) ) OR ( ( x2 AND x10 ) AND x4 ) ) \\
TRP-BIOSYNTHESIS & 6 & 1 & 5 & x1: v\_TrpE, x2: v\_TrpR, x3: v\_Trp\_b1, x4: v\_Trp\_b2, x5: v\_Trpext\_b1, x6: v\_Trpext\_b2 & x1 = ( NOT x3 AND NOT x2 )
x2 = ( x3 AND x4 )
x3 = ( ( ( ( ( NOT x5 AND NOT x3 ) AND x1 ) OR ( ( ( NOT x5 AND x3 ) AND NOT x4 ) AND x1 ) ) OR ( ( NOT x5 AND x3 ) AND x4 ) ) OR x5 )
x4 = ( ( x5 AND x6 ) AND x3 )
x6 = ( x5 AND x6 ) \\
MULTILEVEL-CELL-CYCLE & 13 & 1 & 12 & x1: v\_Cdc20, x2: v\_Cdh1, x3: v\_CycA, x4: v\_CycB, x5: v\_CycD, x6: v\_CycE, x7: v\_E2F, x8: v\_Rb\_b1, x9: v\_Rb\_b2, x10: v\_Skp2, x11: v\_UbcH10, x12: v\_p27\_b1, x13: v\_p27\_b2 & x1 = x4
x2 = ( ( ( ( NOT x3 AND NOT x4 ) OR ( ( NOT x3 AND x4 ) AND x12 ) ) OR ( ( ( x3 AND x12 ) AND NOT x13 ) AND NOT x10 ) ) OR ( ( x3 AND x12 ) AND x13 ) )
x3 = ( ( ( ( ( ( ( ( ( ( ( ( NOT x8 AND NOT x7 ) AND x3 ) AND NOT x1 ) AND NOT x2 ) OR ( ( ( ( ( NOT x8 AND NOT x7 ) AND x3 ) AND NOT x1 ) AND x2 ) AND NOT x11 ) ) OR ( ( ( ( NOT x8 AND NOT x7 ) AND x3 ) AND x1 ) AND NOT x11 ) ) OR ( ( ( NOT x8 AND x7 ) AND NOT x1 ) AND NOT x2 ) ) OR ( ( ( ( NOT x8 AND x7 ) AND NOT x1 ) AND x2 ) AND NOT x11 ) ) OR ( ( ( NOT x8 AND x7 ) AND x1 ) AND NOT x11 ) ) OR ( ( ( x8 AND x3 ) AND NOT x1 ) AND NOT x2 ) ) OR ( ( ( ( x8 AND x3 ) AND NOT x1 ) AND x2 ) AND NOT x11 ) ) OR ( ( ( x8 AND x3 ) AND x1 ) AND NOT x11 ) )
x4 = ( ( NOT x1 AND NOT x2 ) OR ( ( x1 AND NOT x2 ) AND NOT x11 ) )
x6 = ( ( NOT x8 AND x7 ) OR ( ( x8 AND NOT x9 ) AND x7 ) )
x7 = ( ( ( ( ( ( ( ( ( ( ( ( ( NOT x8 AND NOT x3 ) AND NOT x4 ) OR ( ( ( NOT x8 AND NOT x3 ) AND x4 ) AND NOT x1 ) ) OR ( ( ( ( ( NOT x8 AND x3 ) AND NOT x4 ) AND x12 ) AND NOT x13 ) AND NOT x10 ) ) OR ( ( ( ( NOT x8 AND x3 ) AND NOT x4 ) AND x12 ) AND x13 ) ) OR ( ( ( ( ( ( NOT x8 AND x3 ) AND x4 ) AND x12 ) AND NOT x13 ) AND NOT x1 ) AND NOT x10 ) ) OR ( ( ( ( ( NOT x8 AND x3 ) AND x4 ) AND x12 ) AND x13 ) AND NOT x1 ) ) OR ( ( ( x8 AND NOT x9 ) AND NOT x3 ) AND NOT x4 ) ) OR ( ( ( ( x8 AND NOT x9 ) AND NOT x3 ) AND x4 ) AND NOT x1 ) ) OR ( ( ( ( ( ( x8 AND NOT x9 ) AND x3 ) AND NOT x4 ) AND x12 ) AND NOT x13 ) AND NOT x10 ) ) OR ( ( ( ( ( x8 AND NOT x9 ) AND x3 ) AND NOT x4 ) AND x12 ) AND x13 ) ) OR ( ( ( ( ( ( ( x8 AND NOT x9 ) AND x3 ) AND x4 ) AND x12 ) AND NOT x13 ) AND NOT x1 ) AND NOT x10 ) ) OR ( ( ( ( ( ( x8 AND NOT x9 ) AND x3 ) AND x4 ) AND x12 ) AND x13 ) AND NOT x1 ) )
x8 = ( ( ( ( ( ( ( ( ( ( ( NOT x8 AND NOT x6 ) AND NOT x3 ) AND NOT x4 ) OR ( ( ( ( NOT x8 AND NOT x6 ) AND NOT x3 ) AND x4 ) AND x12 ) ) OR ( ( ( NOT x8 AND NOT x6 ) AND x3 ) AND x12 ) ) OR ( ( NOT x8 AND x6 ) AND x12 ) ) OR ( ( ( ( x8 AND NOT x9 ) AND NOT x6 ) AND NOT x3 ) AND NOT x4 ) ) OR ( ( ( ( ( x8 AND NOT x9 ) AND NOT x6 ) AND NOT x3 ) AND x4 ) AND x12 ) ) OR ( ( ( ( x8 AND NOT x9 ) AND NOT x6 ) AND x3 ) AND x12 ) ) OR ( ( ( x8 AND NOT x9 ) AND x6 ) AND x12 ) ) OR ( x8 AND x9 ) )
x9 = ( ( ( ( ( ( ( ( NOT x5 AND x8 ) AND NOT x6 ) AND NOT x3 ) AND NOT x4 ) OR ( ( ( ( ( NOT x5 AND x8 ) AND NOT x6 ) AND NOT x3 ) AND x4 ) AND x12 ) ) OR ( ( ( ( NOT x5 AND x8 ) AND NOT x6 ) AND x3 ) AND x12 ) ) OR ( ( ( ( NOT x5 AND x8 ) AND x6 ) AND NOT x3 ) AND x12 ) ) OR ( ( ( ( ( NOT x5 AND x8 ) AND x6 ) AND x3 ) AND NOT x4 ) AND x12 ) )
x10 = ( ( NOT x8 OR ( x8 AND NOT x9 ) ) OR ( ( x8 AND x9 ) AND NOT x2 ) )
x11 = ( ( ( ( ( ( ( ( ( NOT x3 AND NOT x4 ) AND NOT x1 ) AND NOT x2 ) OR ( ( ( NOT x3 AND NOT x4 ) AND x1 ) AND NOT x2 ) ) OR ( ( ( ( NOT x3 AND NOT x4 ) AND x1 ) AND x2 ) AND x11 ) ) OR ( ( NOT x3 AND x4 ) AND NOT x2 ) ) OR ( ( ( NOT x3 AND x4 ) AND x2 ) AND x11 ) ) OR ( x3 AND NOT x2 ) ) OR ( ( x3 AND x2 ) AND x11 ) )
x12 = ( ( ( ( ( ( ( ( ( ( ( ( ( NOT x6 AND NOT x3 ) AND NOT x4 ) OR ( ( ( ( NOT x6 AND NOT x3 ) AND x4 ) AND NOT x12 ) AND NOT x10 ) ) OR ( ( ( ( ( NOT x6 AND NOT x3 ) AND x4 ) AND x12 ) AND NOT x13 ) AND NOT x10 ) ) OR ( ( ( ( NOT x6 AND NOT x3 ) AND x4 ) AND x12 ) AND x13 ) ) OR ( ( ( ( NOT x6 AND x3 ) AND NOT x4 ) AND NOT x12 ) AND NOT x10 ) ) OR ( ( ( NOT x6 AND x3 ) AND NOT x4 ) AND x12 ) ) OR ( ( ( ( NOT x6 AND x3 ) AND x4 ) AND NOT x12 ) AND NOT x10 ) ) OR ( ( ( ( ( NOT x6 AND x3 ) AND x4 ) AND x12 ) AND NOT x13 ) AND NOT x10 ) ) OR ( ( ( ( NOT x6 AND x3 ) AND x4 ) AND x12 ) AND x13 ) ) OR ( ( x6 AND NOT x12 ) AND NOT x10 ) ) OR ( ( ( x6 AND x12 ) AND NOT x13 ) AND NOT x10 ) ) OR ( ( x6 AND x12 ) AND x13 ) )
x13 = ( ( ( ( ( ( ( ( NOT x5 AND NOT x6 ) AND NOT x4 ) AND x12 ) OR ( ( ( ( NOT x5 AND NOT x6 ) AND x4 ) AND x12 ) AND NOT x10 ) ) OR ( ( ( ( ( ( NOT x5 AND x6 ) AND NOT x3 ) AND NOT x4 ) AND x12 ) AND NOT x13 ) AND NOT x10 ) ) OR ( ( ( ( ( NOT x5 AND x6 ) AND NOT x3 ) AND NOT x4 ) AND x12 ) AND x13 ) ) OR ( ( ( ( ( NOT x5 AND x6 ) AND NOT x3 ) AND x4 ) AND x12 ) AND NOT x10 ) ) OR ( ( ( ( NOT x5 AND x6 ) AND x3 ) AND x12 ) AND NOT x10 ) ) \\
ACUTE-RESPONSES-DURING-HYPERINSULINEMIA & 19 & 9 & 10 & x1: v\_FOXP3, x2: v\_GATA3, x3: v\_IFNG, x4: v\_IFNGe, x5: v\_IL10, x6: v\_IL10e, x7: v\_IL12e, x8: v\_IL2, x9: v\_IL21, x10: v\_IL21e, x11: v\_IL27e, x12: v\_IL2e, x13: v\_IL4, x14: v\_IL4e, x15: v\_INSULIN, x16: v\_RORGT, x17: v\_TBET, x18: v\_TGFB, x19: v\_TGFBe & x1 = ( ( x8 AND ( x18 OR x1 ) ) AND NOT ( x9 OR x16 ) )
x2 = ( ( ( x8 AND x13 ) OR x2 ) AND NOT ( ( ( x17 OR x18 ) OR x9 ) OR x3 ) )
x3 = ( ( x4 OR ( ( x3 OR x17 ) AND NOT ( x2 OR x18 ) ) ) AND NOT ( ( x9 OR x13 ) OR x5 ) )
x5 = ( x6 OR ( ( x5 AND ( ( ( ( x3 OR x9 ) OR x18 ) OR x2 ) OR x11 ) ) AND NOT x15 ) )
x8 = ( ( x12 OR ( x8 AND NOT x1 ) ) AND NOT ( ( x3 OR x9 ) OR ( x5 AND NOT x1 ) ) )
x9 = ( ( ( x10 OR x9 ) OR x16 ) AND NOT ( ( ( x3 OR x13 ) OR x5 ) OR x8 ) )
x13 = ( ( x14 OR ( ( x2 AND ( x8 OR x13 ) ) AND NOT x17 ) ) AND NOT ( x3 OR x9 ) )
x16 = ( ( x9 AND x18 ) AND NOT ( ( x17 OR x1 ) OR x2 ) )
x17 = ( ( ( x3 OR ( x7 AND NOT ( ( x9 OR x13 ) OR x5 ) ) ) OR x17 ) AND NOT ( ( x13 OR x2 ) OR x9 ) )
x18 = ( x19 OR ( ( x18 OR x1 ) AND NOT x9 ) ) \\
VEGF-PATHWAY-OF-DROSOPHILA & 18 & 8 & 10 & x1: v\_Aop, x2: v\_CNK, x3: v\_Drk, x4: v\_Dsor1, x5: v\_Ksr, x6: v\_Pnt, x7: v\_Pvf1, x8: v\_Pvf2, x9: v\_Pvf3, x10: v\_Pvr, x11: v\_Raf, x12: v\_Ras, x13: v\_Rl, x14: v\_Sos, x15: v\_Src42, x16: v\_Sty, x17: v\_Targets, x18: v\_msk & x1 = NOT x13
x3 = x10
x4 = x11
x6 = x13
x10 = ( ( x8 OR x7 ) OR x9 )
x11 = ( x12 AND ( ( x2 AND x5 ) AND x15 ) )
x12 = ( x14 AND NOT x16 )
x13 = ( x4 AND x18 )
x14 = x3
x17 = ( x6 AND NOT x1 ) \\
ERBB-REGULATED-G1-S-TRANSITION & 20 & 1 & 19 & x1: v\_AKT1, x2: v\_CDK2, x3: v\_CDK4, x4: v\_CDK6, x5: v\_CyclinD1, x6: v\_CyclinE1, x7: v\_EGF, x8: v\_ERBB1, x9: v\_ERBB1\_2, x10: v\_ERBB1\_3, x11: v\_ERBB2, x12: v\_ERBB2\_3, x13: v\_ERBB3, x14: v\_ERalpha, x15: v\_IGF1R, x16: v\_MEK1, x17: v\_MYC, x18: v\_p21, x19: v\_p27, x20: v\_pRB1 & x1 = ( ( ( ( ( ( ( ( NOT x15 AND NOT x8 ) AND NOT x12 ) AND NOT x9 ) AND x10 ) OR ( ( ( NOT x15 AND NOT x8 ) AND NOT x12 ) AND x9 ) ) OR ( ( NOT x15 AND NOT x8 ) AND x12 ) ) OR ( NOT x15 AND x8 ) ) OR x15 )
x2 = ( ( NOT x18 AND NOT x19 ) AND x6 )
x3 = ( ( NOT x18 AND x5 ) AND NOT x19 )
x4 = x5
x5 = ( ( ( ( NOT x16 AND x14 ) AND x1 ) AND x17 ) OR ( ( x16 AND x14 ) AND x17 ) )
x6 = x17
x8 = x7
x9 = ( x8 AND x11 )
x10 = ( x8 AND x13 )
x11 = x7
x12 = ( x11 AND x13 )
x13 = x7
x14 = ( ( NOT x16 AND x1 ) OR x16 )
x15 = ( ( ( NOT x14 AND x1 ) AND NOT x12 ) OR ( x14 AND NOT x12 ) )
x16 = ( ( ( ( ( ( ( ( NOT x15 AND NOT x8 ) AND NOT x12 ) AND NOT x9 ) AND x10 ) OR ( ( ( NOT x15 AND NOT x8 ) AND NOT x12 ) AND x9 ) ) OR ( ( NOT x15 AND NOT x8 ) AND x12 ) ) OR ( NOT x15 AND x8 ) ) OR x15 )
x17 = ( ( ( ( NOT x16 AND NOT x14 ) AND x1 ) OR ( NOT x16 AND x14 ) ) OR x16 )
x18 = ( ( NOT x3 AND NOT x1 ) AND NOT x17 )
x19 = ( ( ( NOT x3 AND NOT x2 ) AND NOT x1 ) AND NOT x17 )
x20 = ( x3 AND x4 ) \\
\bottomrule

\end{longtable}
% \end{adjustbox}



% \end{tabular}
% }

% \caption{Boolean‑network models used in this study.}
% \label{tab:bn-summary}
% \end{longtable}


\begin{figure}[H]
    \centering
    \includegraphics[width=\linewidth]{figures/state_graphs_components/ASYMMETRIC-CELL-DIVISION-A_state_graph_components.png}
    \caption{Asymmetric Cell Division A}
\end{figure}

\begin{figure}[H]
    \centering
    \includegraphics[width=\linewidth]{figures/state_graphs_components/CORTICAL-AREA-DEVELOPMENT_state_graph_components.png}
    \caption{Cortical Area Development}
\end{figure}

\begin{figure}[H]
    \centering
    \includegraphics[width=\linewidth]{figures/state_graphs_components/DROSOPHILA-GAP-A_state_graph_components.png}
    \caption{Drosophila GAP A}
\end{figure}

\begin{figure}[H]
    \centering
    \includegraphics[width=\linewidth]{figures/state_graphs_components/DROSOPHILA-GAP-B_state_graph_components.png}
    \caption{Drosophila GAP B}
\end{figure}

\begin{figure}[H]
    \centering
    \includegraphics[width=\linewidth]{figures/state_graphs_components/DROSOPHILA-GAP-C_state_graph_components.png}
    \caption{Drosophila GAP C}
\end{figure}

\begin{figure}[H]
    \centering
    \includegraphics[width=\linewidth]{figures/state_graphs_components/DROSOPHILA-GAP-D_state_graph_components.png}
    \caption{Drosophila GAP D}
\end{figure}

\begin{figure}[H]
    \centering
    \includegraphics[width=\linewidth]{figures/state_graphs_components/EGGSHELL-PATTERNING-PHENOMOENOLOGICAL_state_graph_components.png}
    \caption{Eggshell Patterning Phenomenological}
\end{figure}

\begin{figure}[H]
    \centering
    \includegraphics[width=\linewidth]{figures/state_graphs_components/LAMBDA-PHAGE-LYSOGENY_state_graph_components.png}
    \caption{Lambda Phage Lysogeny}
\end{figure}

% \begin{figure}[H]
%     \centering
%     \includegraphics[width=\linewidth]{figures/state_graphs_components/MIR-9-NEUROGENESIS_state_graph_components.png}
%     \caption{miR-9 Neurogenesis}
% \end{figure}

\begin{figure}[H]
    \centering
    \includegraphics[width=\linewidth]{figures/state_graphs_components/P53-MDM2-NETWORK_state_graph_components.png}
    \caption{P53-MDM2 Network}
\end{figure}

\begin{figure}[H]
    \centering
    \includegraphics[width=\linewidth]{figures/state_graphs_components/TRP-BIOSYNTHESIS_state_graph_components.png}
    \caption{TRP Biosynthesis}
\end{figure}


\clearpage
\section{Structured Causal Graph}
\label{appendix: causal_graph}


\subsection{Noisy synthetic data}

\begin{figure}[H]
    \centering
    \includegraphics[width=0.8\linewidth]{time_series_plots/plot_lag_2_noise_0_01.png}
    \caption{Maximum Lagging = 2: Time series}
\end{figure}


\begin{figure}[H]
    \centering
    \includegraphics[width=0.8\linewidth]{time_series_plots/Max Lag2.png}
    \caption{Maximum Lagging = 2: Causal Graph}
\end{figure}

\begin{figure}[H]
    \centering
    \includegraphics[width=0.8\linewidth]{time_series_plots/plot_lag_3_noise_0_01.png}
    \caption{Maximum Lagging = 3: Time series}
\end{figure}


\begin{figure}[H]
    \centering
    \includegraphics[width=0.8\linewidth]{time_series_plots/Max Lag3.png}
    \caption{Maximum Lagging = 3: Causal graph}
\end{figure}



\begin{figure}[H]
    \centering
    \includegraphics[width=0.8\linewidth]{time_series_plots/plot_lag_4_noise_0_01.png}
    \caption{Maximum Lagging = 4: Time series}
\end{figure}

\begin{figure}[H]
    \centering
    \includegraphics[width=0.8\linewidth]{time_series_plots/Max Lag4.png}
    \caption{Maximum Lagging = 4: Causal graph}
\end{figure}


\begin{figure}[H]
    \centering
    \includegraphics[width=0.8\linewidth]{time_series_plots/plot_lag_5_noise_0_01.png}
    \caption{Maximum Lagging = 5: Time series}
\end{figure}

\begin{figure}[H]
    \centering
    \includegraphics[width=0.8\linewidth]{time_series_plots/Max Lag 5.png}
    \caption{Maximum Lagging = 5: Causal graph}
\end{figure}



\begin{figure}[H]
    \centering
    \includegraphics[width=0.8\linewidth]{time_series_plots/plot_lag_6_noise_0_01.png}
    \caption{Maximum Lagging = 6: Time series}
\end{figure}

\begin{figure}[H]
    \centering
    \includegraphics[width=0.8\linewidth]{time_series_plots/Max Lag 6.png}
    \caption{Maximum Lagging = 6: Causal graph}
\end{figure}


\subsection{Selected Cases from Coupled Differential equations and boolean networks}

...

\end{appendices}
